# Supplementary material for: Geometric Median (GM) Matching for Robust Data Pruning
Source: arXiv:2406.17188 source file (2025-01-17)
Supplement: Supplementary file 1 [file add_exp.tex]

\clearpage
\subsection{Toy Experiments}
We simulate a Gaussian Mixture Model (GMM) with clean and adversarial components to evaluate robust moment estimation in noisy datasets. The clean data, is drawn from a Gaussian distribution with mean $[0, 0]$ and covariance $\begin{bmatrix} 1 & 0.5 \\ 0.5 & 1 \end{bmatrix}$, while the adversarial data, is drawn from a Gaussian with mean $[-5, 5]$ and the same covariance. We generate 1000 samples, forming a corrupted dataset by combining the clean and adversarial data. 

\begin{itemize}
    \item In~\cref{fig:toy-mean-estimation}, we compare the mean of the corrupted dataset (noisy moment) with a robustly estimated mean using the geometric median to mitigate adversarial influence. 
    
    \item Additionally, in~\cref{fig:toy-corr=0}-\ref{fig:toy-corr=45}, we  compare different geometric pruning strategies in the toy setting. 
\end{itemize}

\begin{figure*} 
\centering
\subfloat[$\psi = 0$]{
\includegraphics[width=0.32\textwidth]{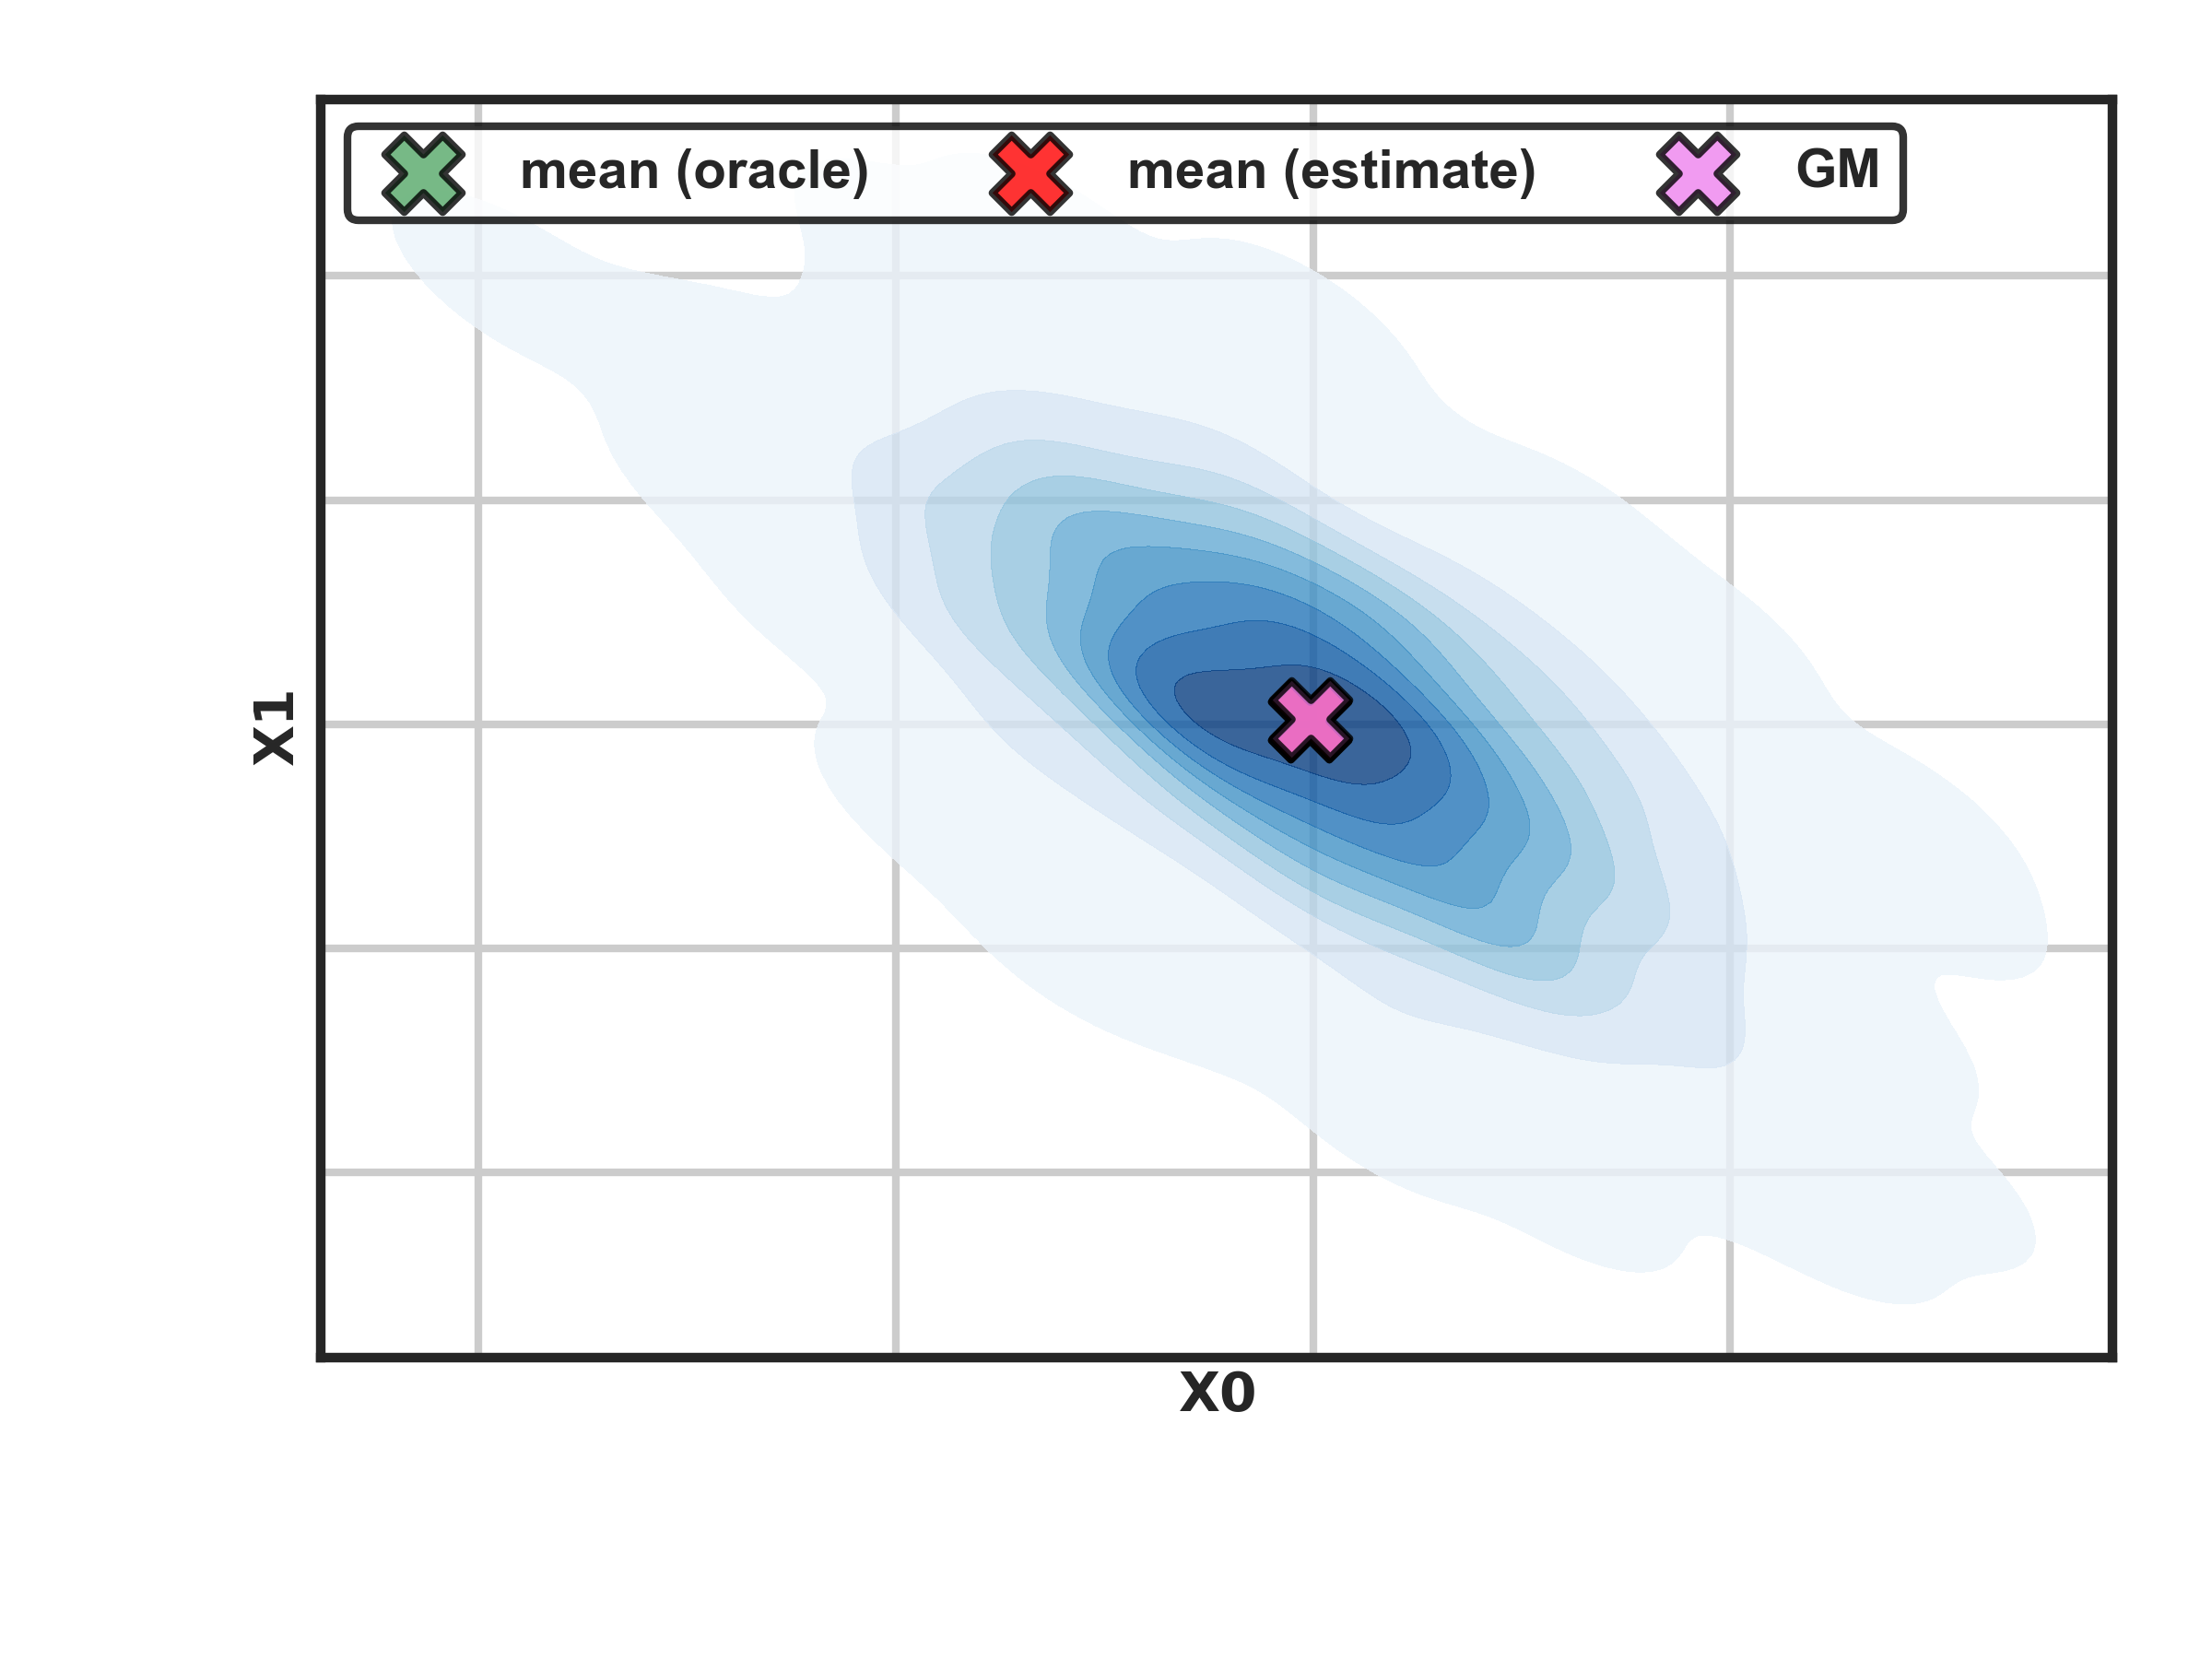}}
\subfloat[$\psi = 0.2$]
{\includegraphics[width=0.32\textwidth]{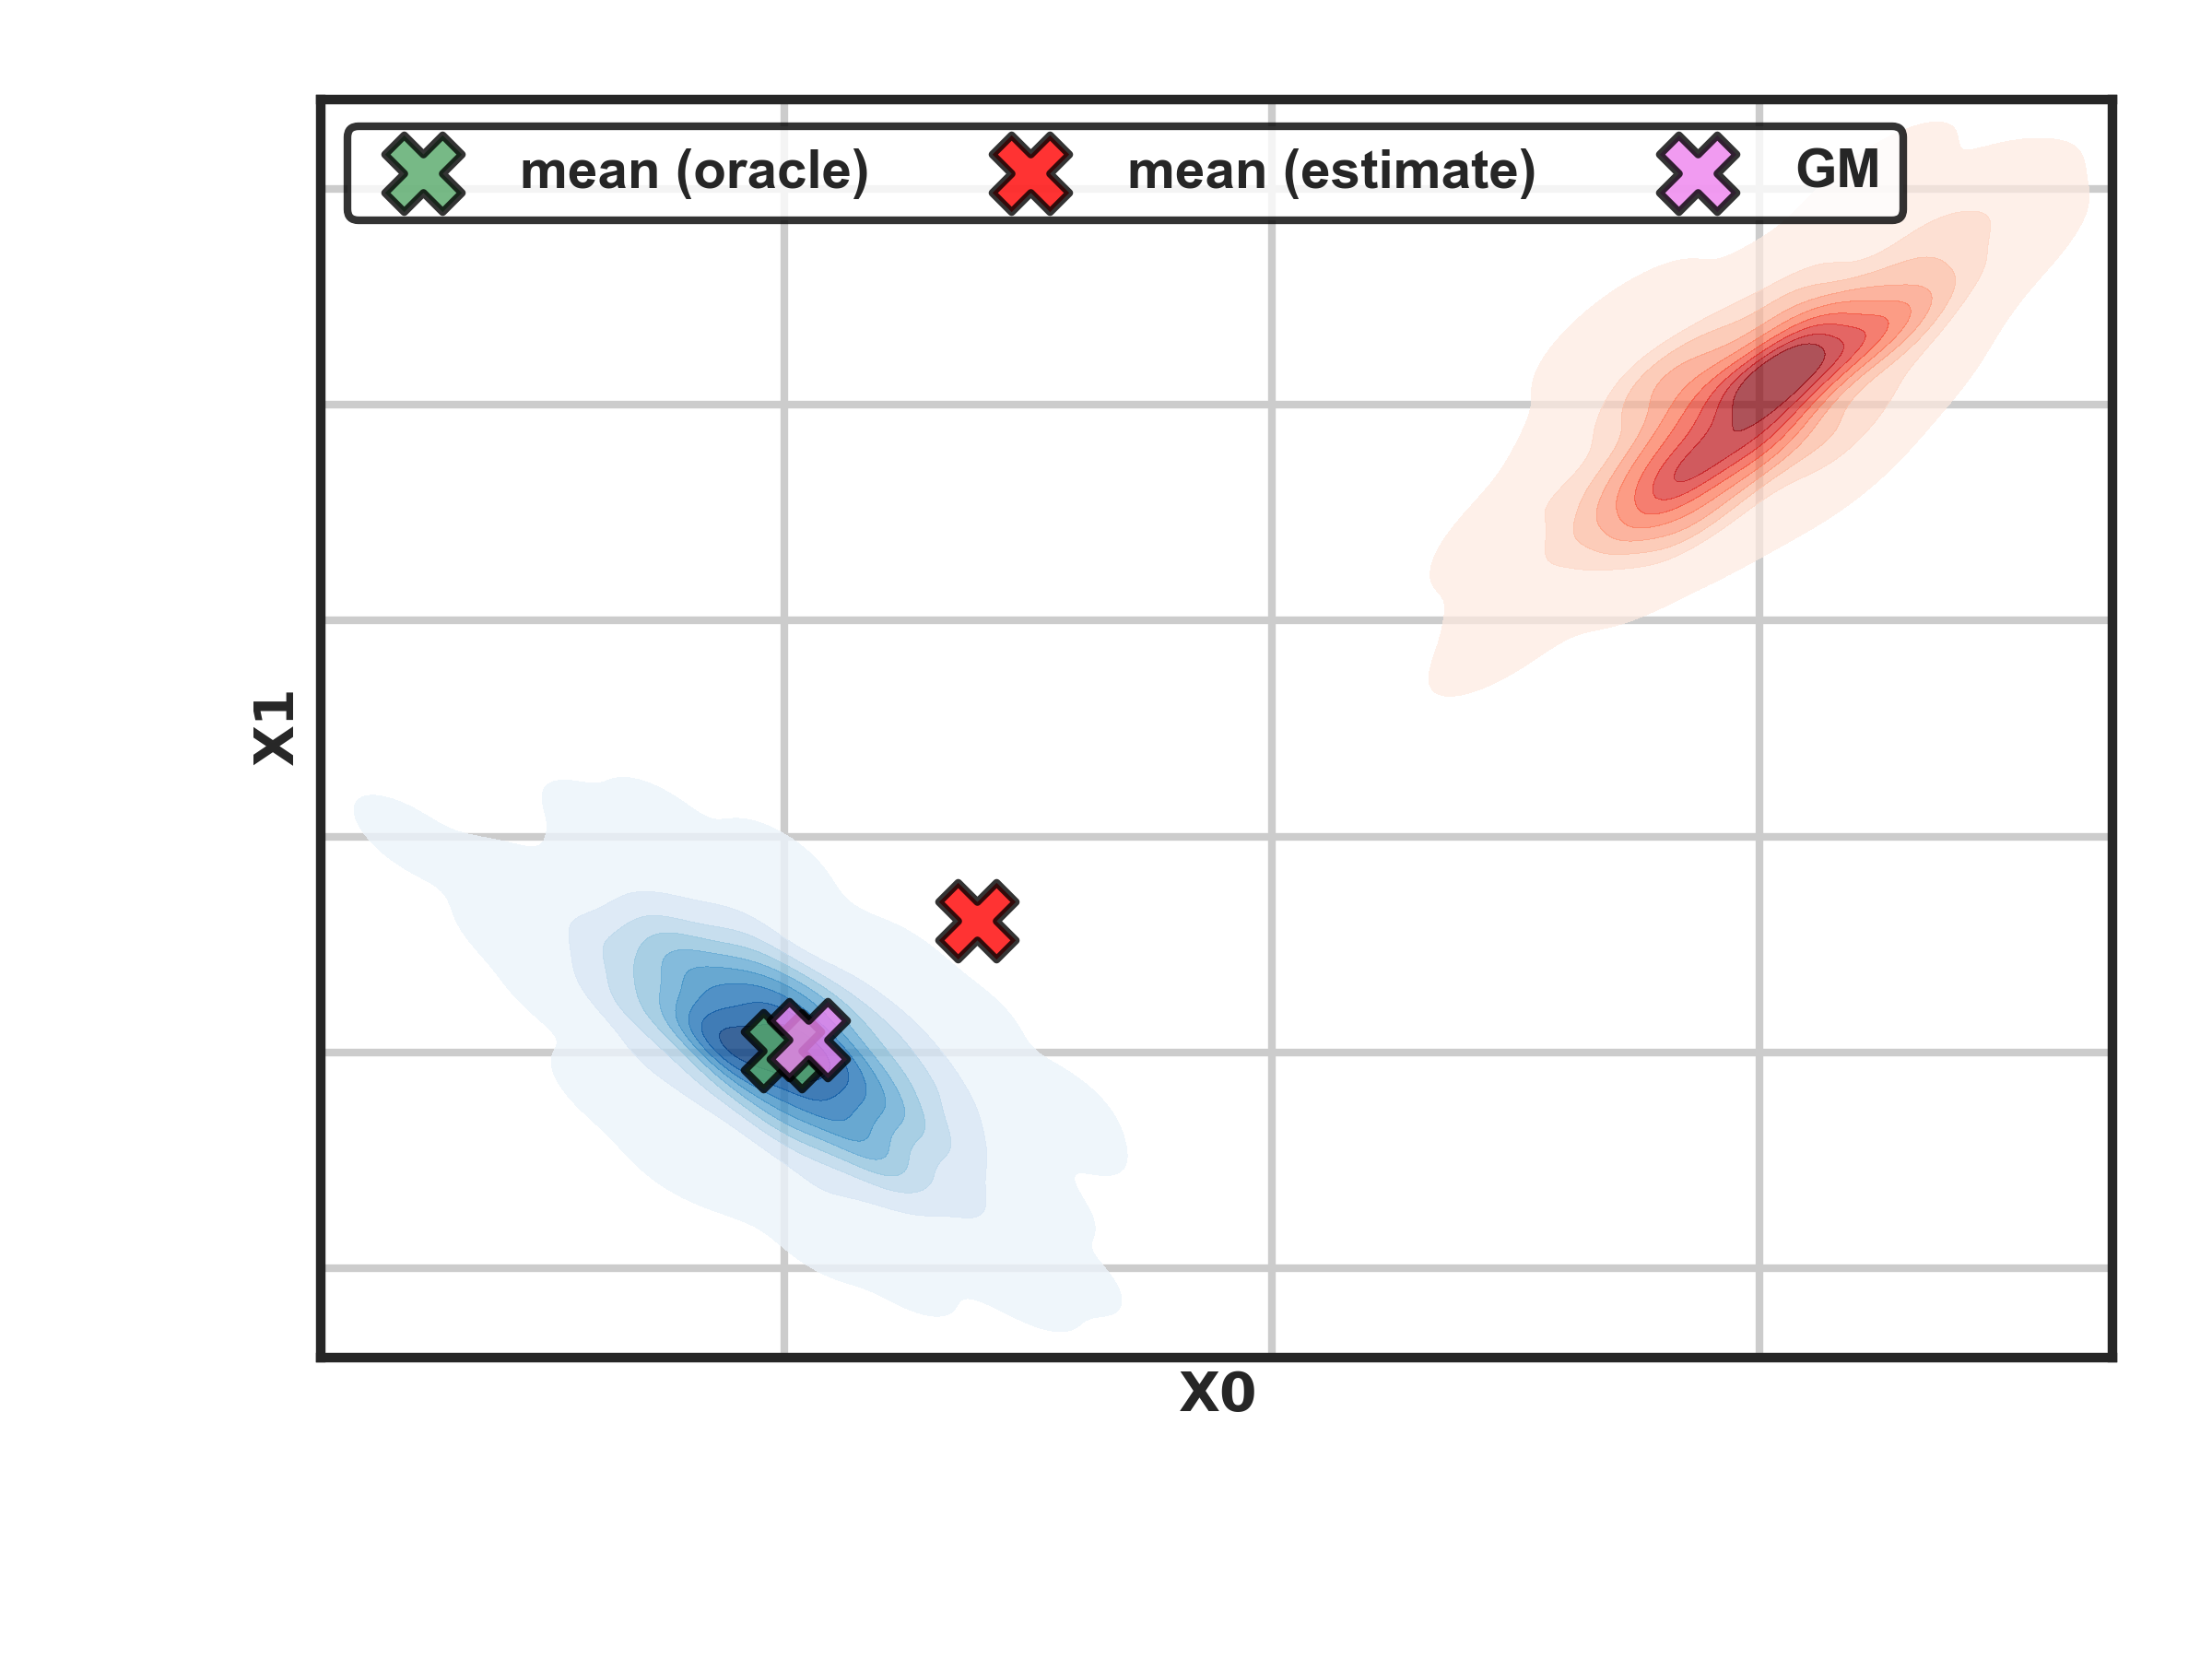}}
\subfloat[$\psi = 0.45$]
{\includegraphics[width=0.32\textwidth]{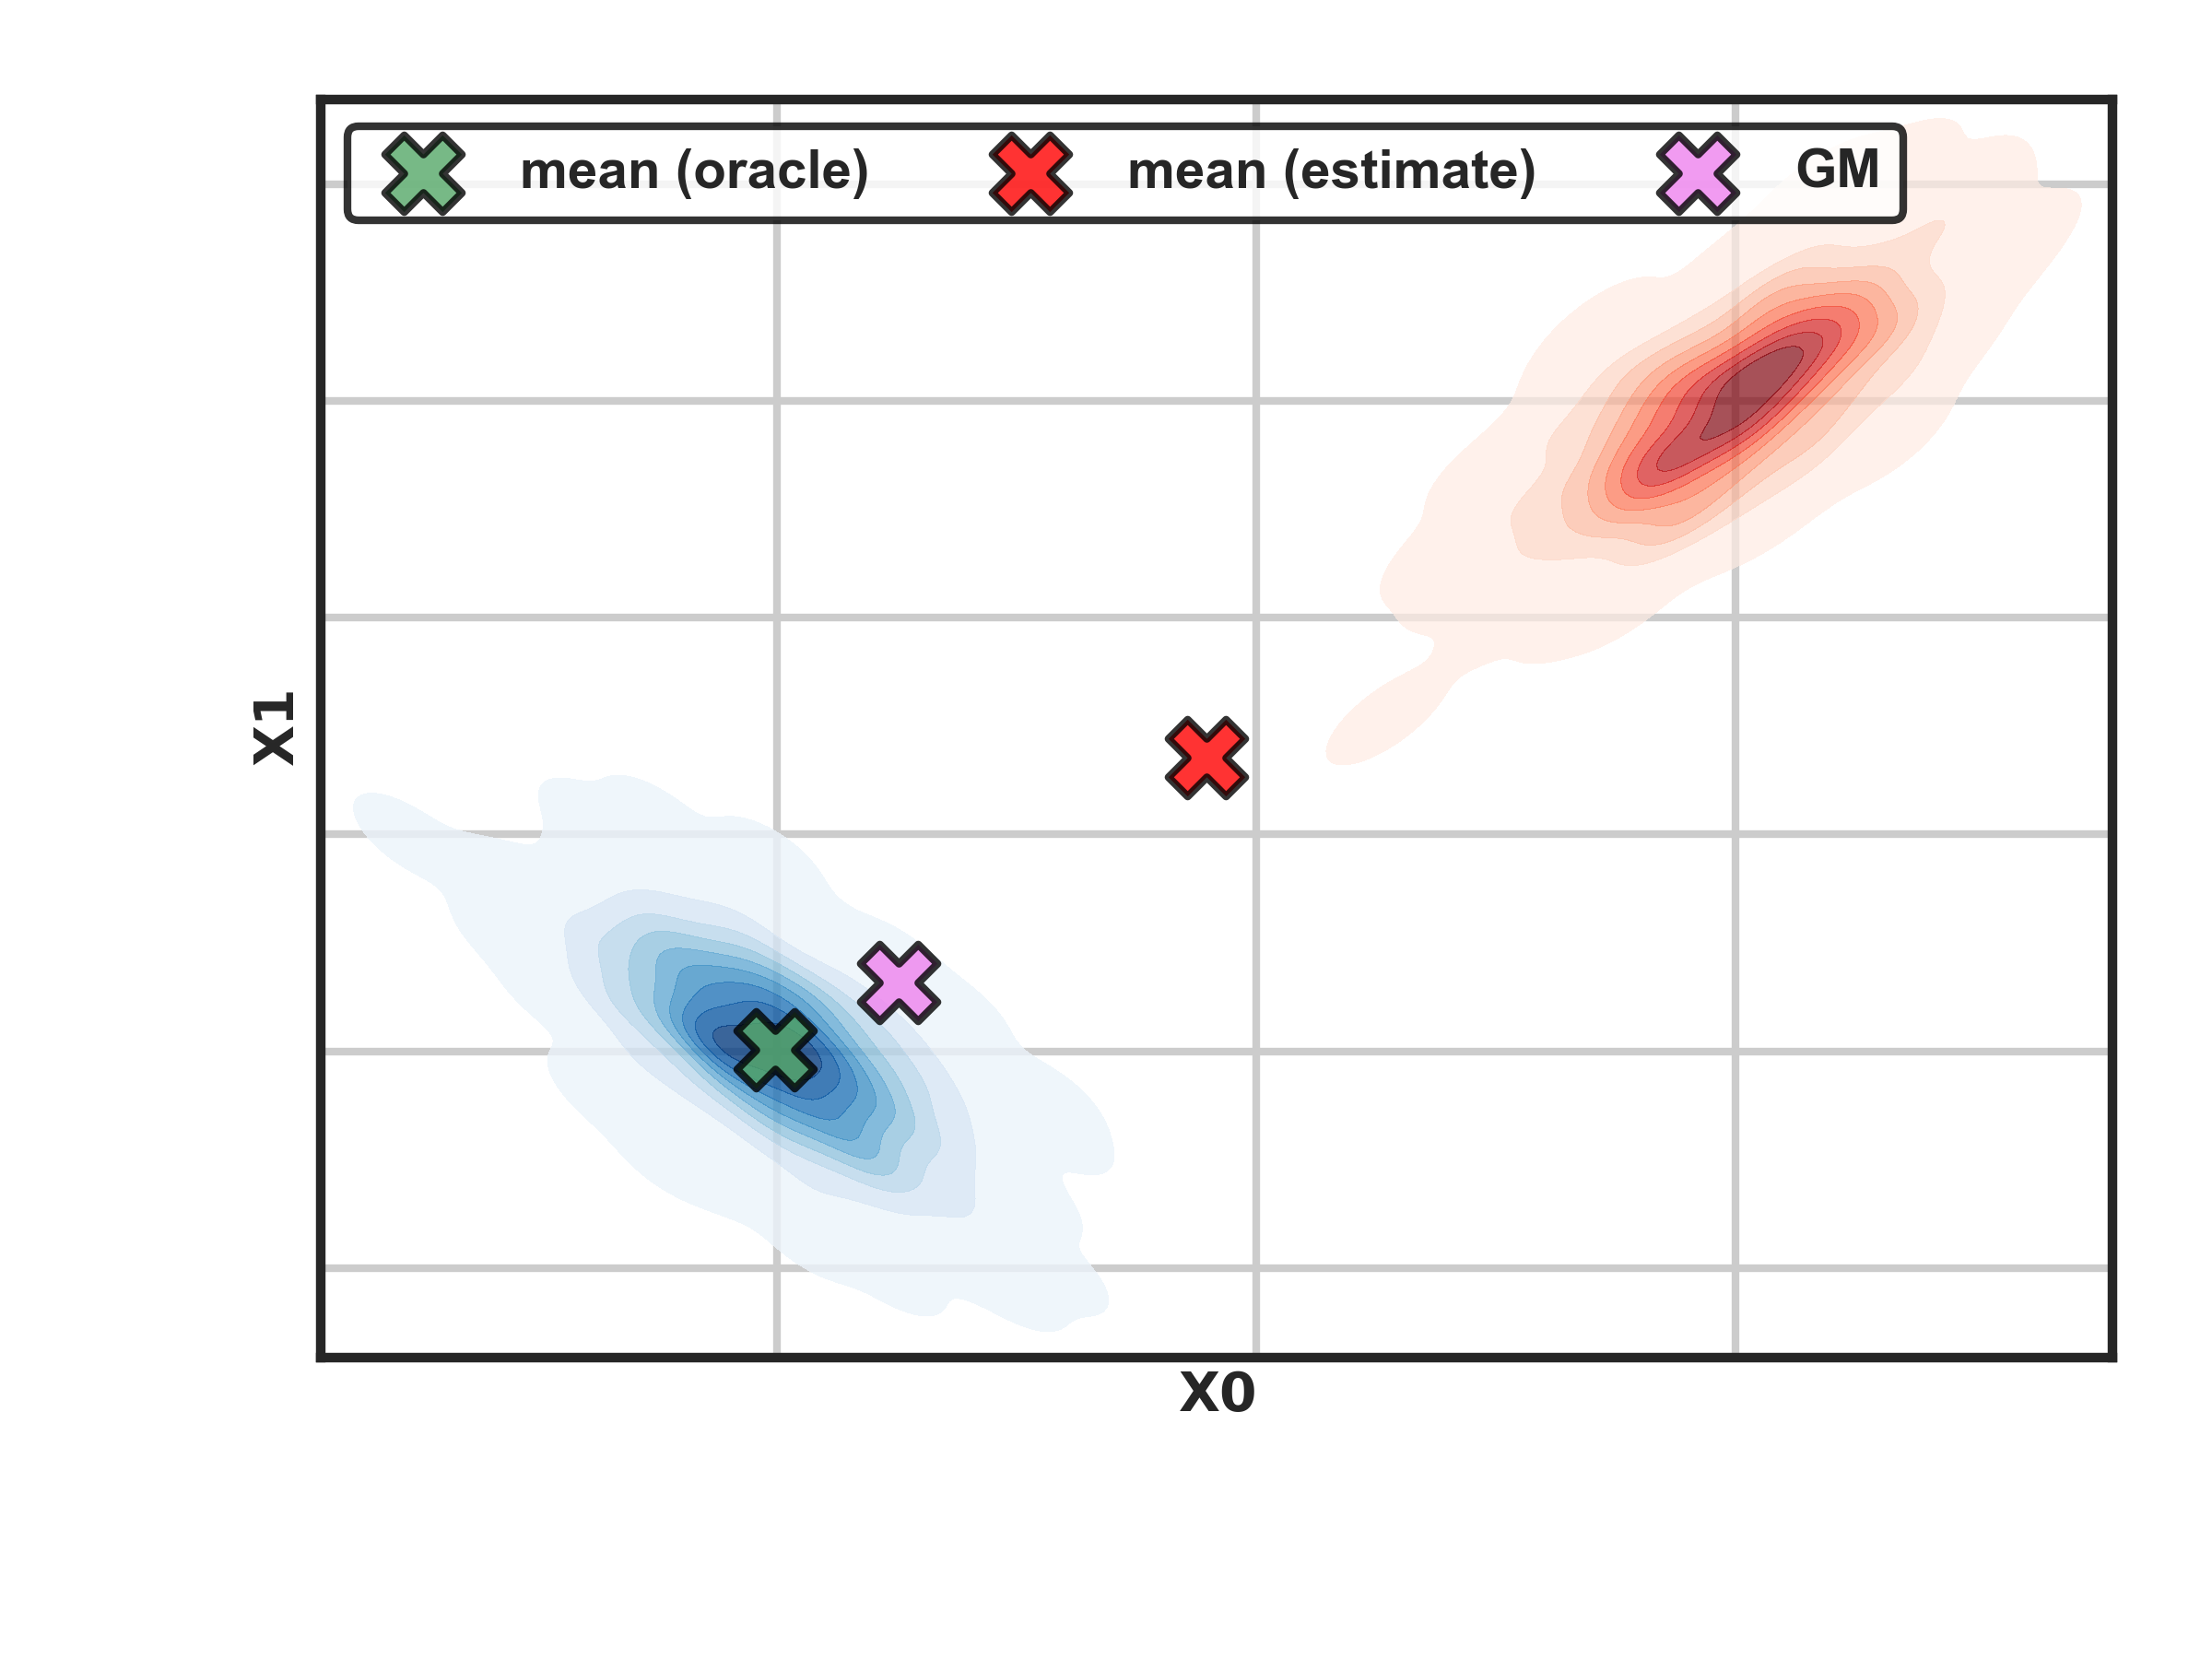}}

\caption{\footnotesize {\bf \textsc{Robust Mean Estimation}}: As we progressively increase $0 \leq \psi < 1/2$ (fraction of corrupt samples in the data); while the empirical mean drifts away,  $\gm$ remains close to the uncorrupted mean.}
\label{fig:toy-mean-estimation}
\end{figure*}

\begin{figure*} 
\centering
\subfloat[\textsc{Uniform}]
{\includegraphics[width=0.32\textwidth]{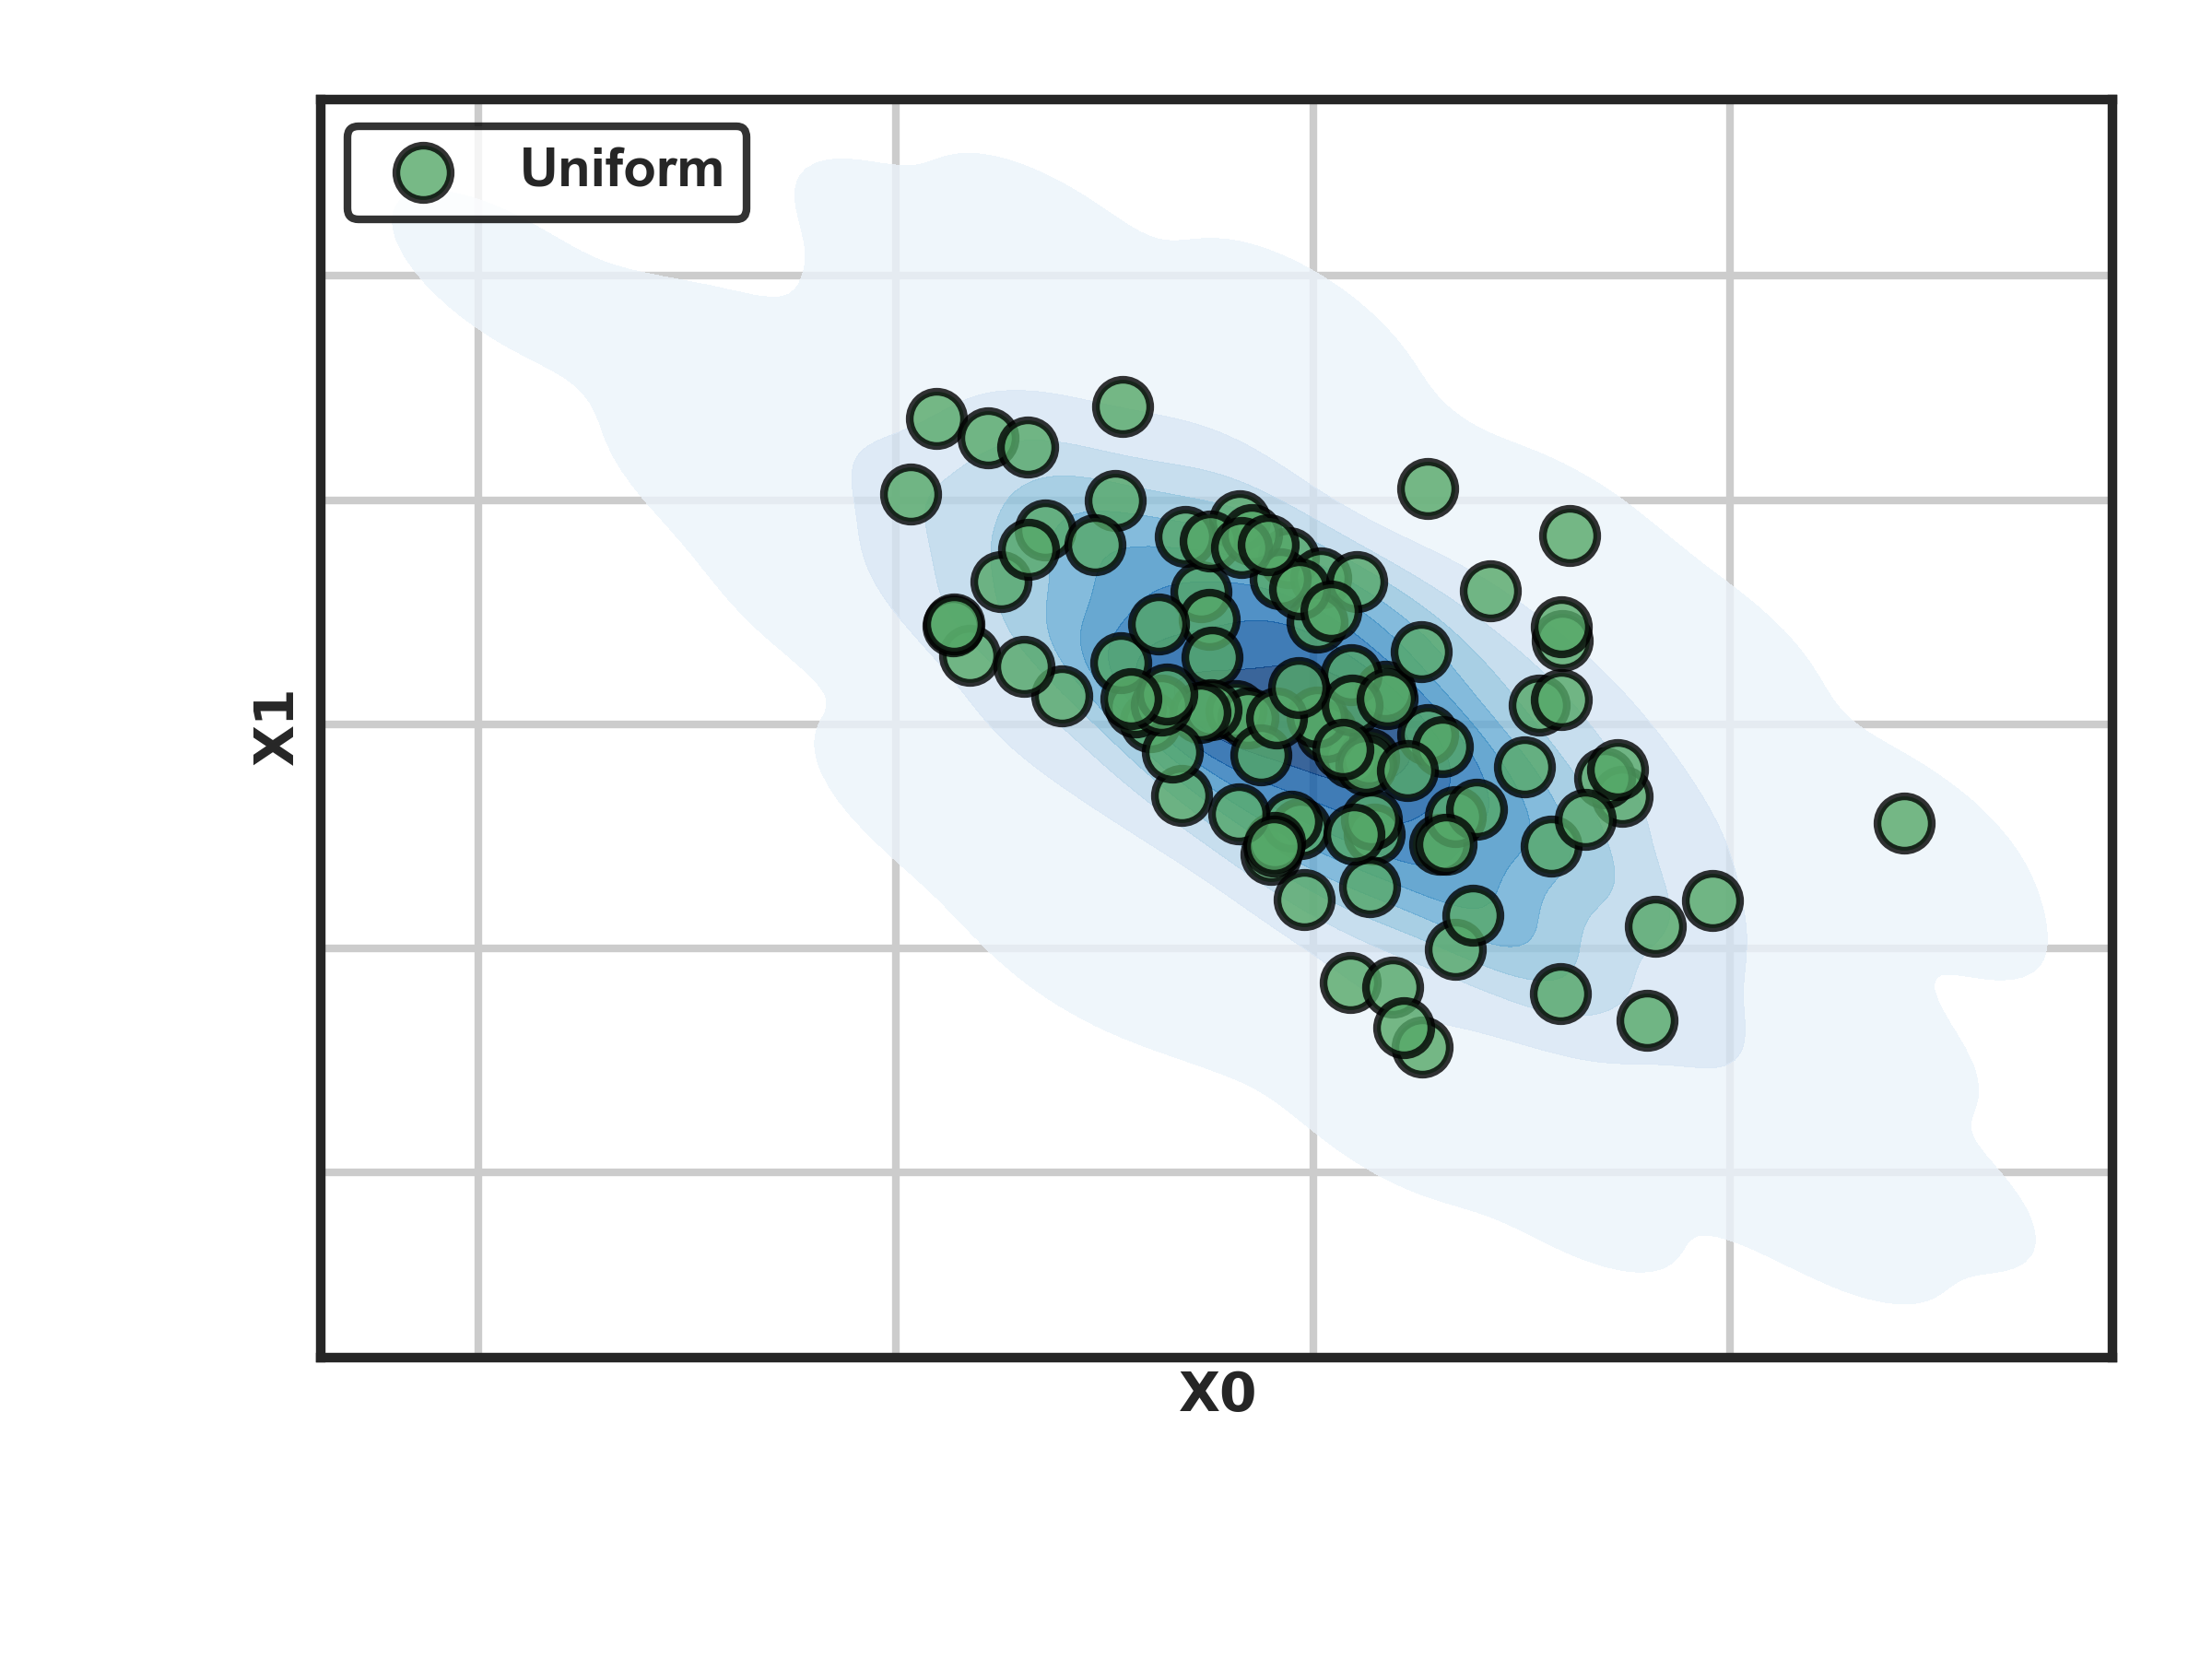}}
\subfloat[\textsc{Easy}]
{\includegraphics[width=0.32\textwidth]{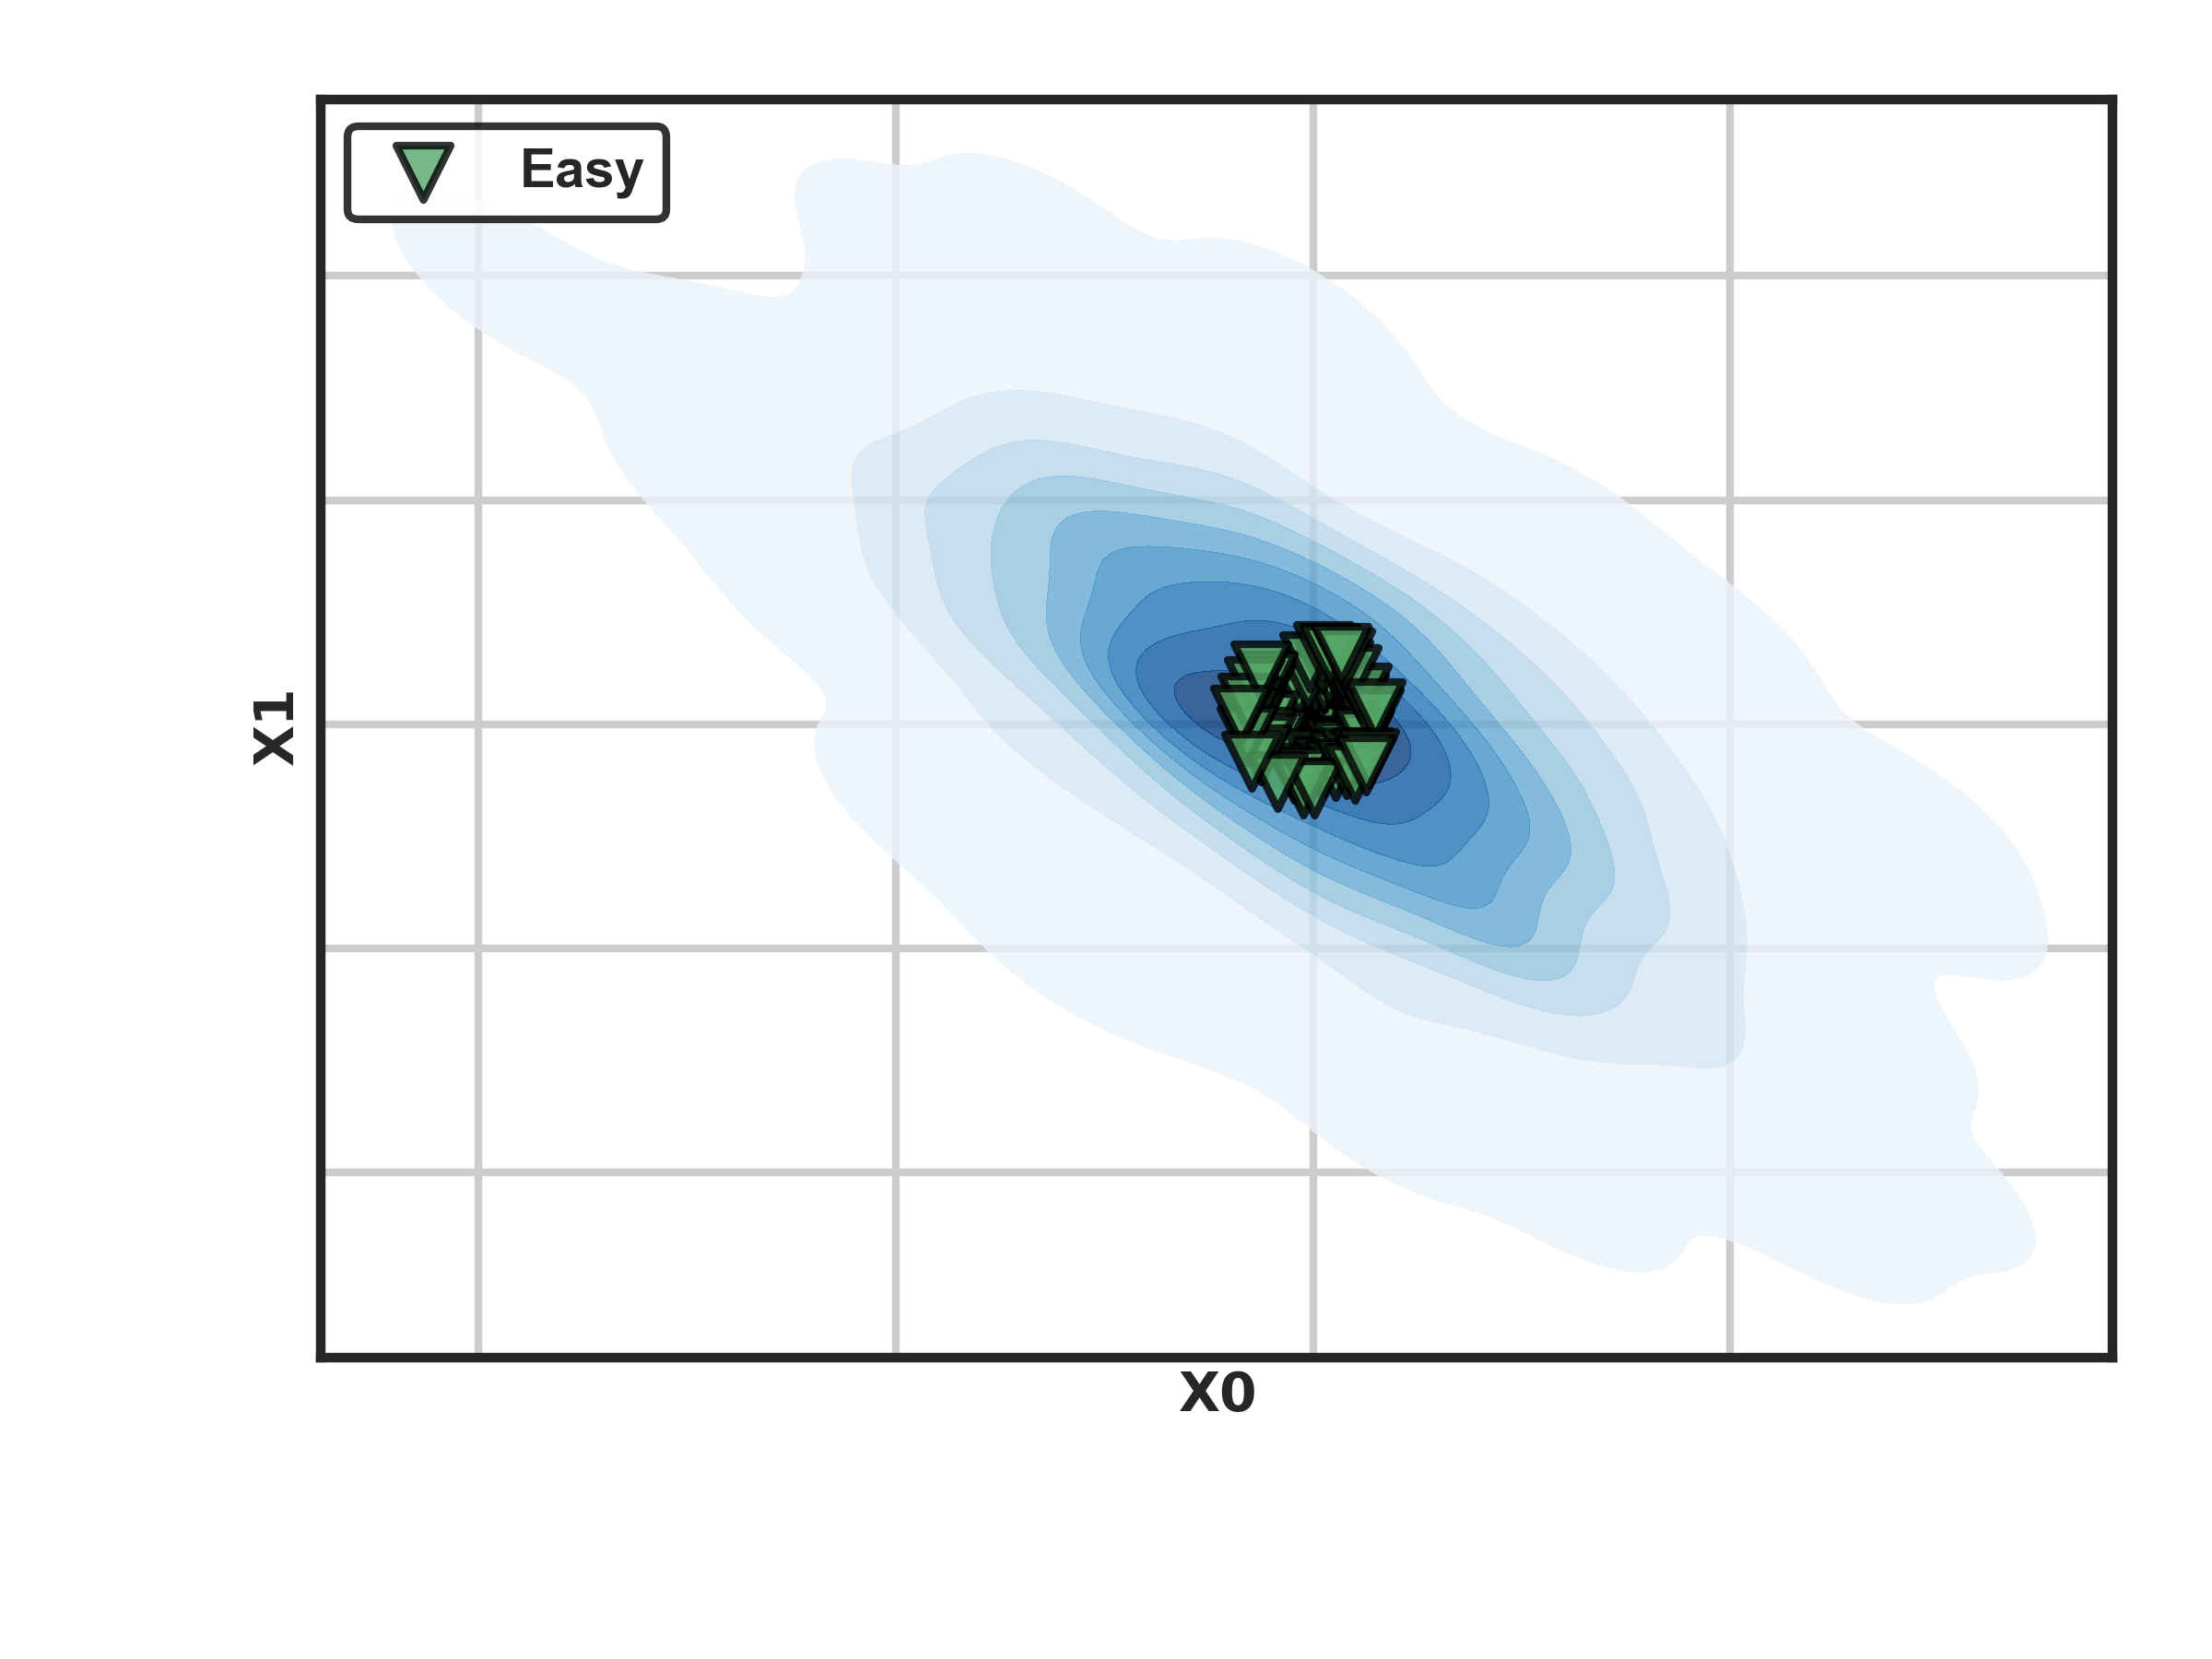}}
\subfloat[\textsc{Hard}]
{\includegraphics[width=0.32\textwidth]{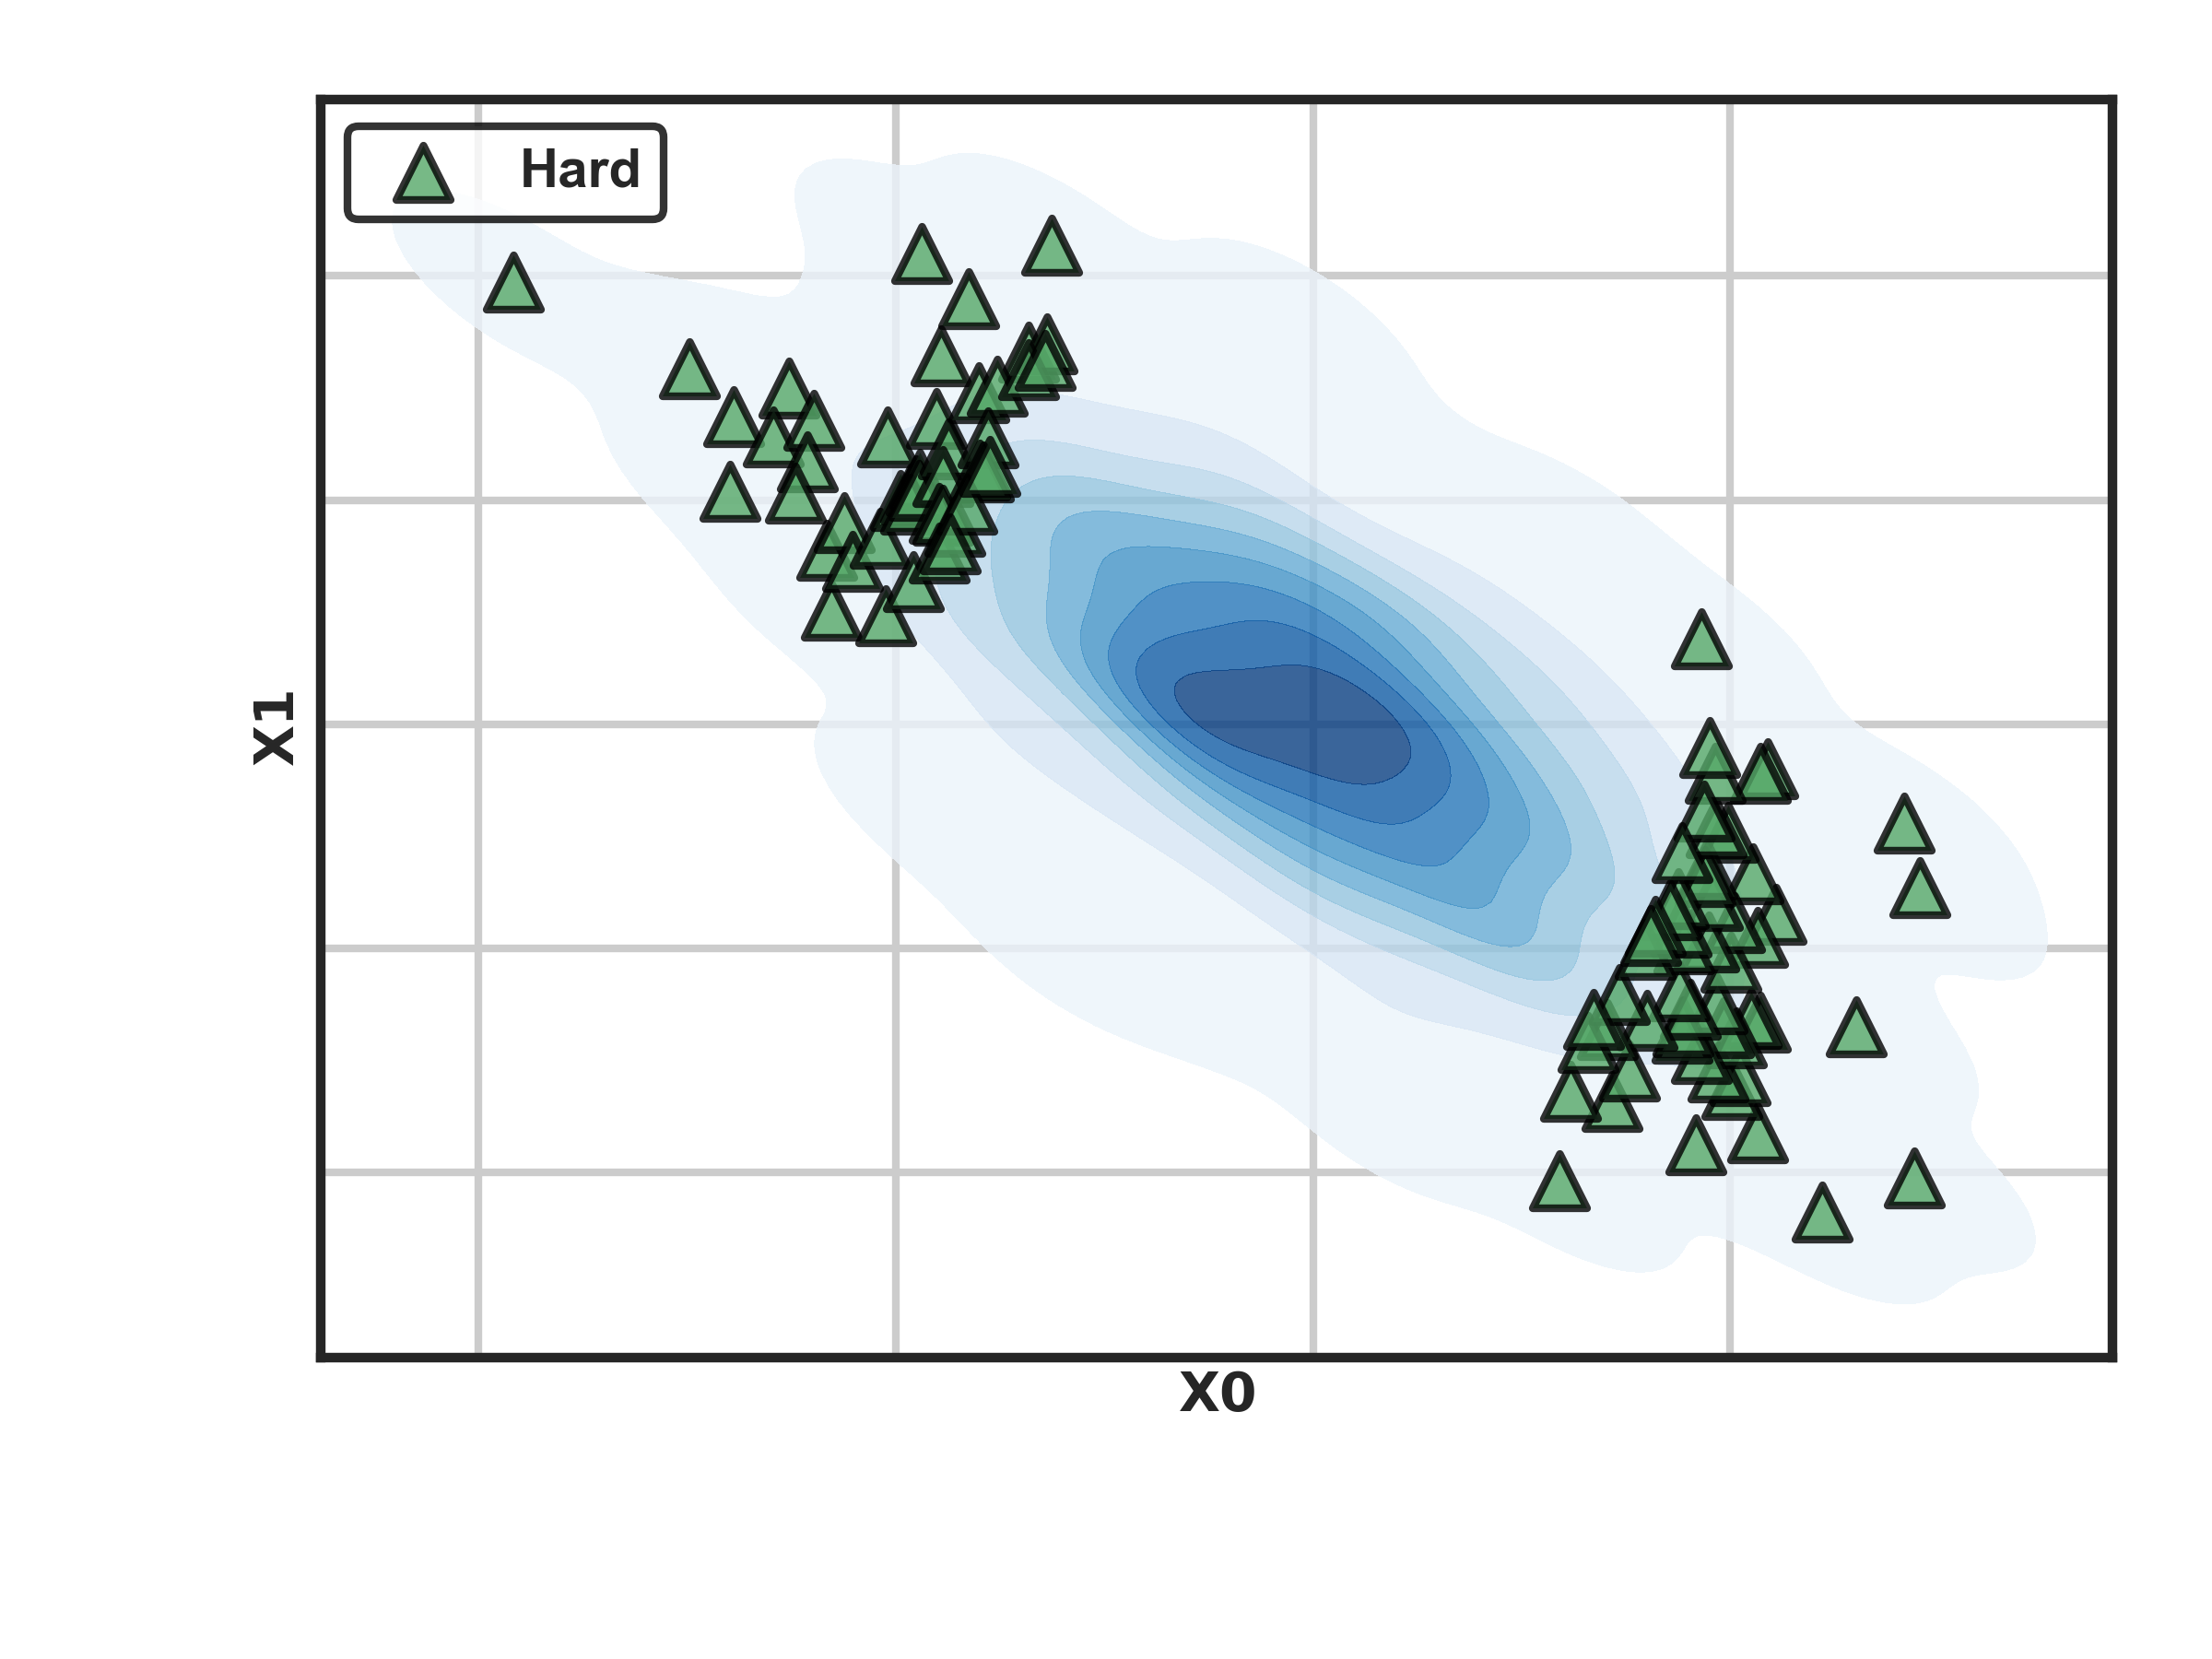}}
\\
\subfloat[\textsc{Moderate}]
{\includegraphics[width=0.32\textwidth]{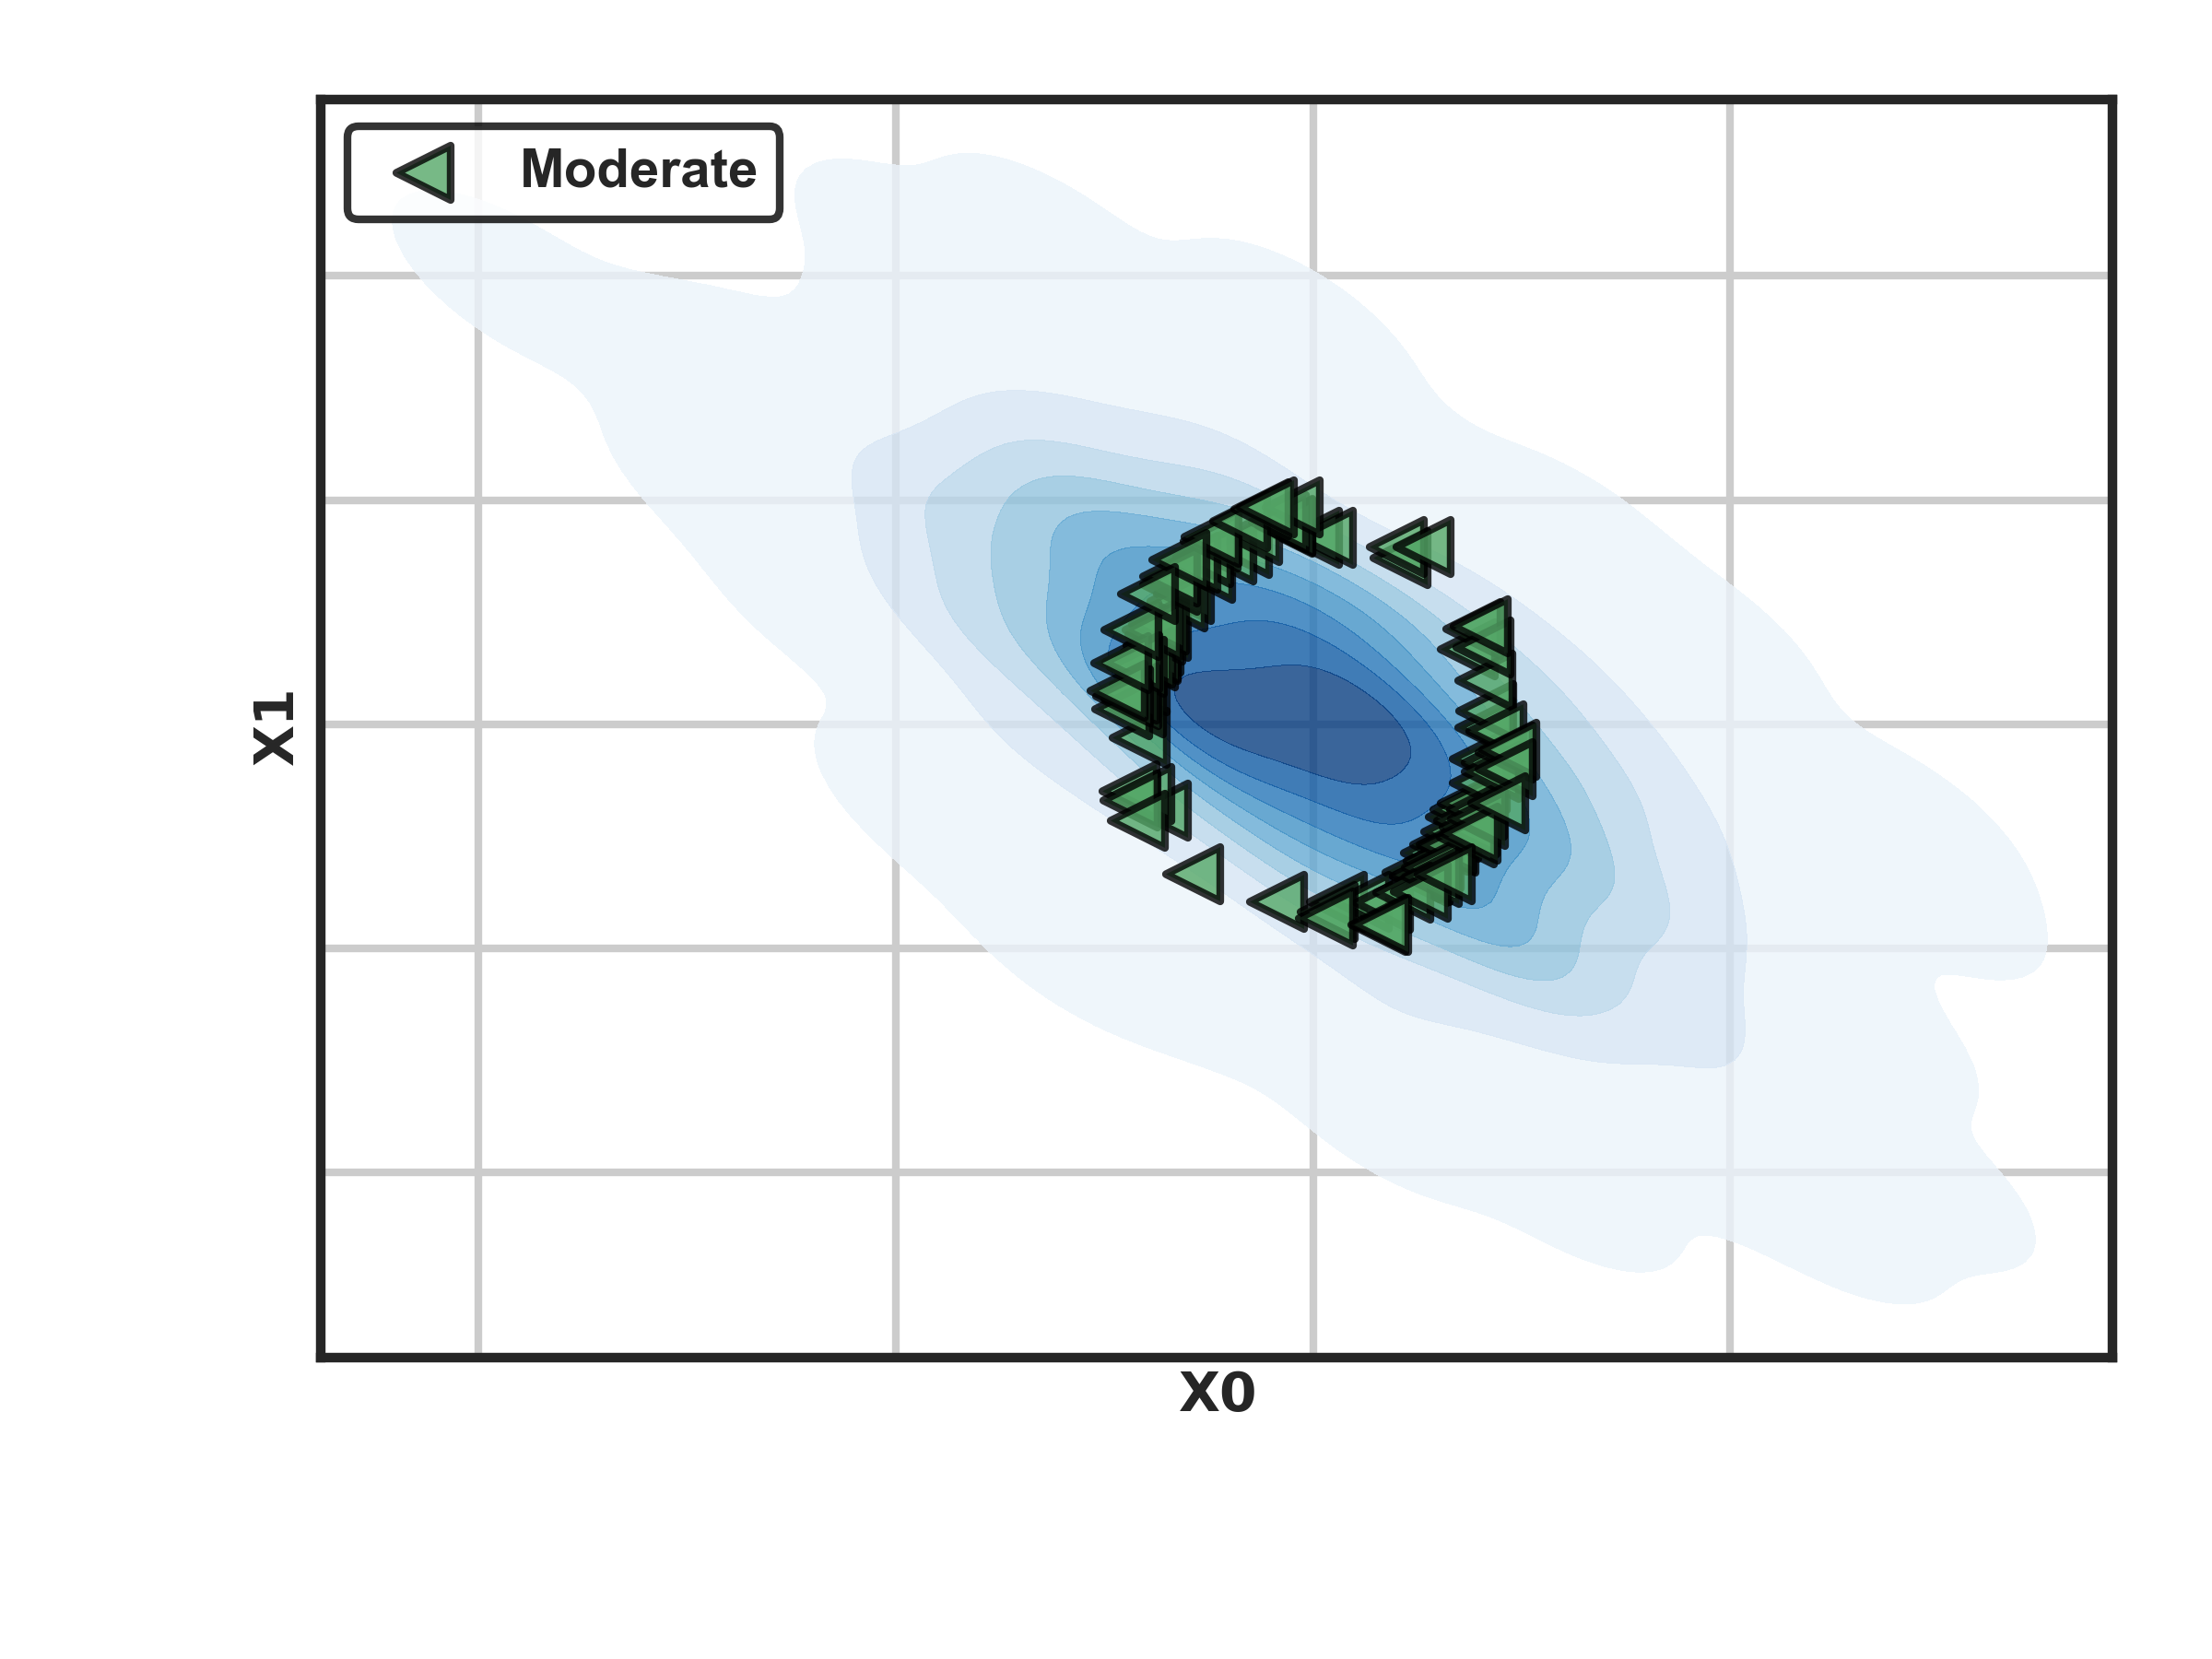}}
\subfloat[\textsc{Herding}]
{\includegraphics[width=0.32\textwidth]{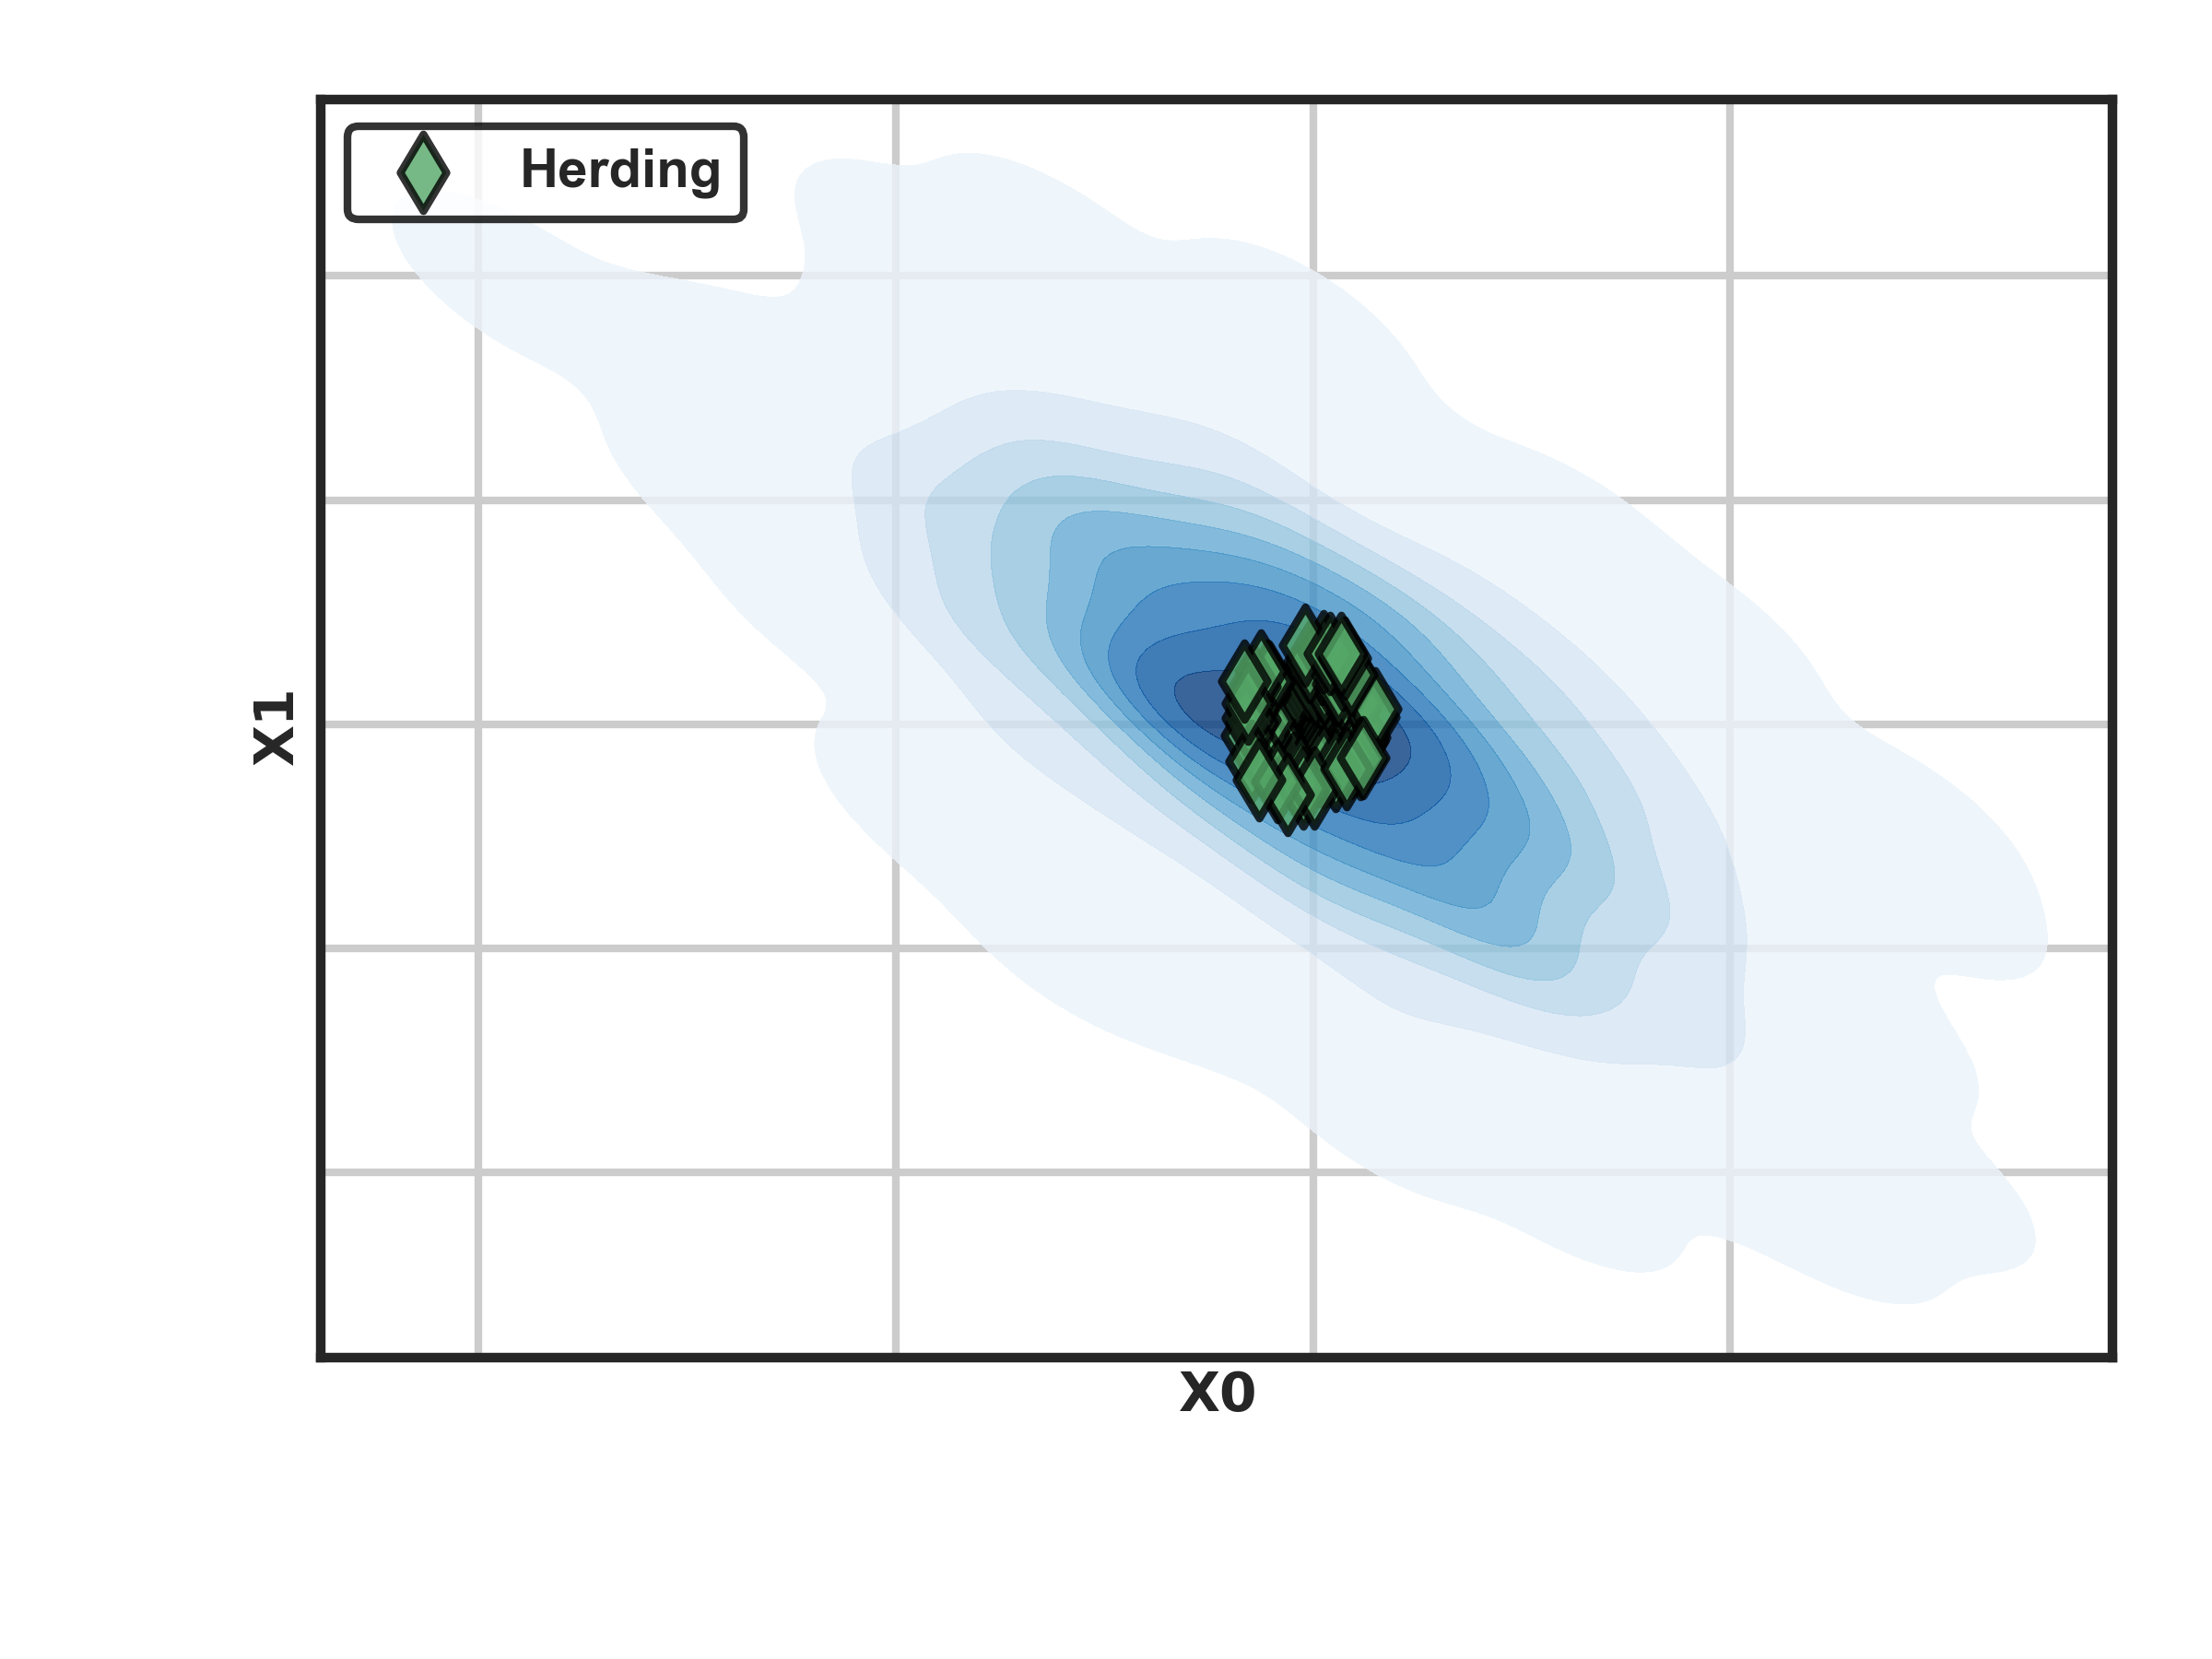}}
\subfloat[$\gm$ \textsc{Matching}]
{\includegraphics[width=0.32\textwidth]{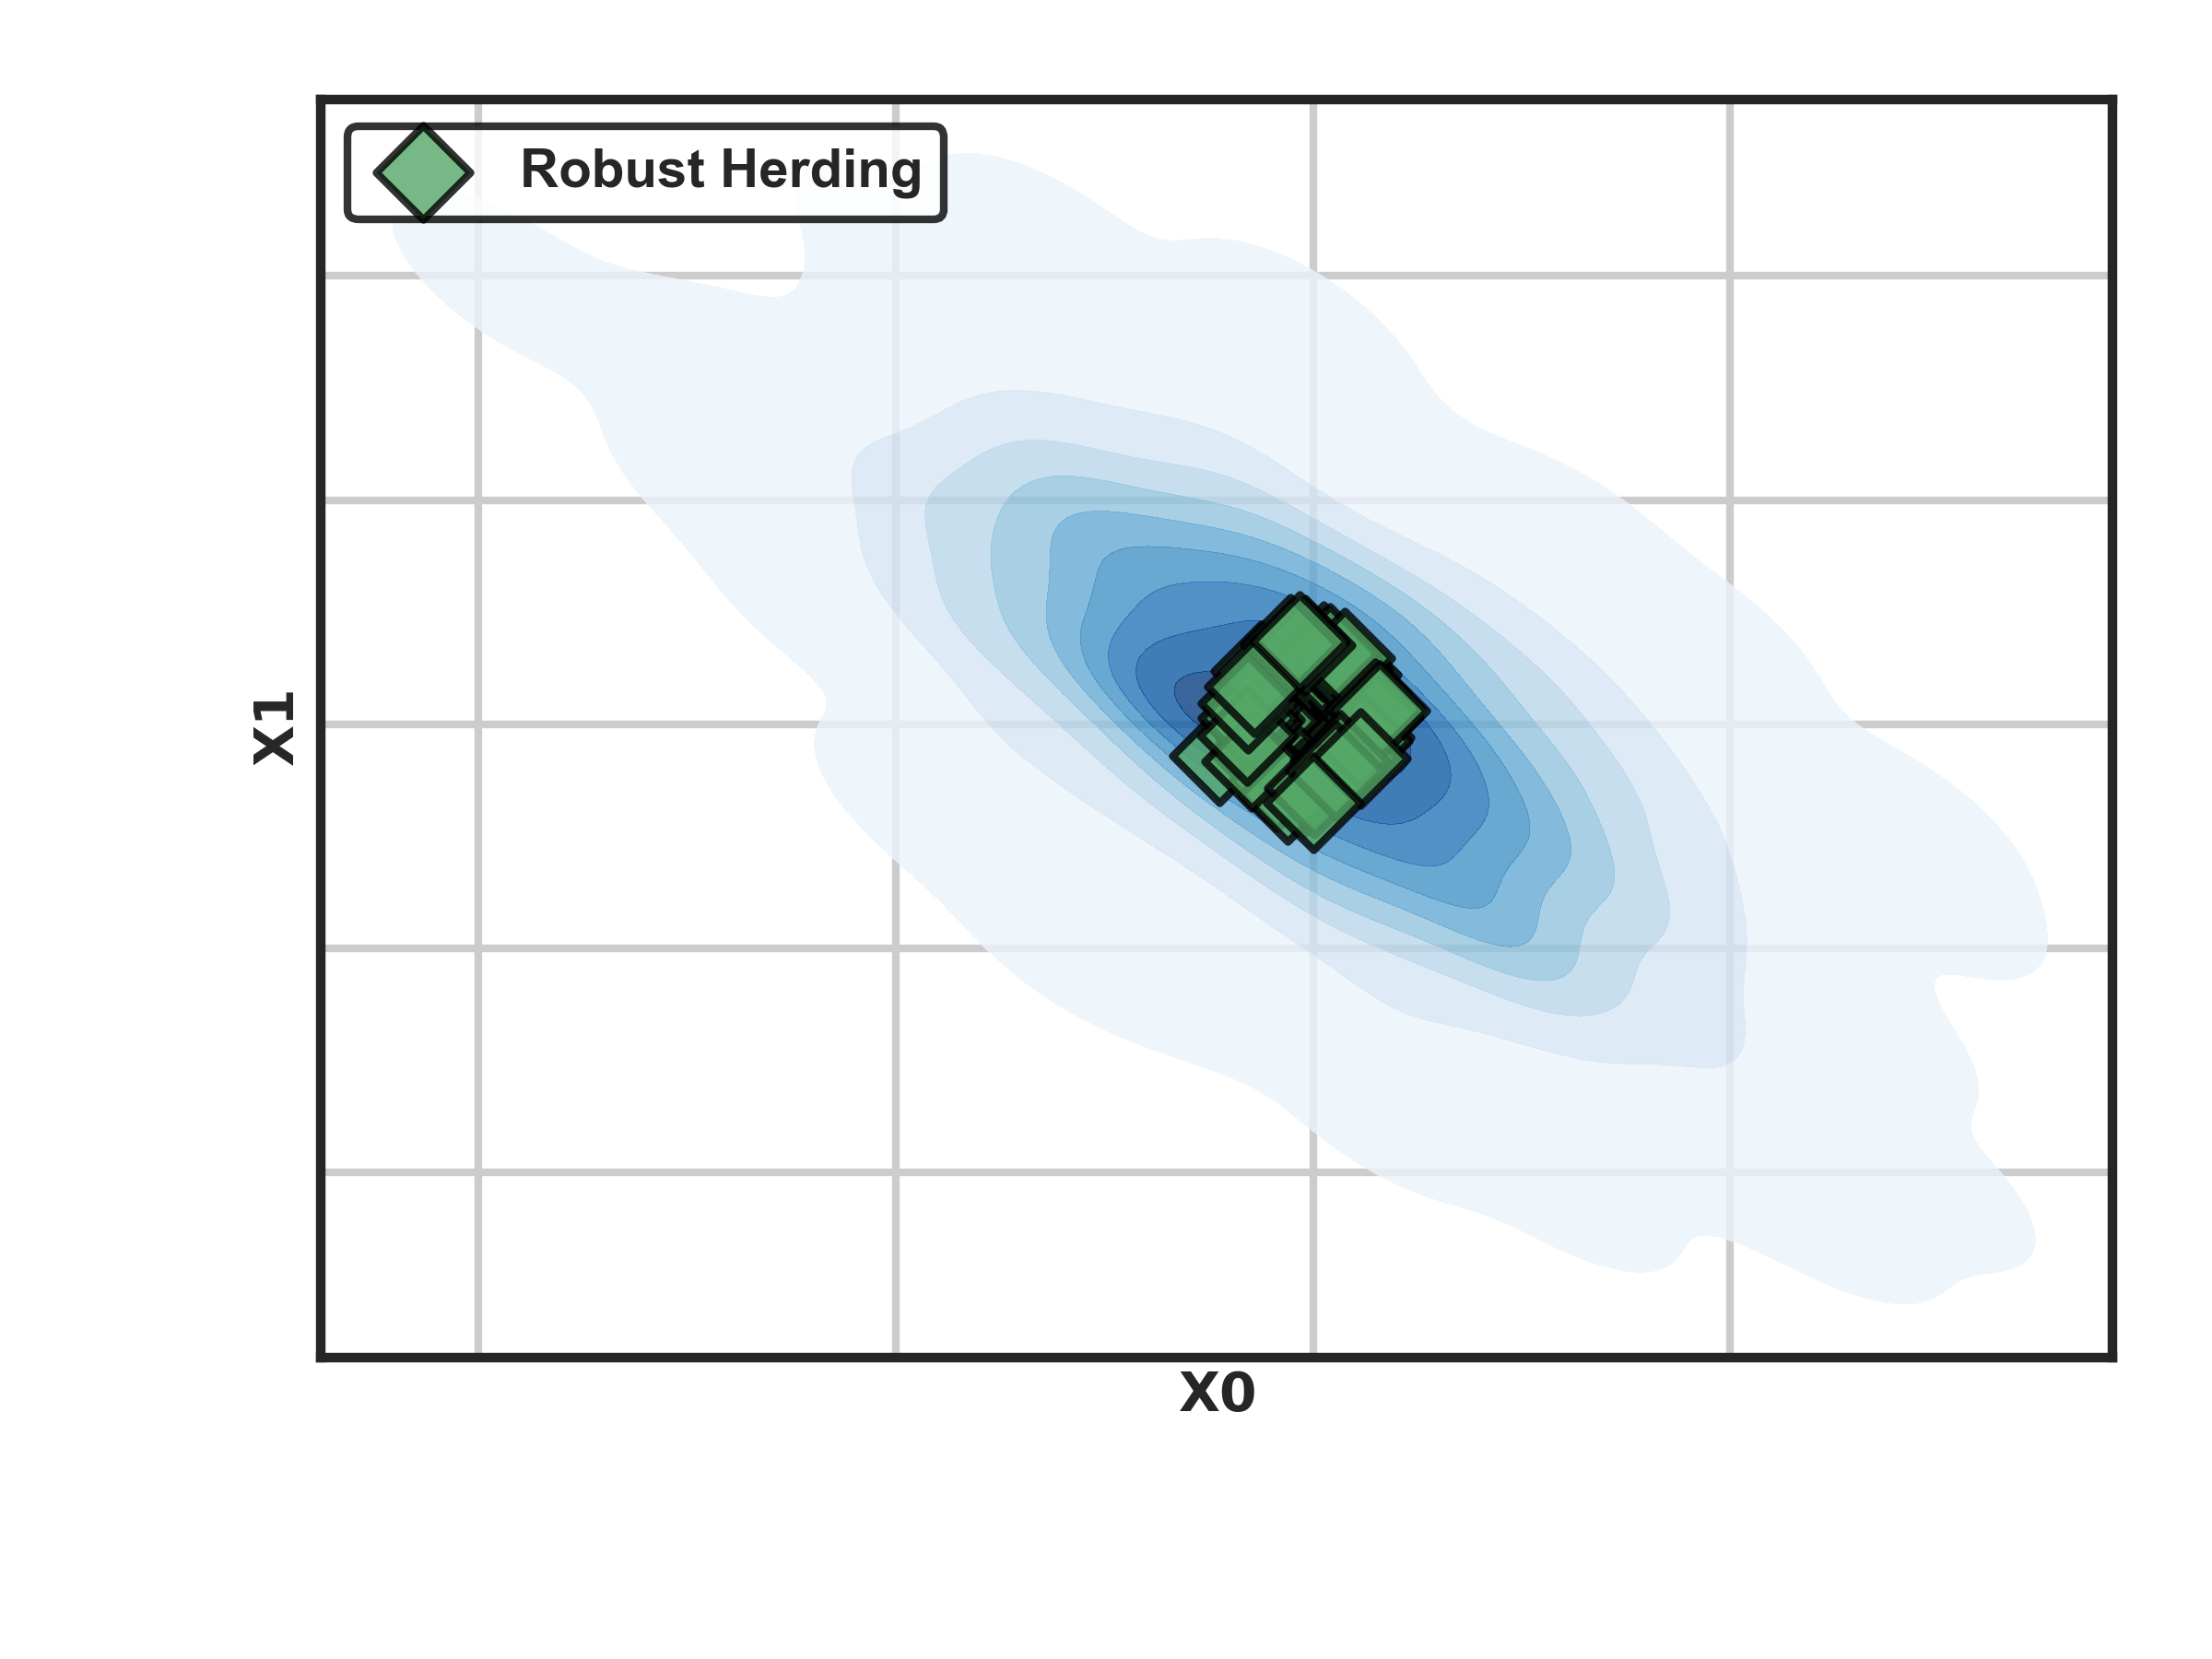}}
\caption{\footnotesize {\bf No Corruption :} We select 10\% of the samples using: (\textsc{Uniform}) Random Sampling, (\textsc{Easy}) Selection of samples closest to the centroid. (\textsc{Hard}) Selection of samples farthest from the centroid. (\textsc{Moderate}) Selection of samples closest to the median distance from the centroid. (\textsc{Herding}) Moment Matching, (\textsc{GM Matching}) Robust Moment (GM) Matching~\eqref{eq:gm_matching}.}

\label{fig:toy-corr=0}
\end{figure*}
\begin{figure*}[t]
\centering
\subfloat[\textsc{Uniform}]
{\includegraphics[width=0.32\textwidth]{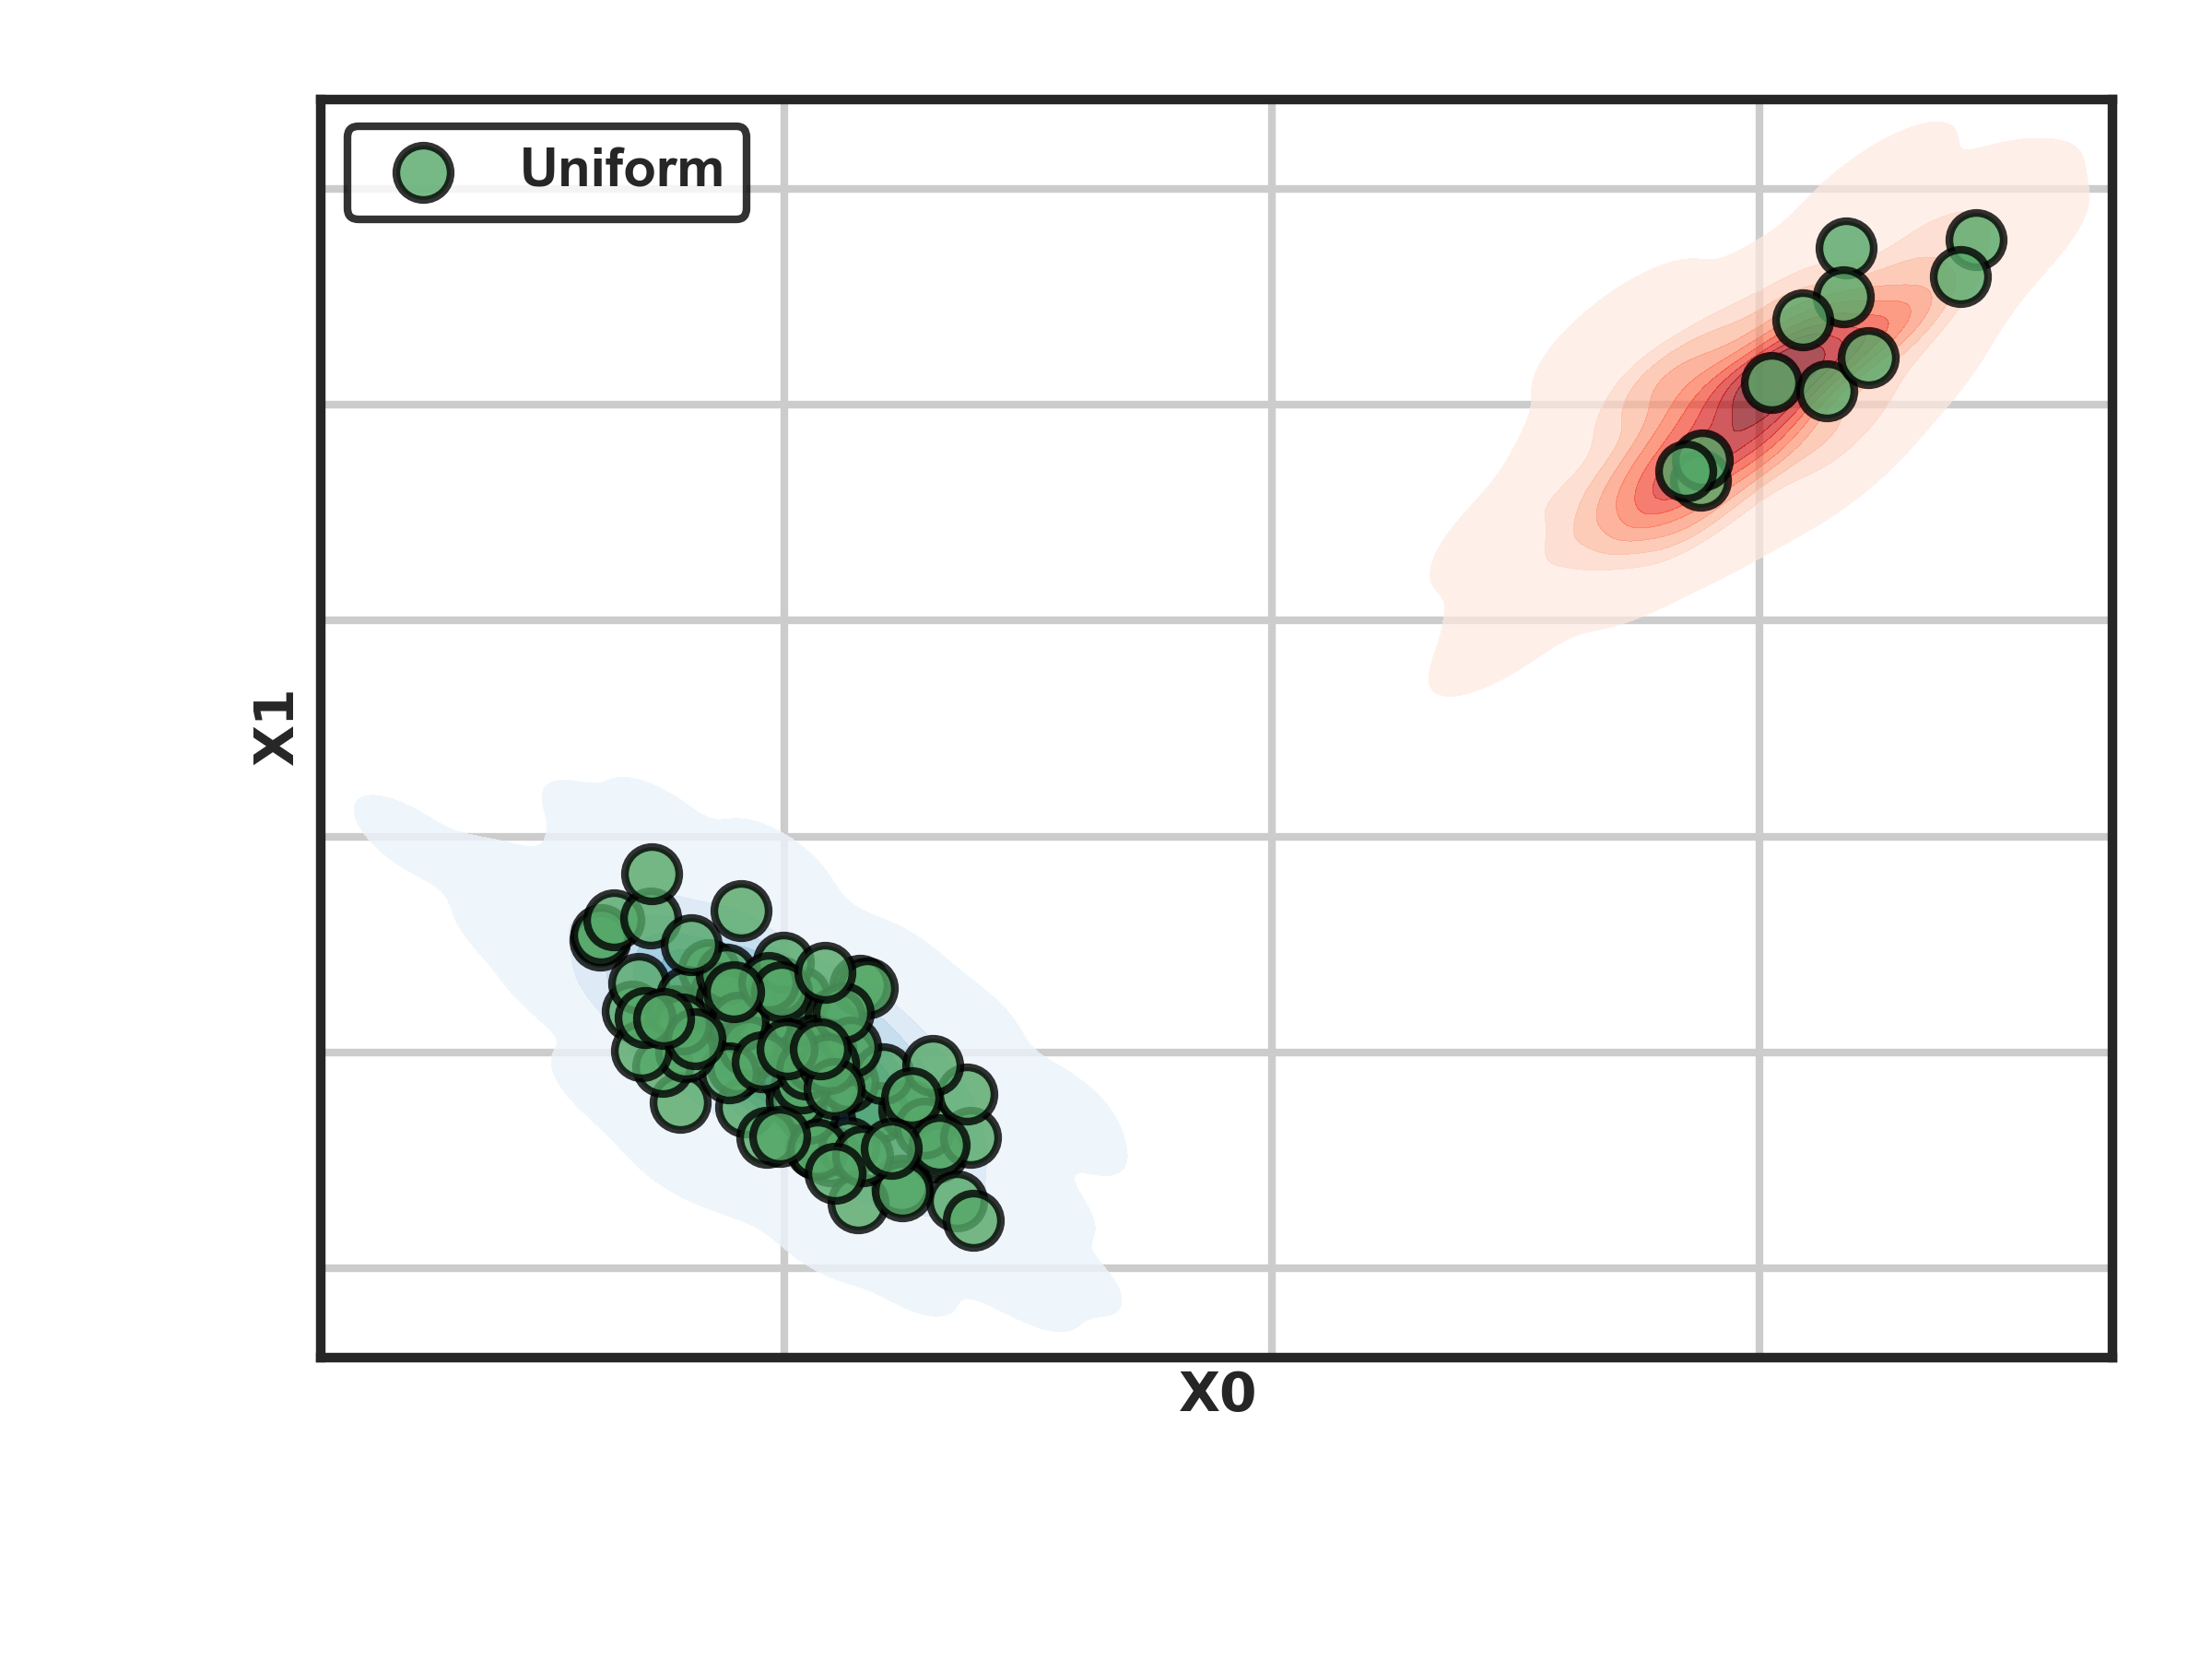}}
\subfloat[\textsc{Easy}]
{\includegraphics[width=0.32\textwidth]{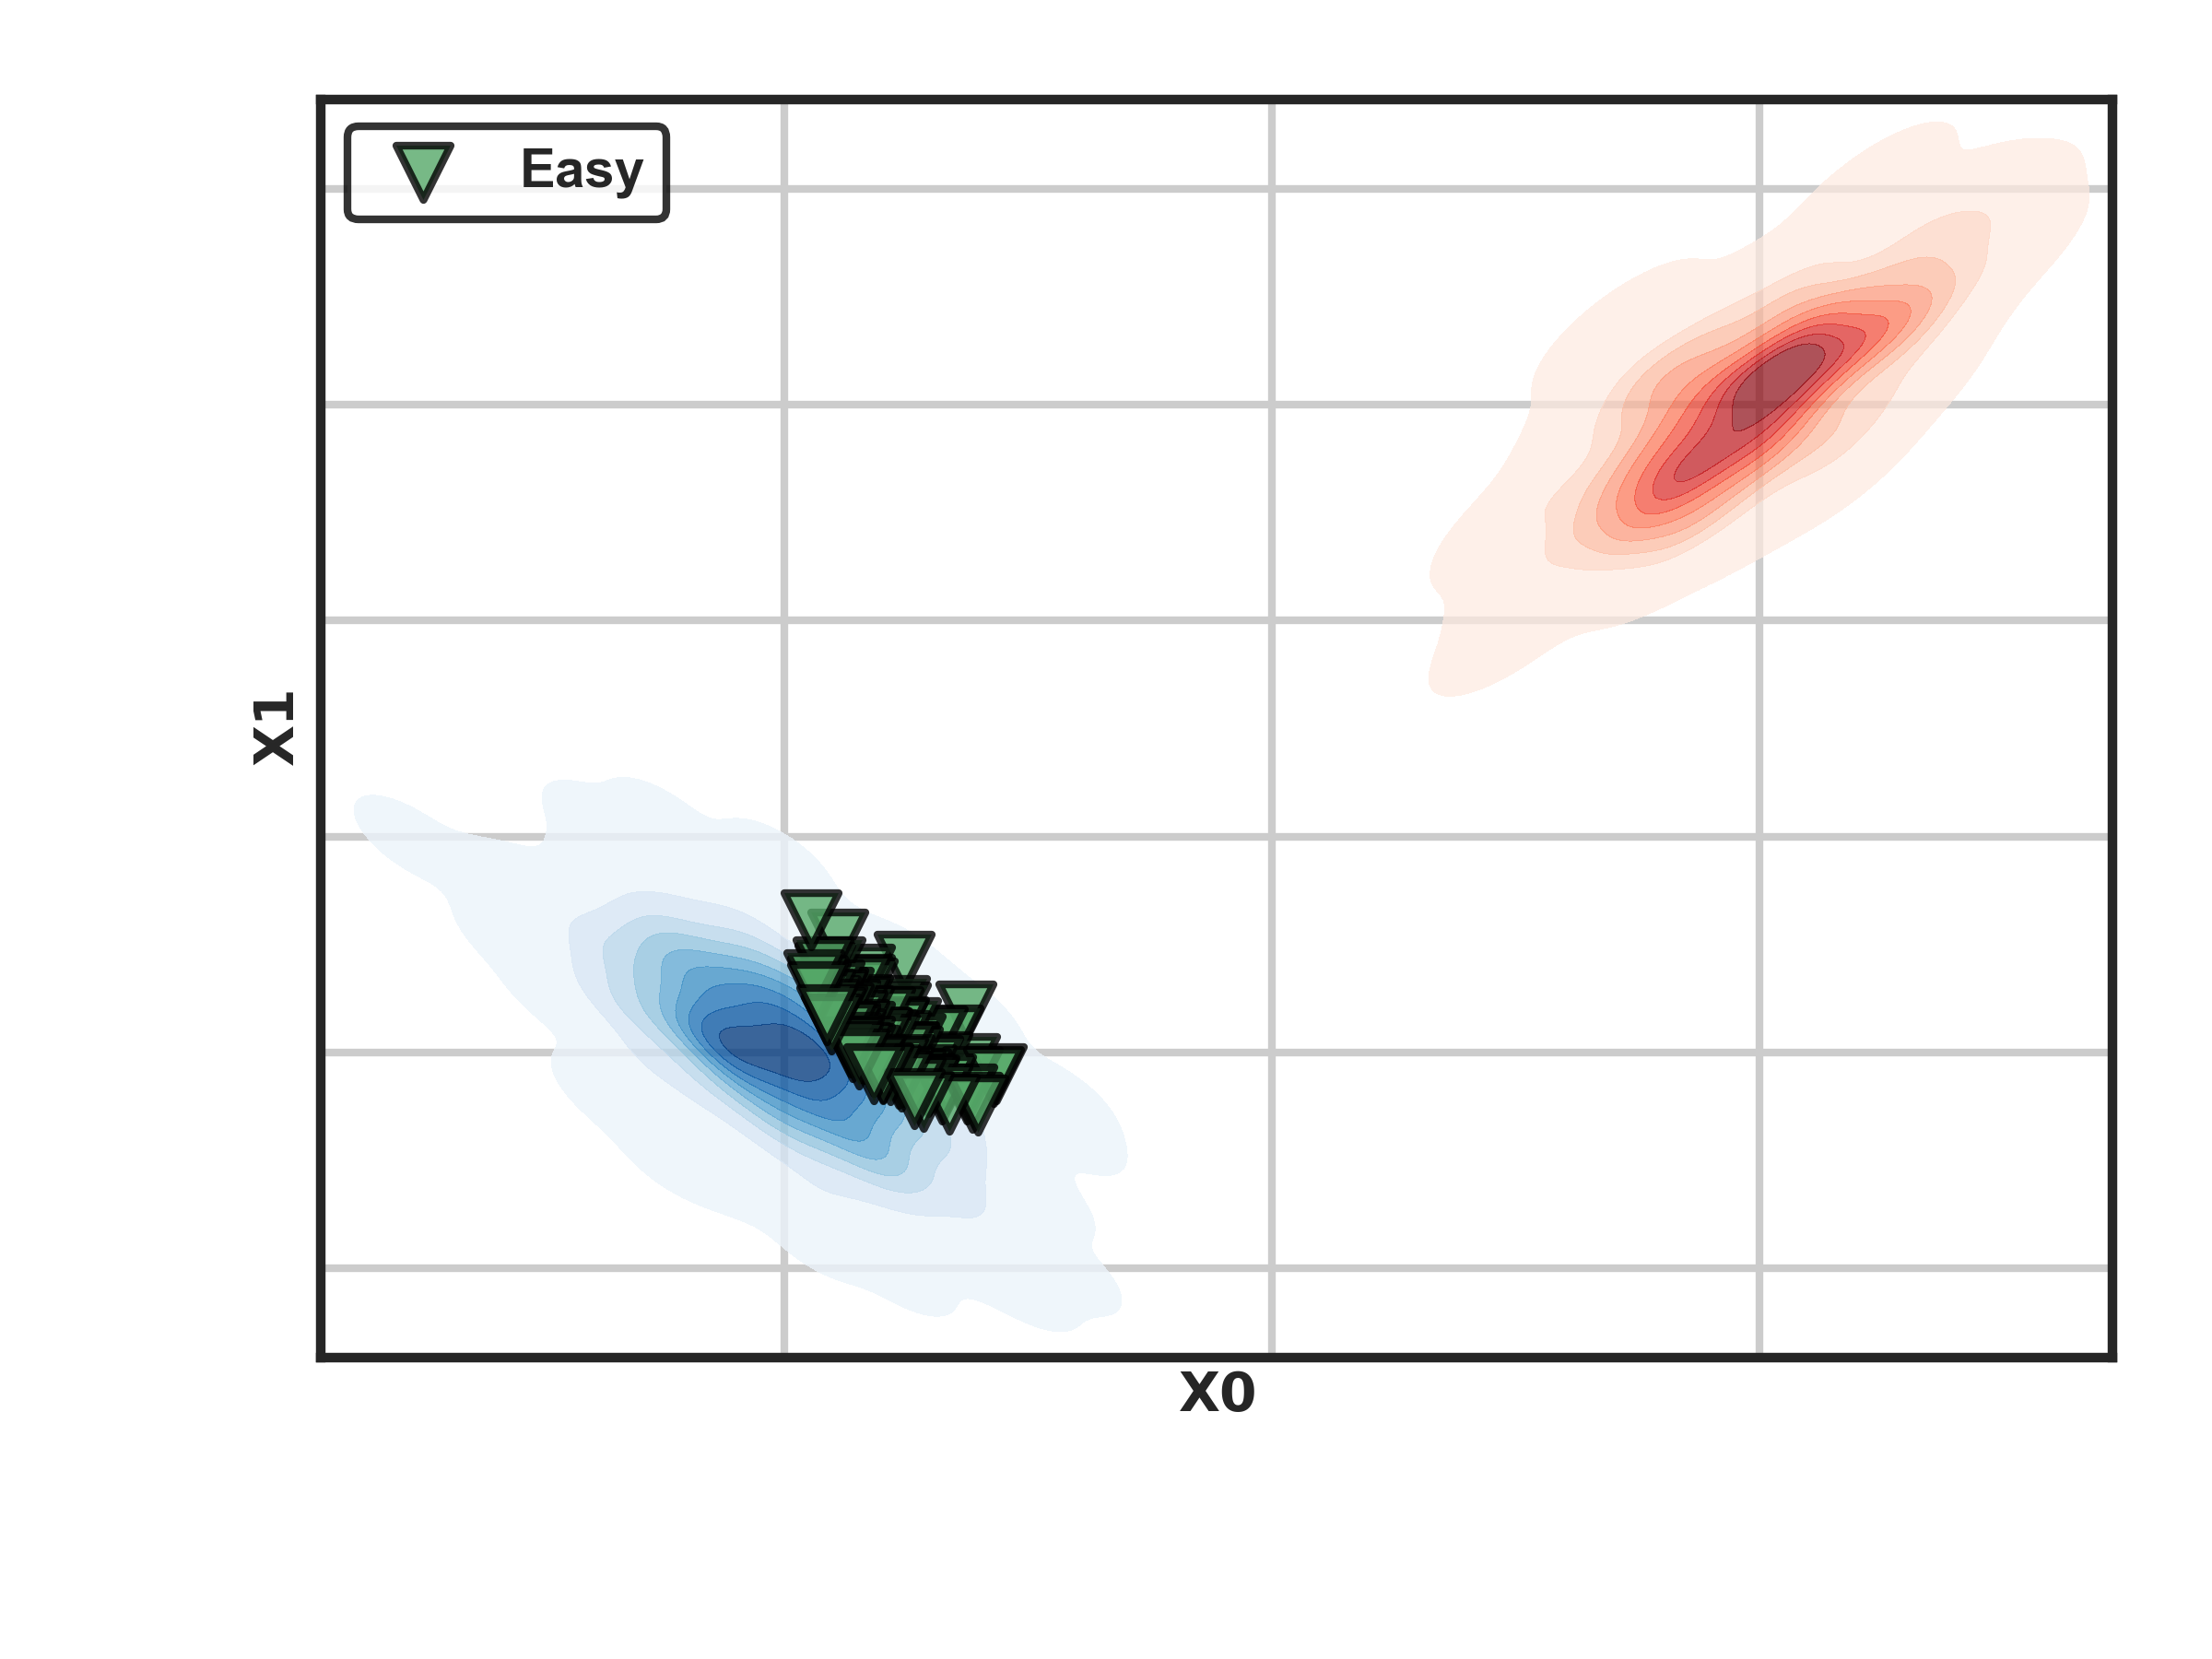}}
\subfloat[\textsc{Hard}]
{\includegraphics[width=0.32\textwidth]{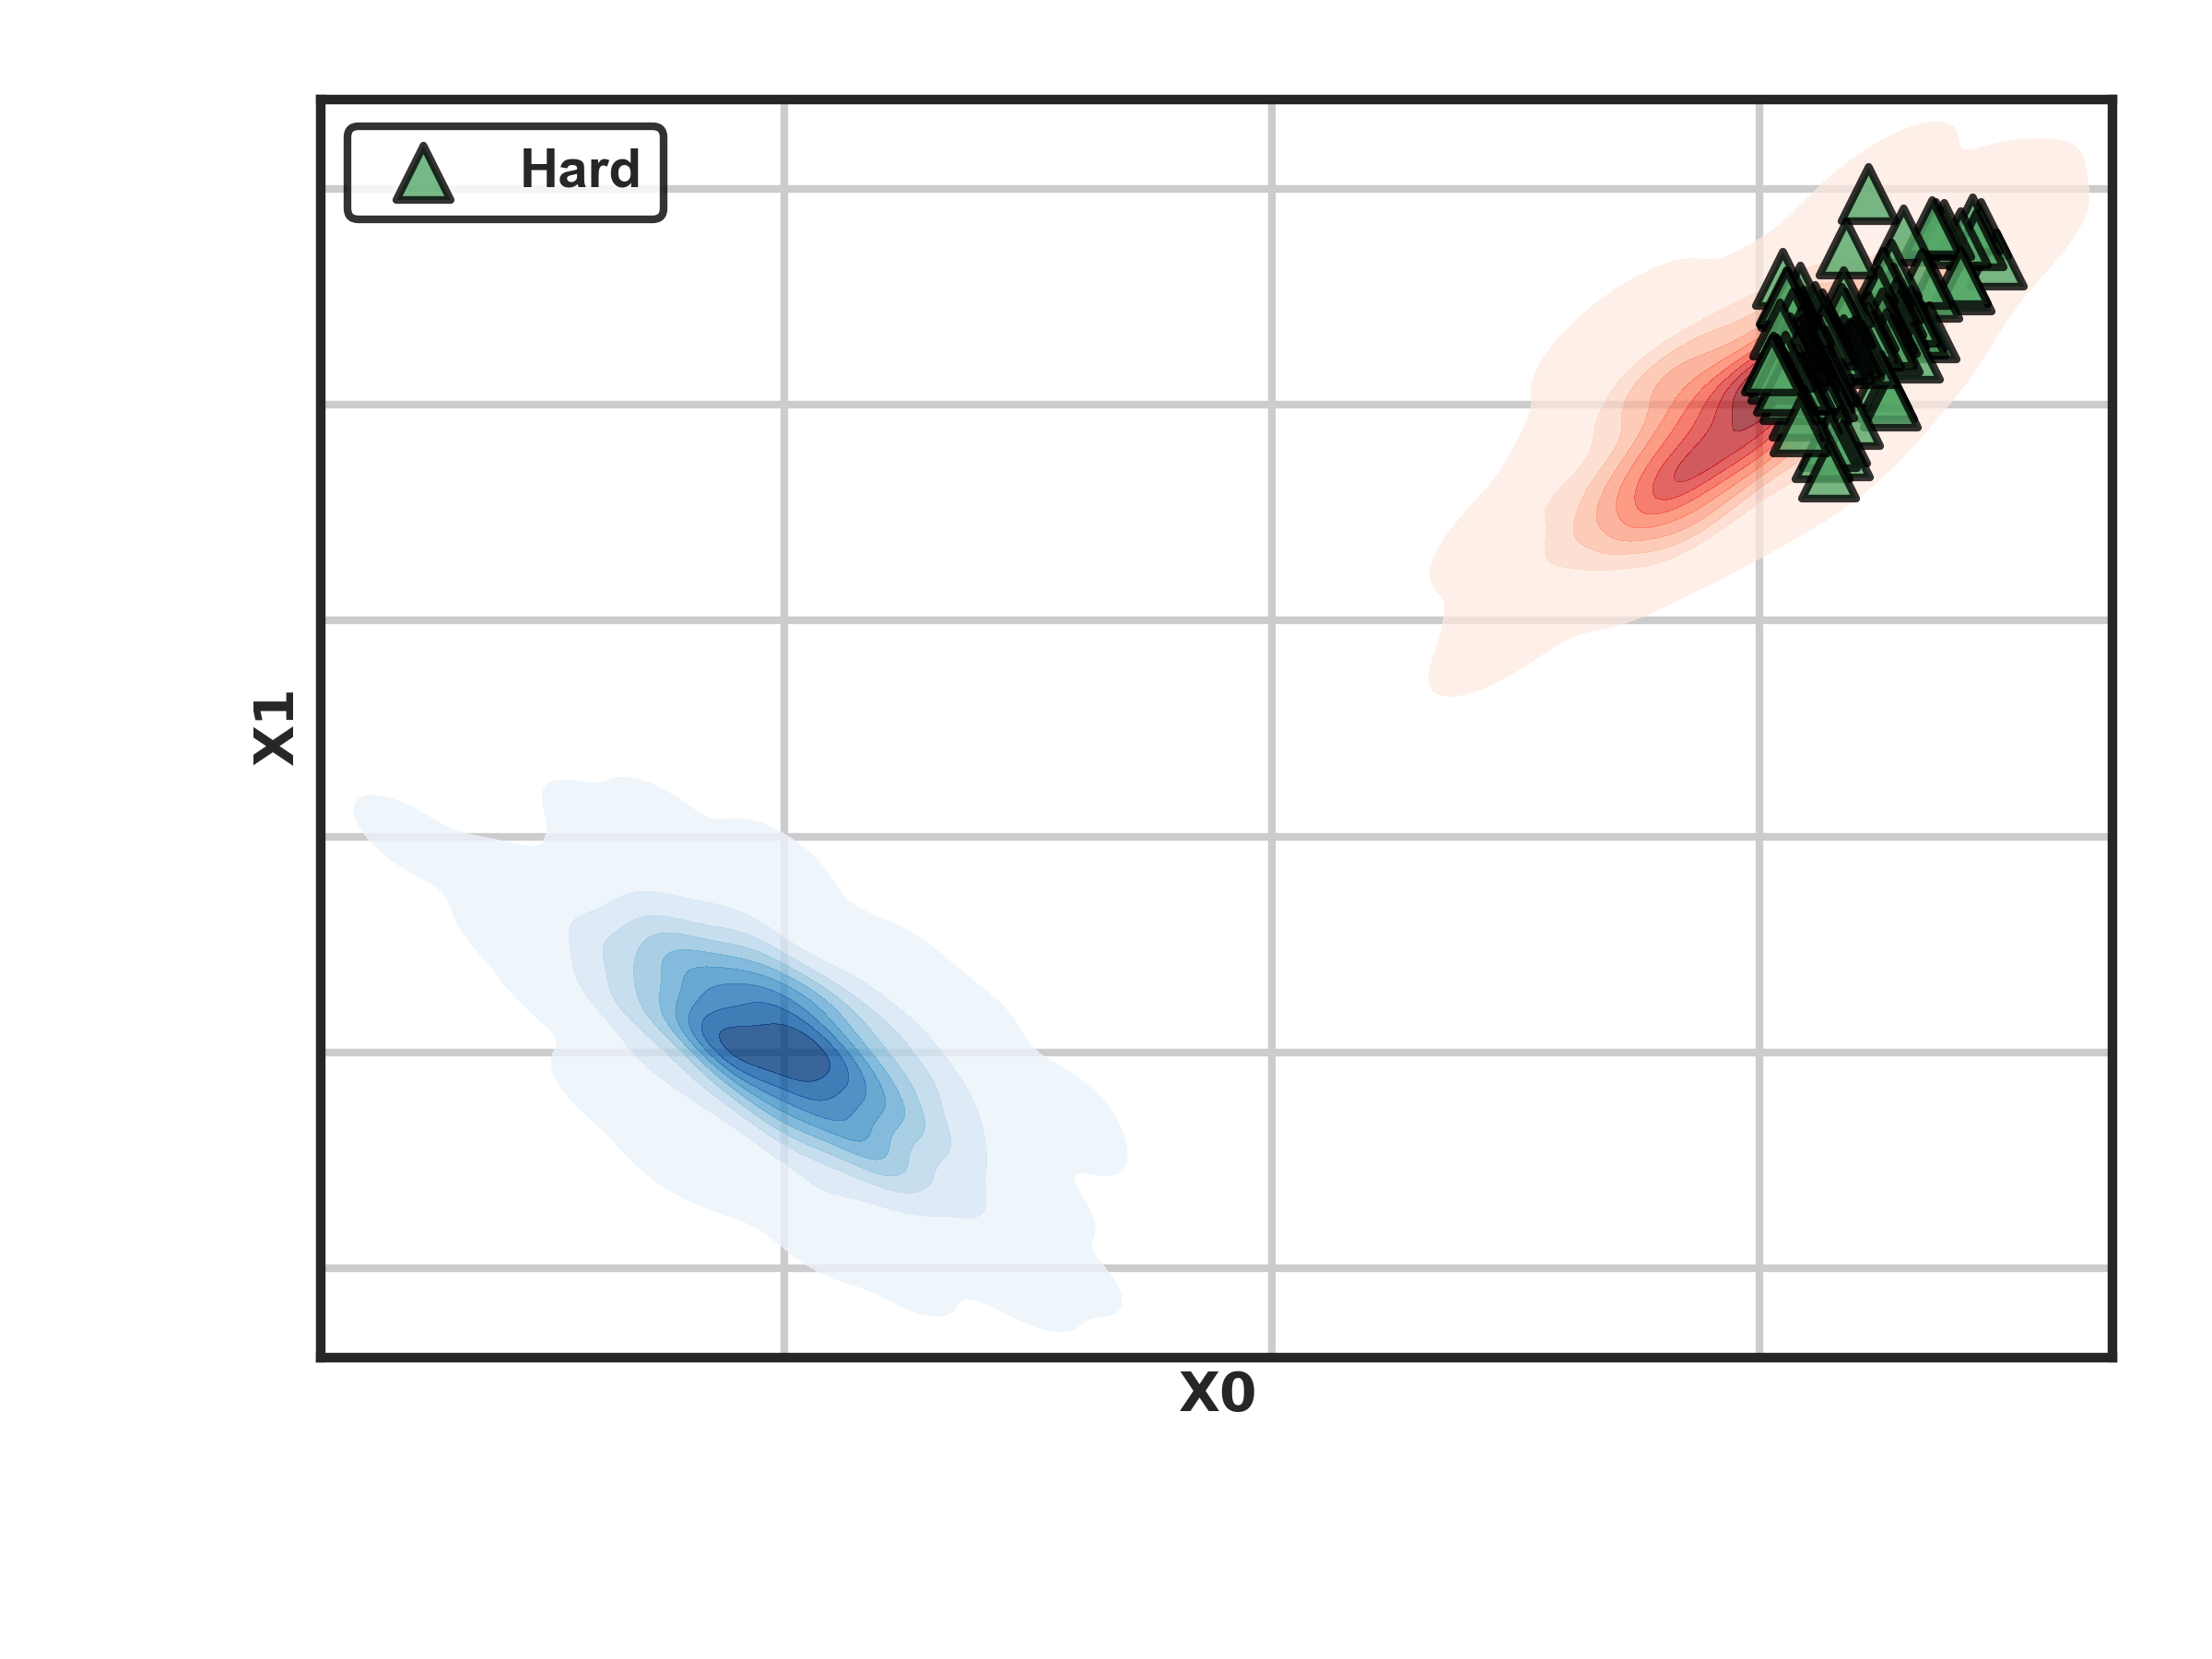}}
\\
\subfloat[\textsc{Moderate}]
{\includegraphics[width=0.32\textwidth]{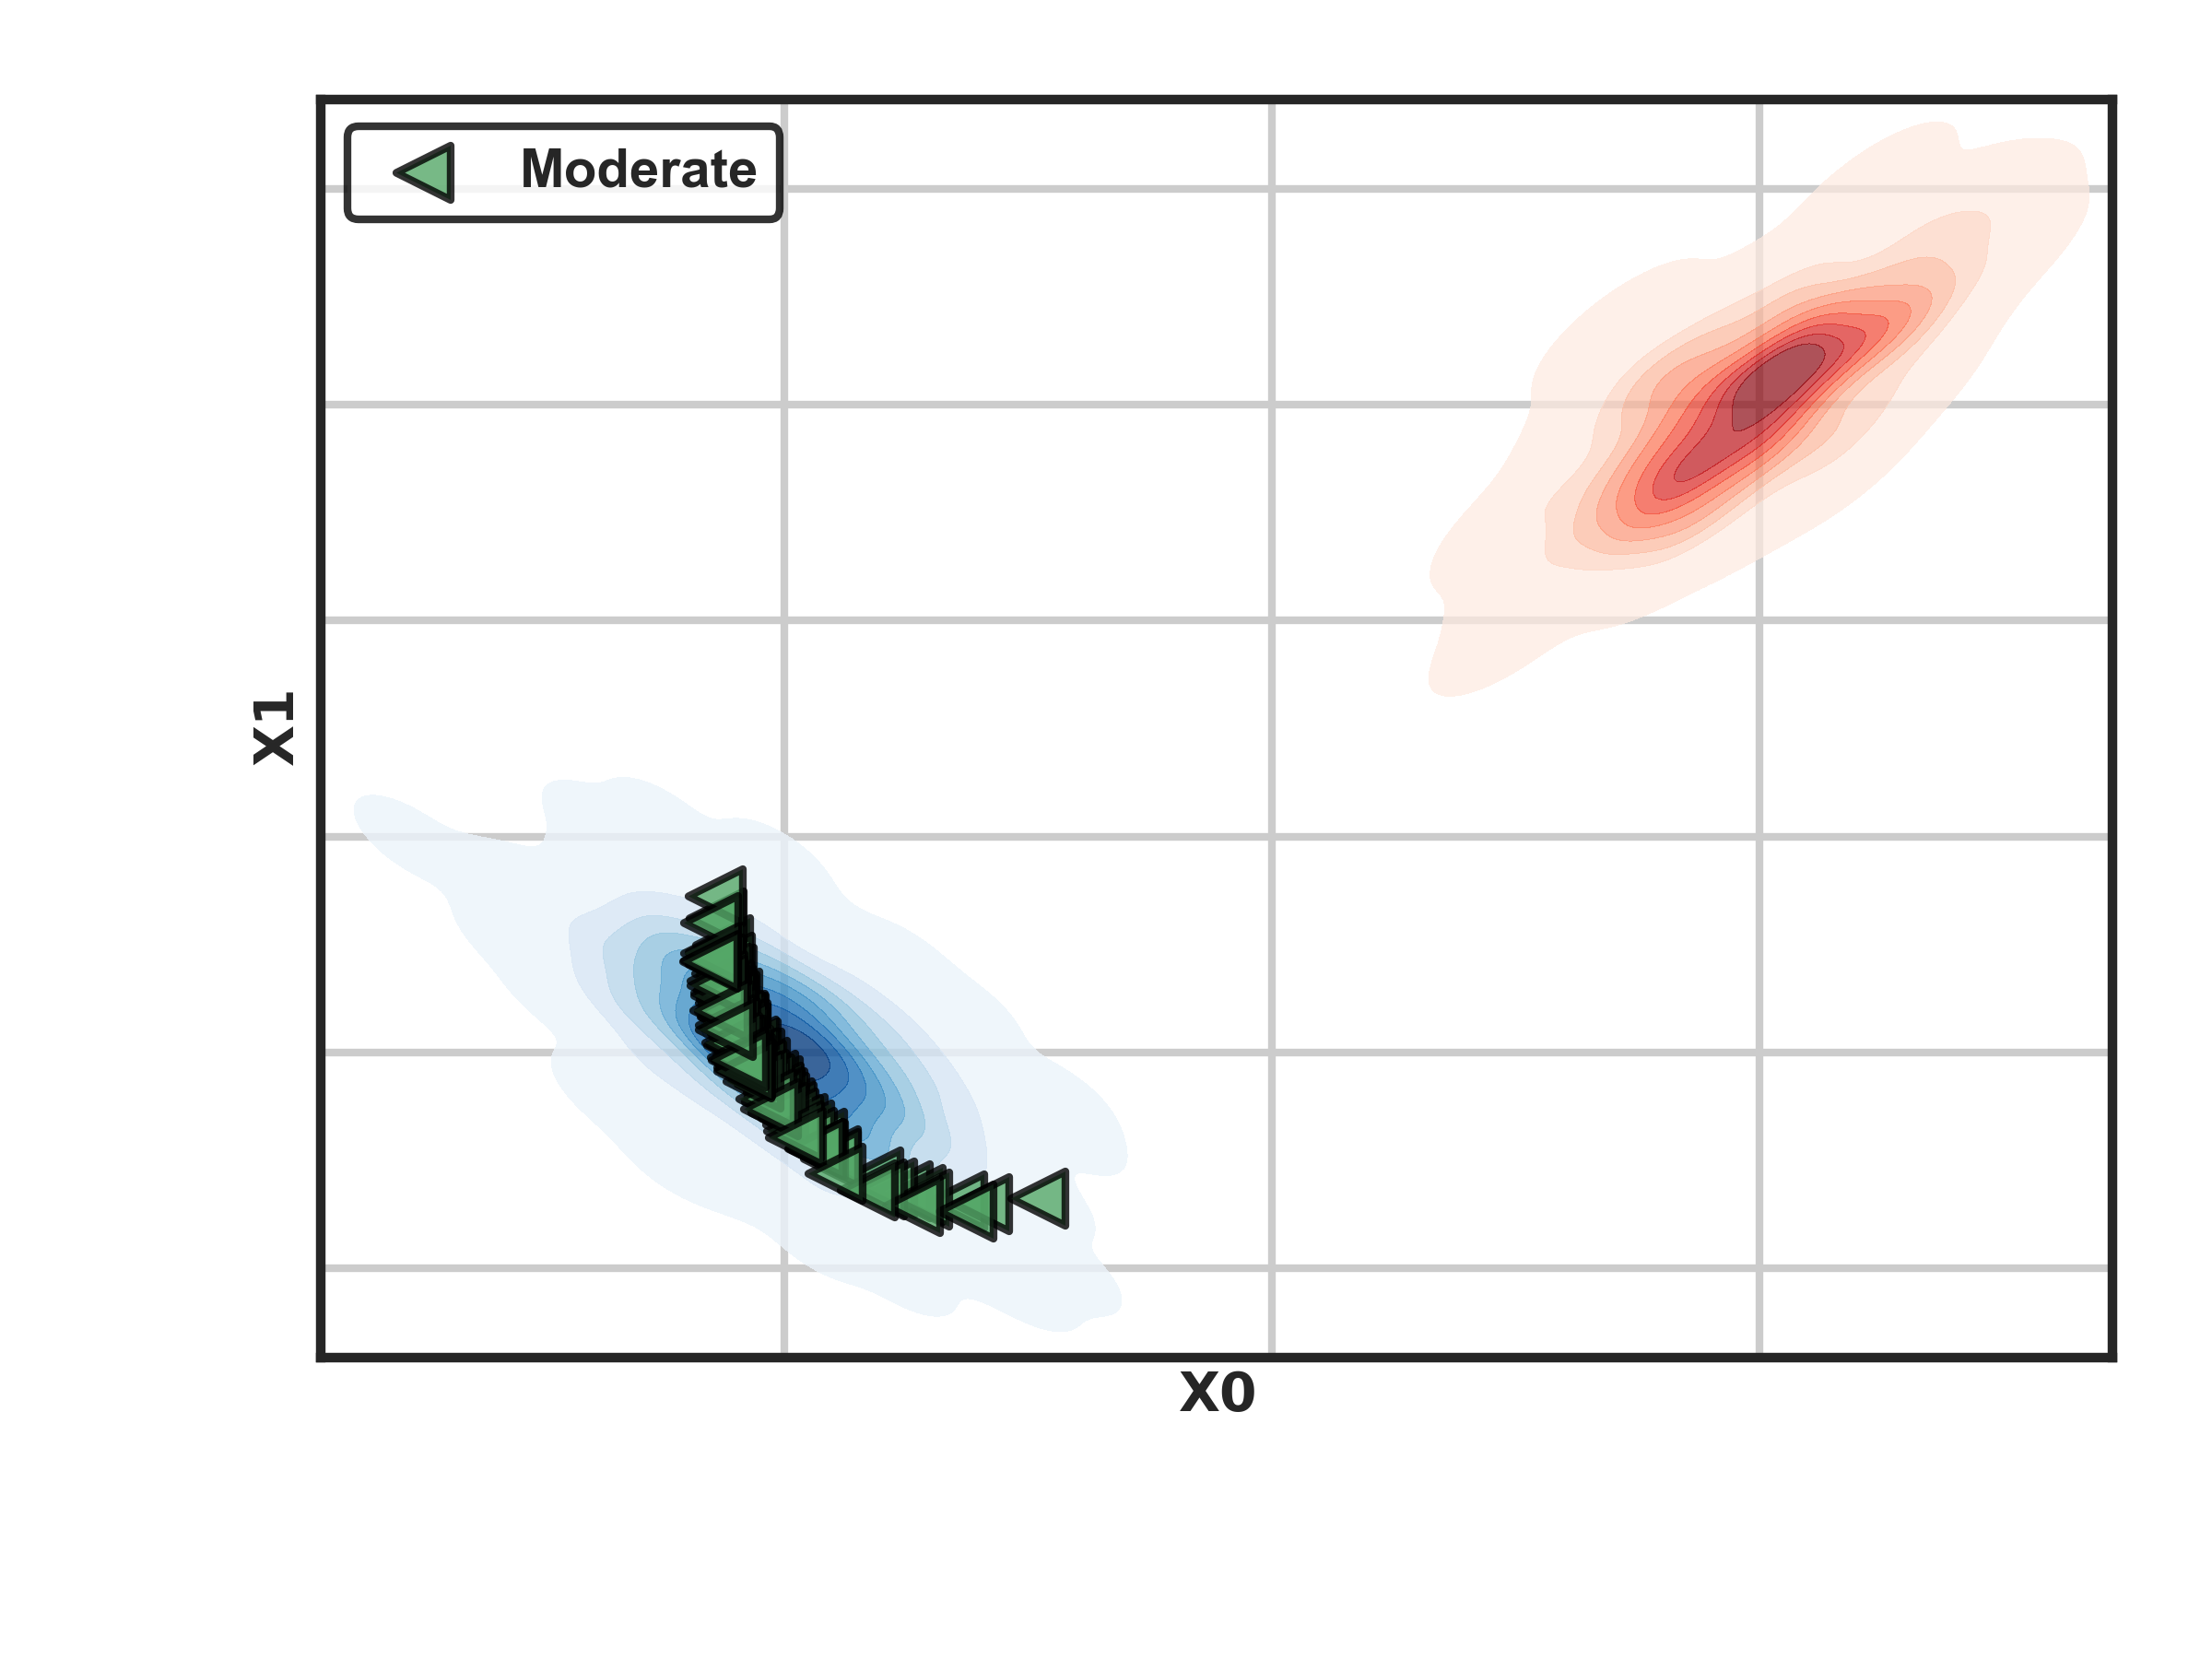}}
\subfloat[\textsc{Herding}]
{\includegraphics[width=0.32\textwidth]{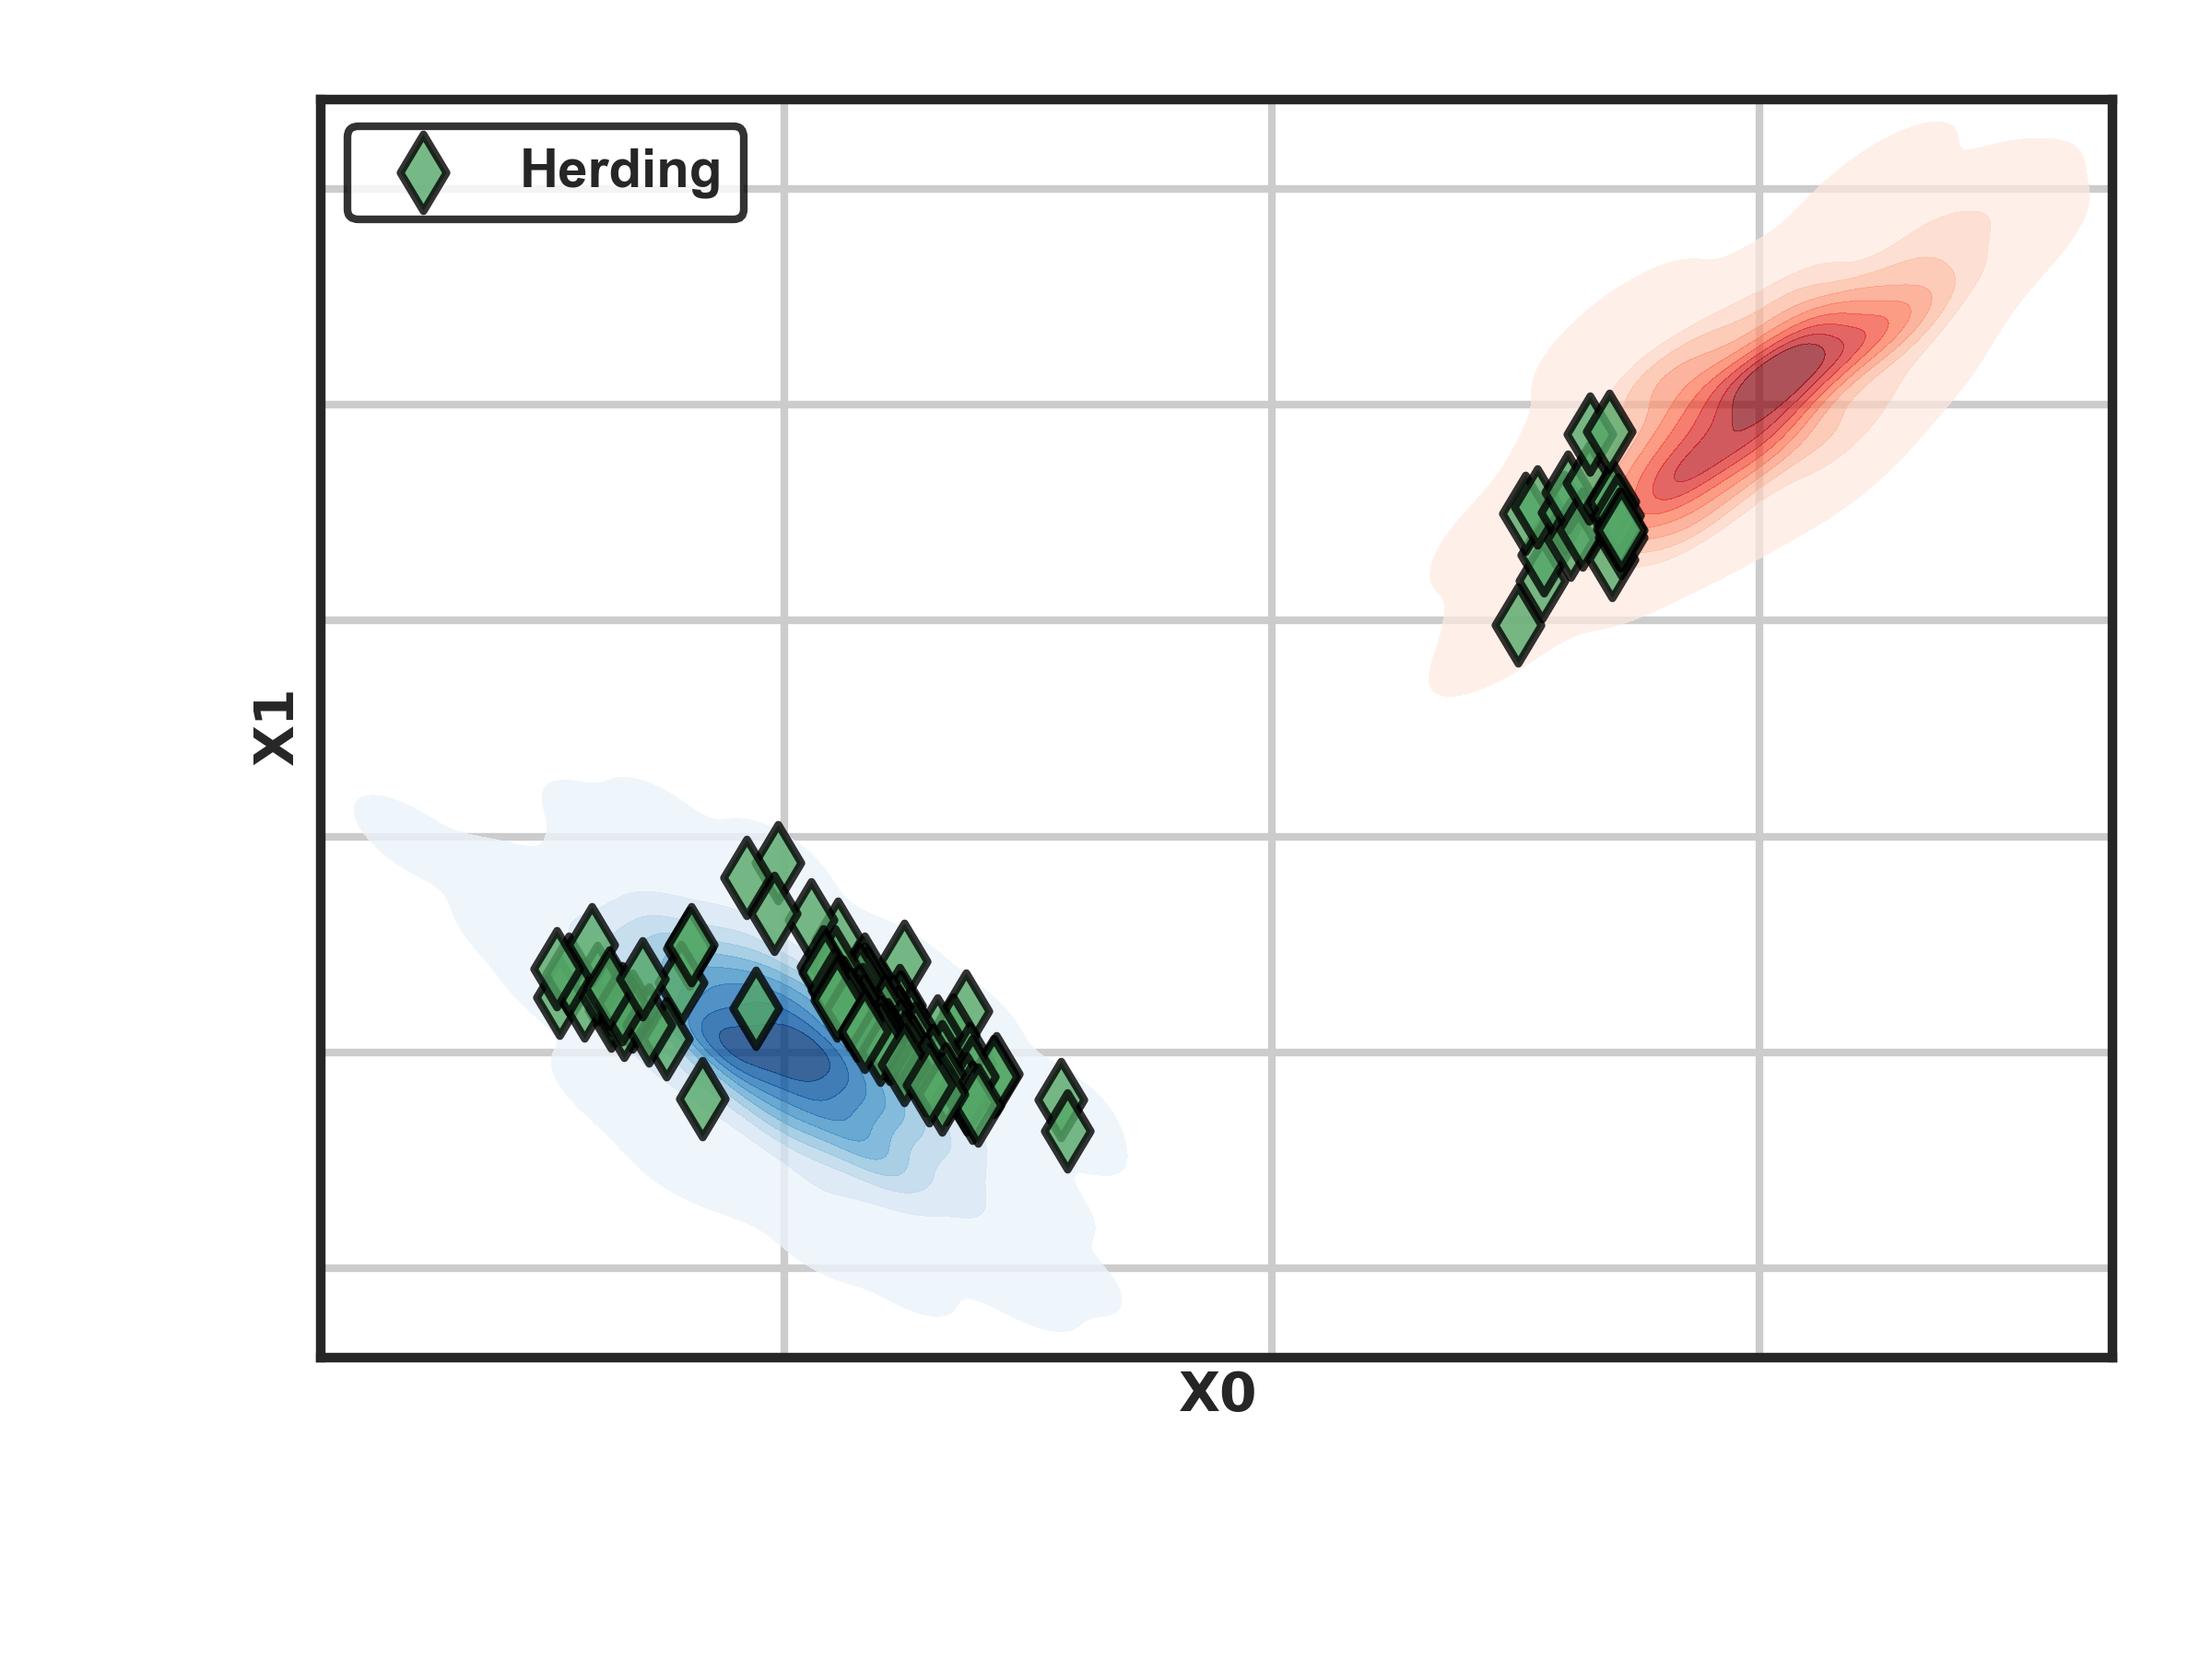}}
\subfloat[$\gm$ \textsc{Matching}]
{\includegraphics[width=0.32\textwidth]{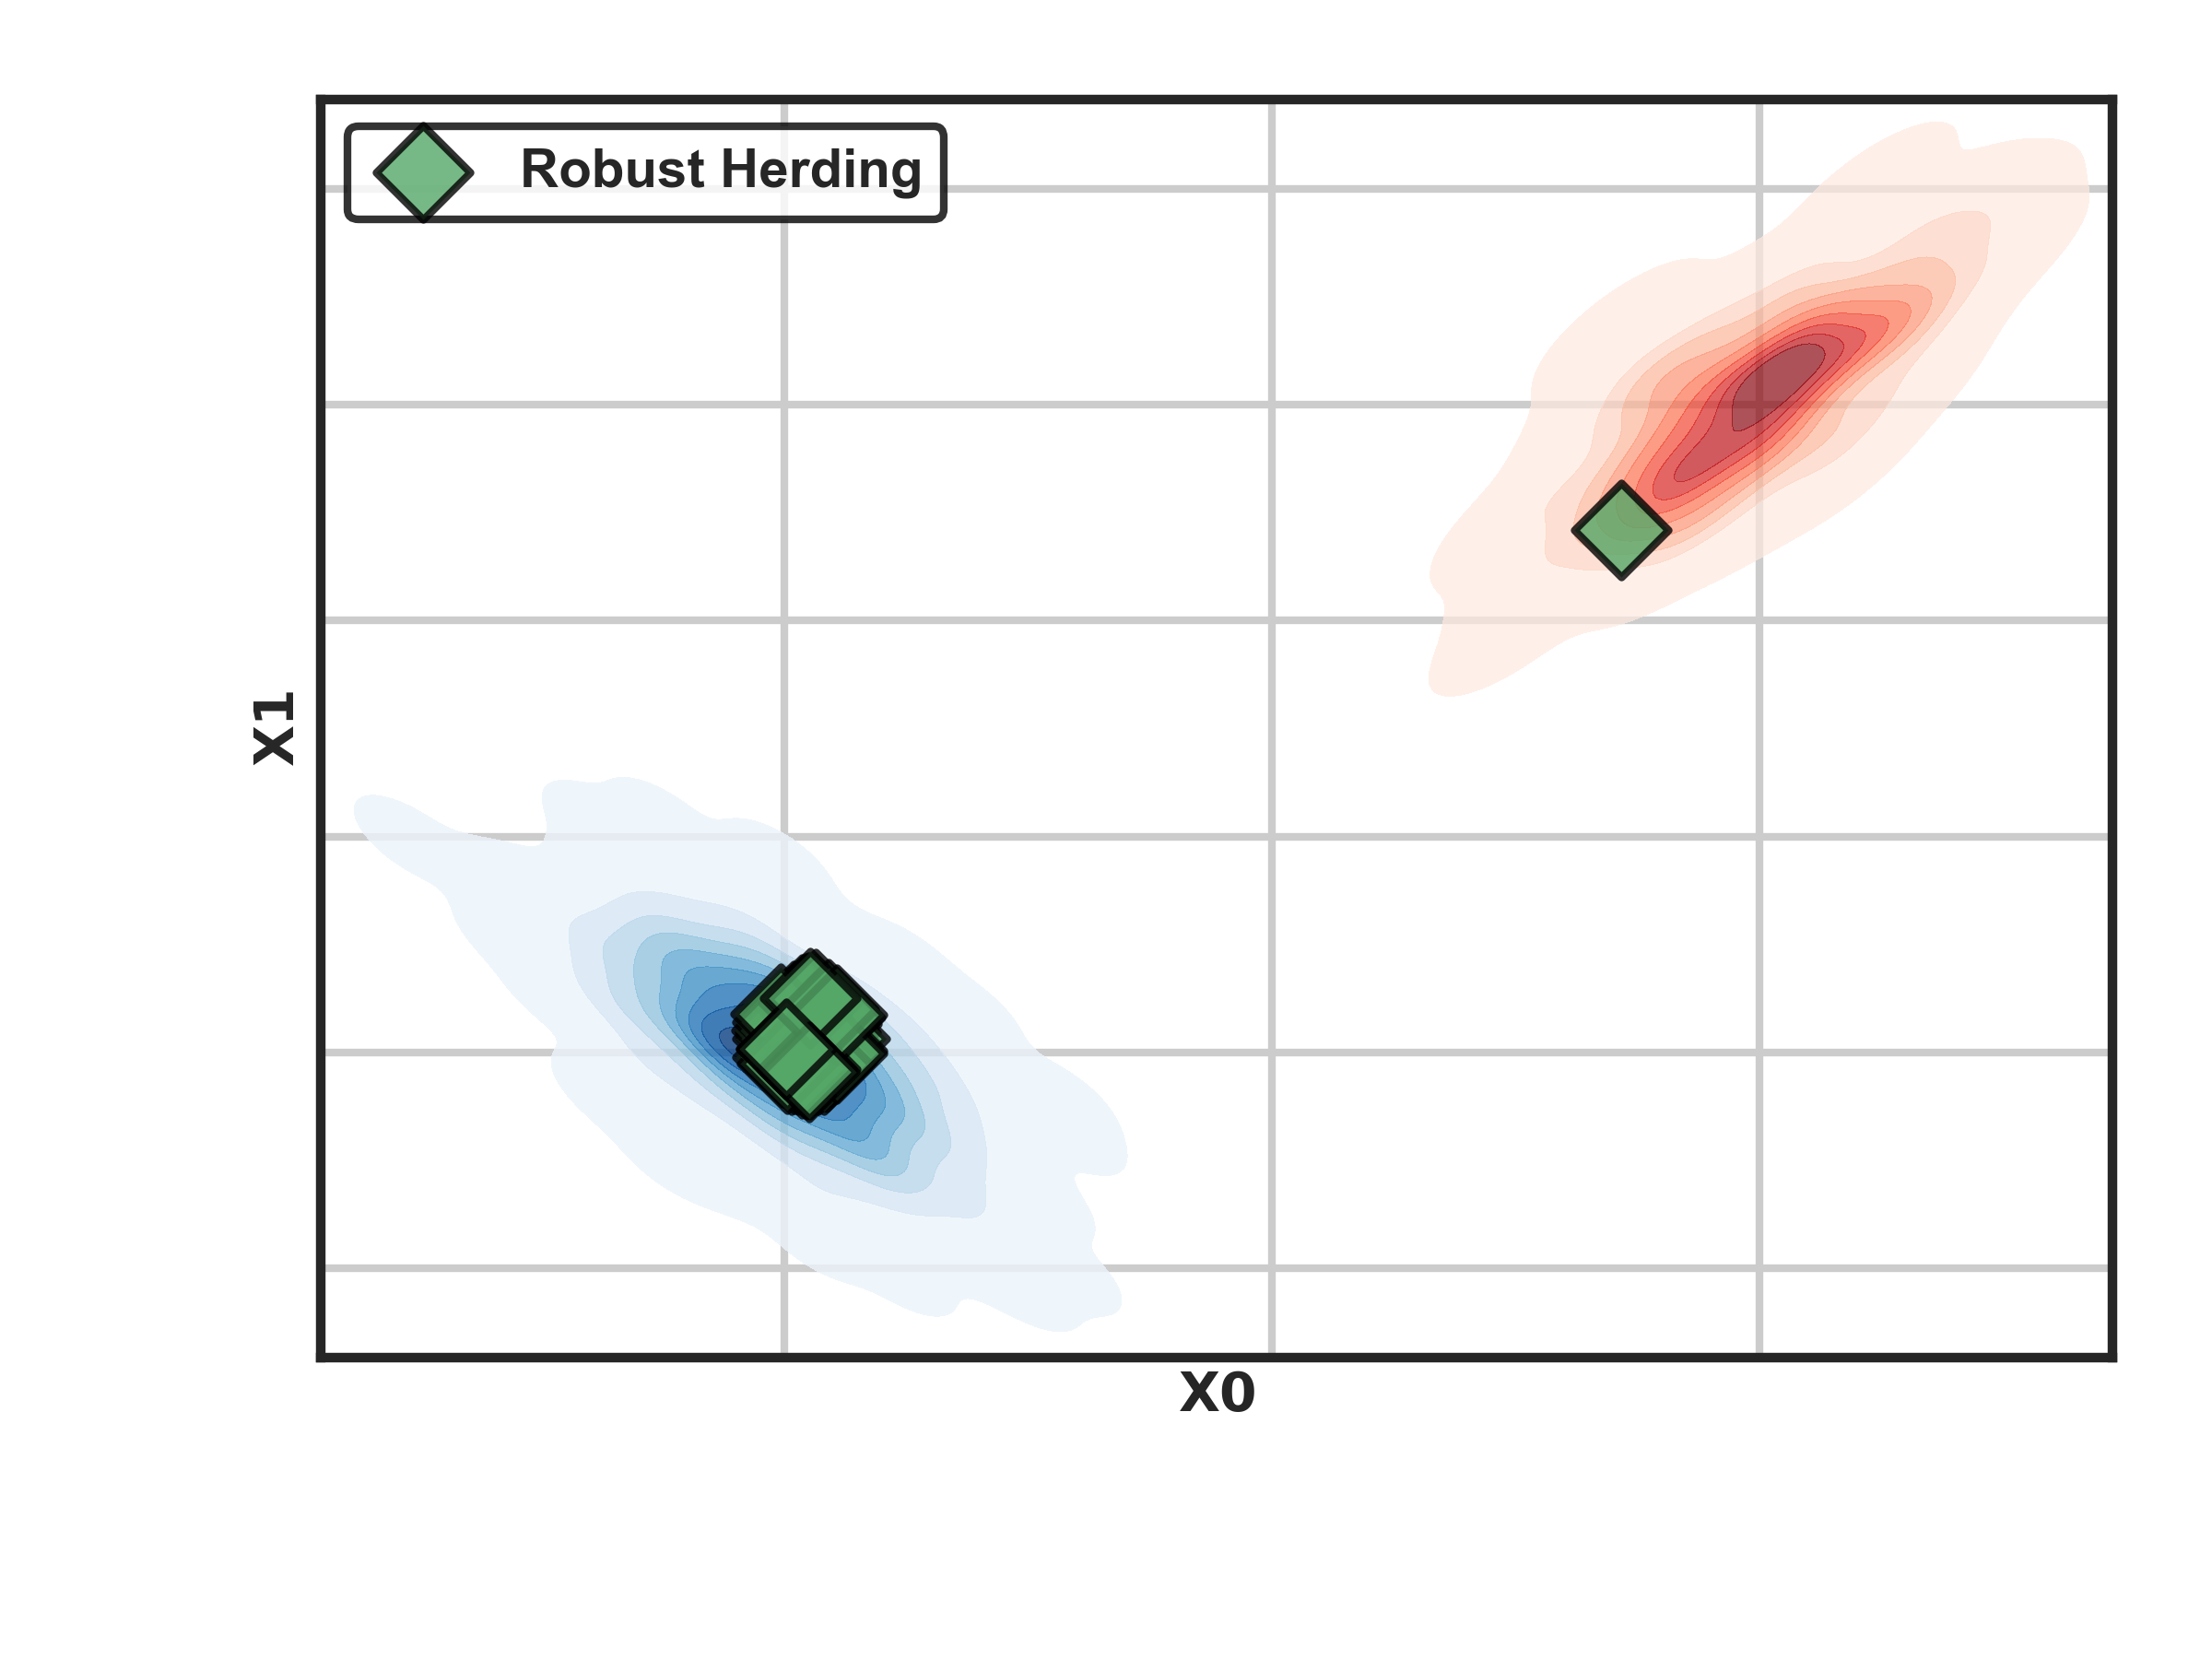}}
\caption{\footnotesize {\bf 20\% Corruption}: In this experiment, 20\% of the samples are corrupted -- drawn from a adversary chosen distribution (red). We select 10\% samples using: (\textsc{Uniform}) Random Sampling, (\textsc{Easy}) Selection of samples closest to the centroid. (\textsc{Hard}) Selection of samples farthest from the centroid. (\textsc{Moderate}) Selection of samples closest to the median distance from the centroid. (\textsc{Herding}) Moment Matching, (\textsc{GM Matching}) Robust Moment (GM) Matching~\eqref{eq:gm_matching}. We see that while \textsc{Easy} remains robust, it is clearly sampling from low-density areas -- failing to capture the prototypical samples.}
\label{fig:toy-corr=20}
\end{figure*}
\begin{figure*}[t] 
\centering
\subfloat[\textsc{Uniform}]
{\includegraphics[width=0.32\textwidth]{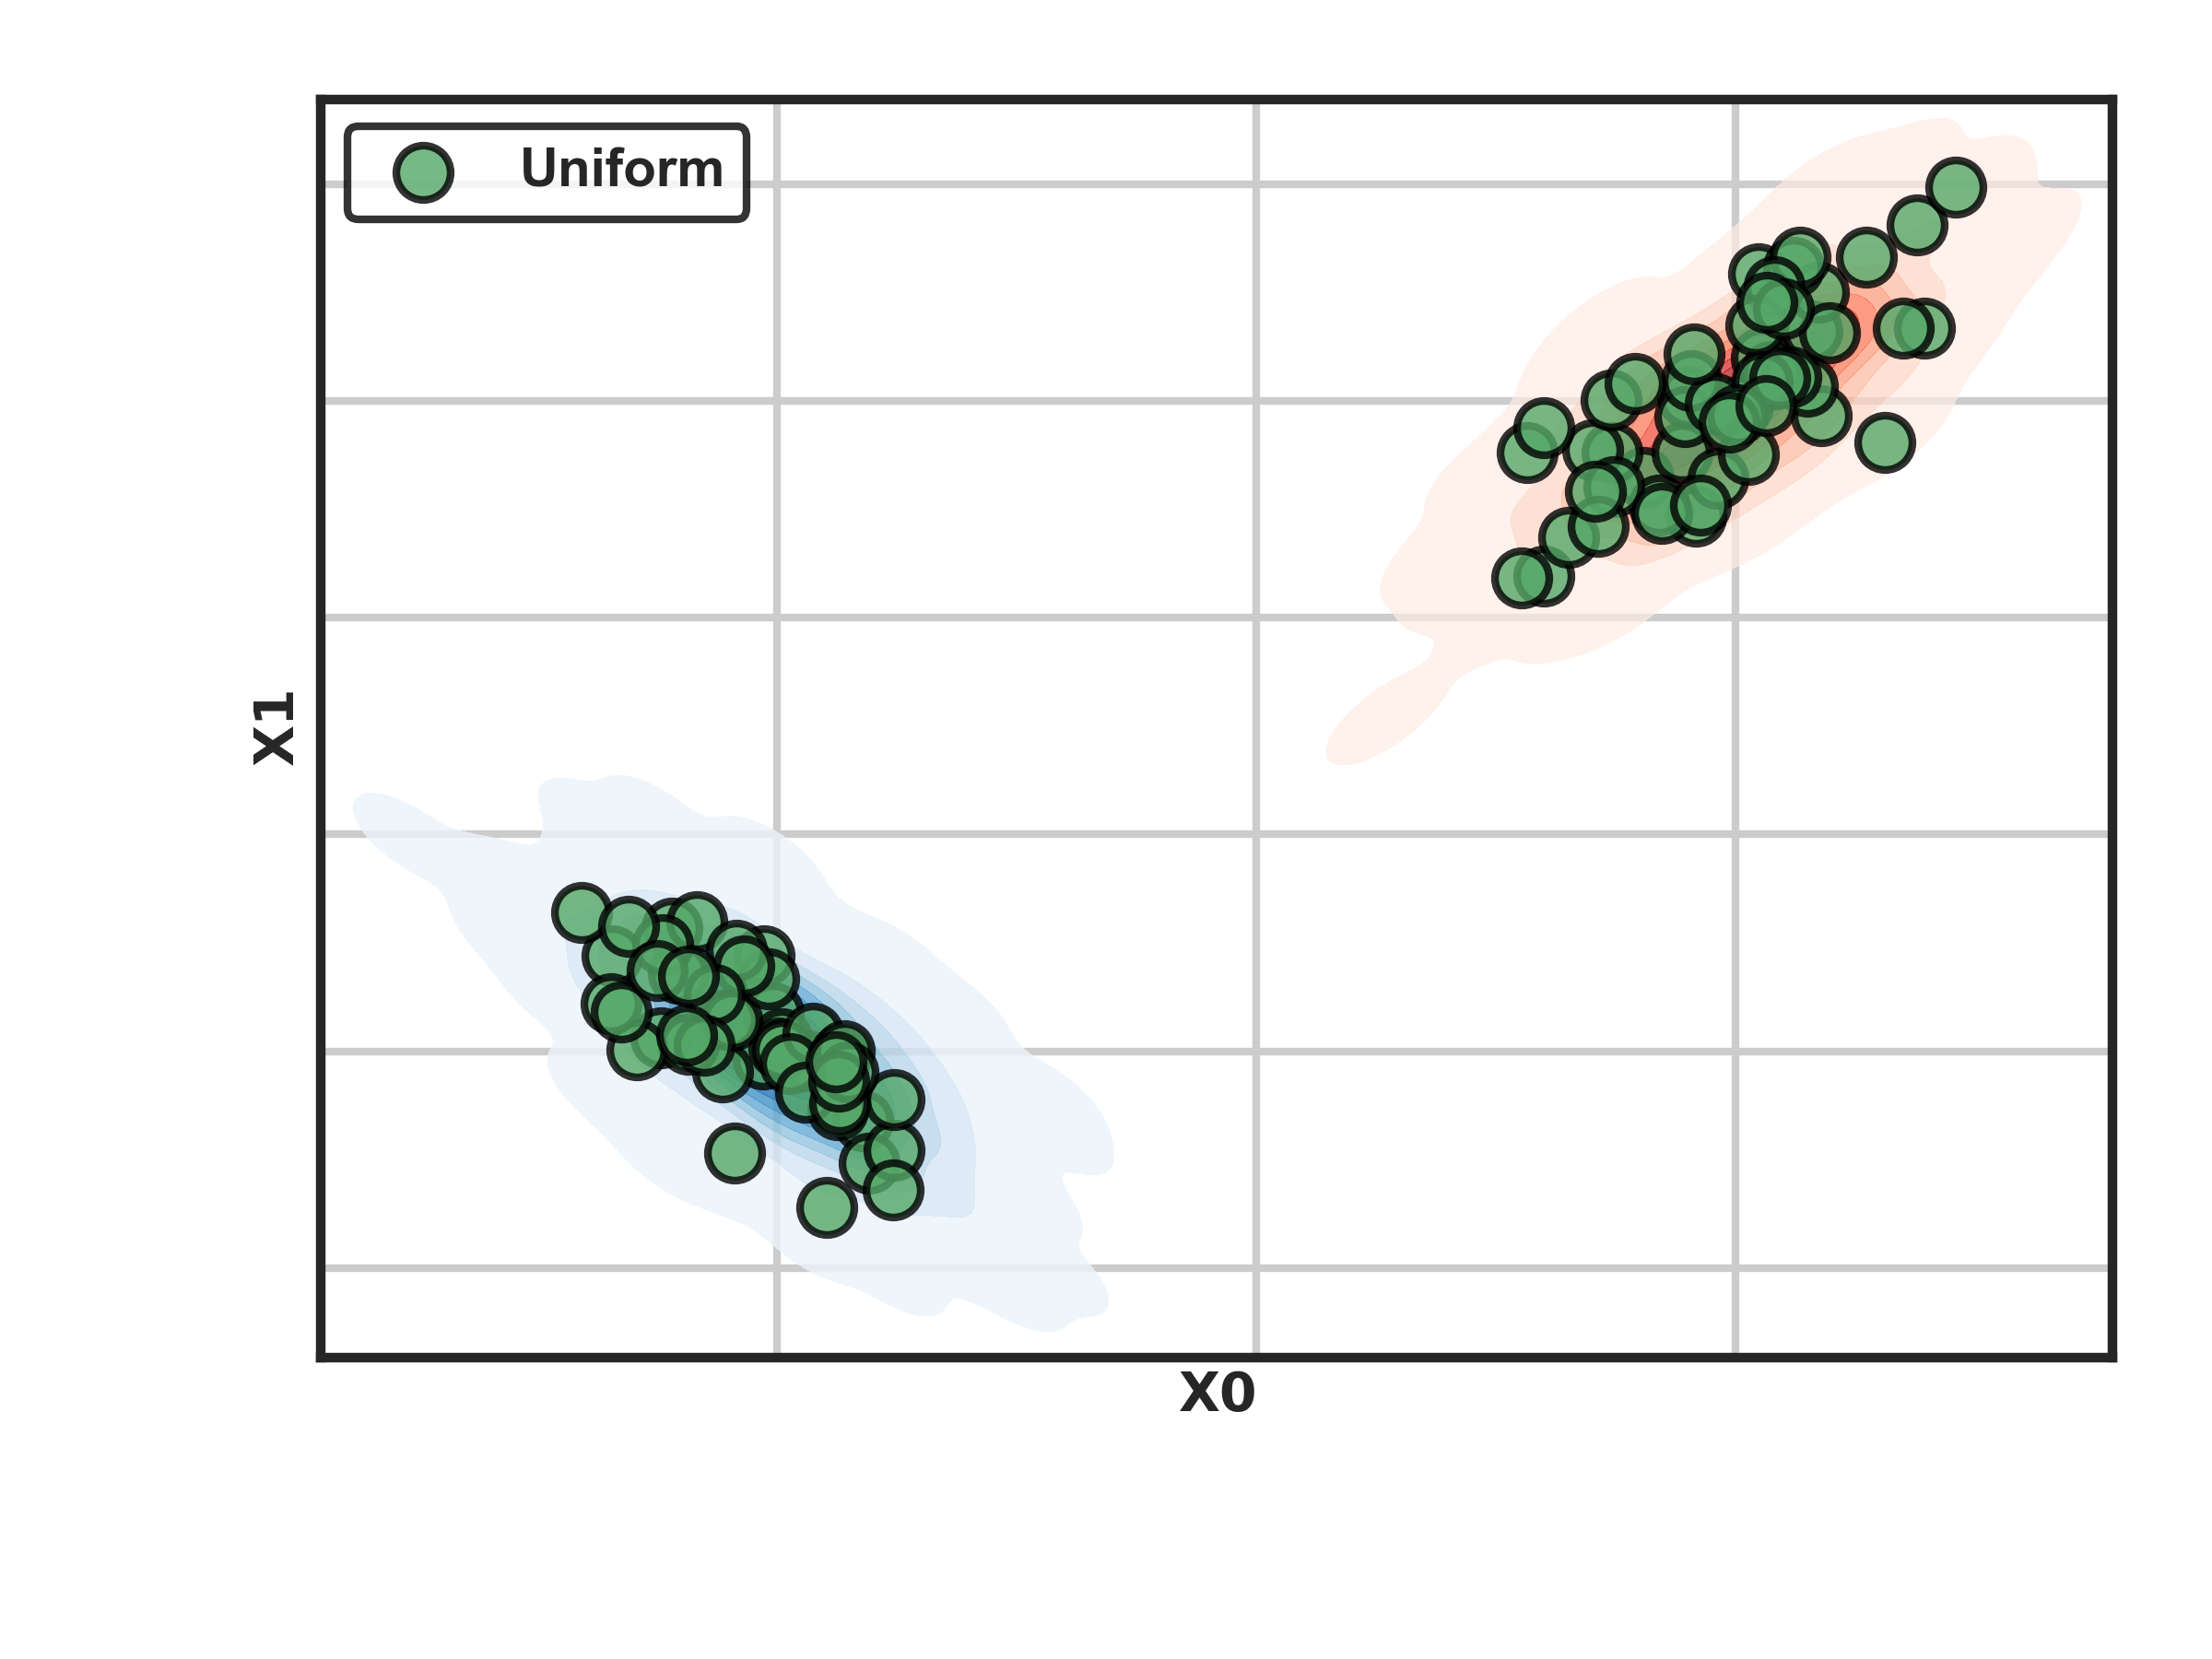}}
\subfloat[\textsc{Easy}]
{\includegraphics[width=0.32\textwidth]{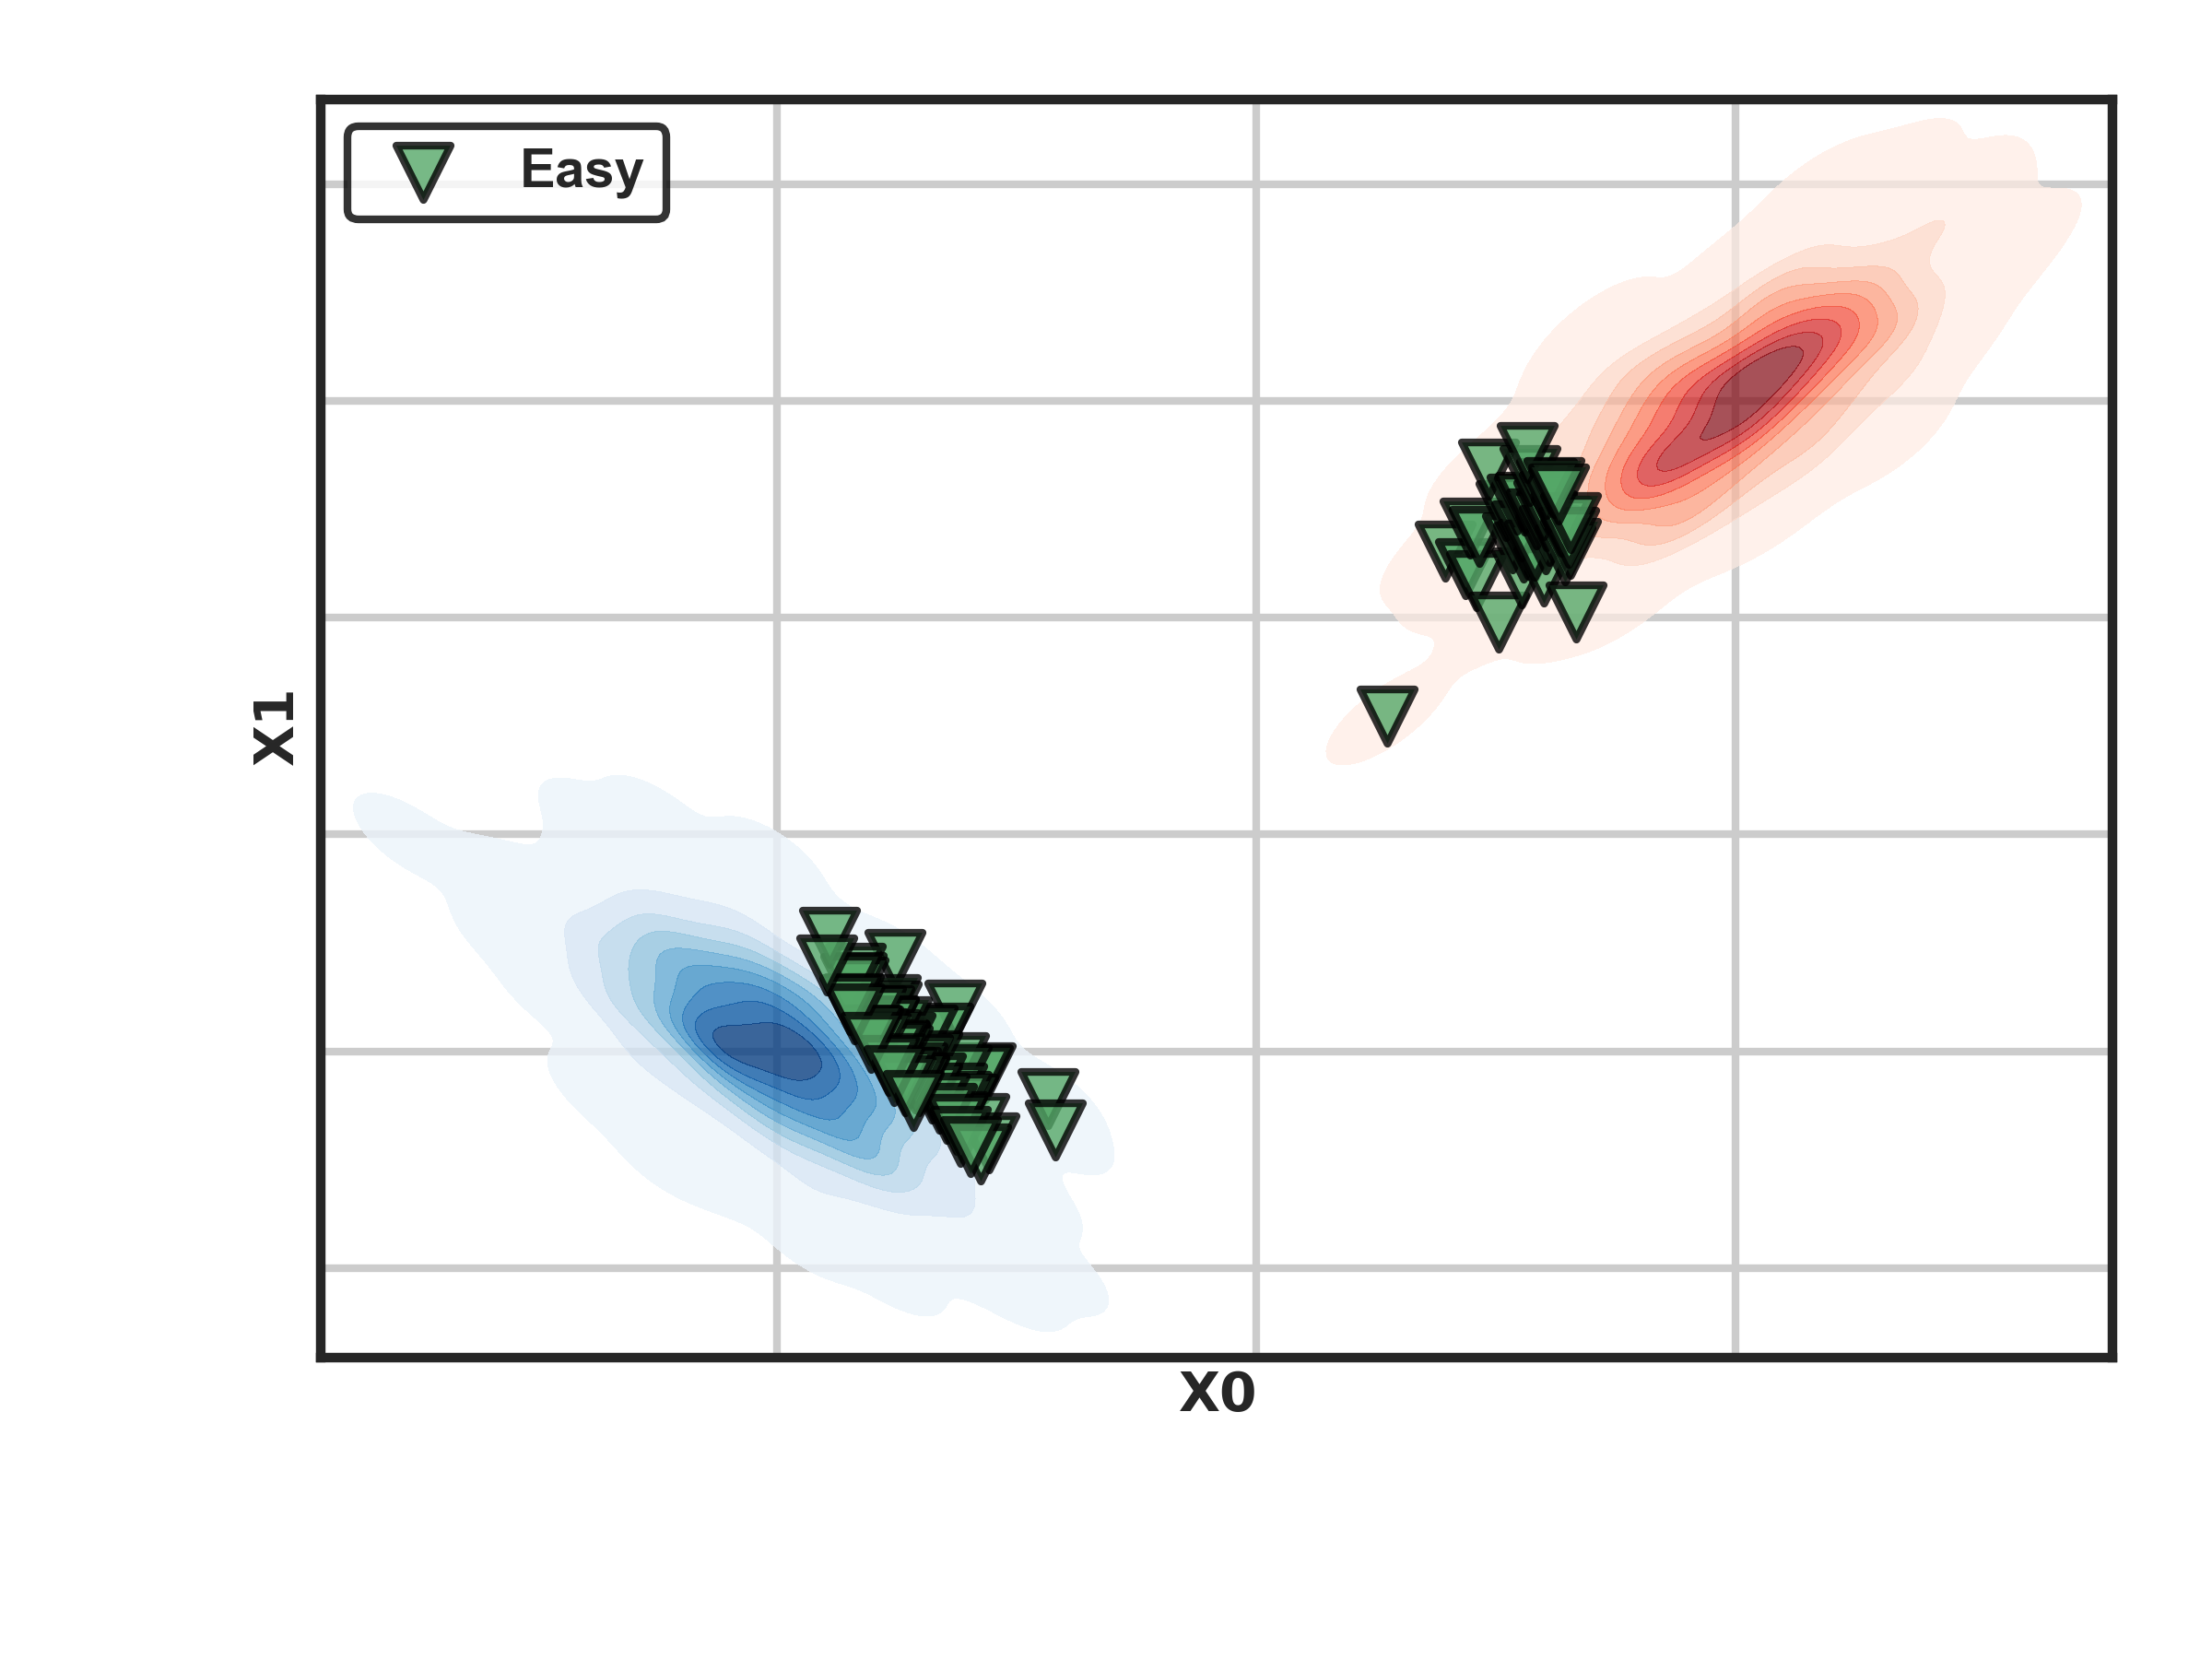}}
\subfloat[\textsc{Hard}]
{\includegraphics[width=0.32\textwidth]{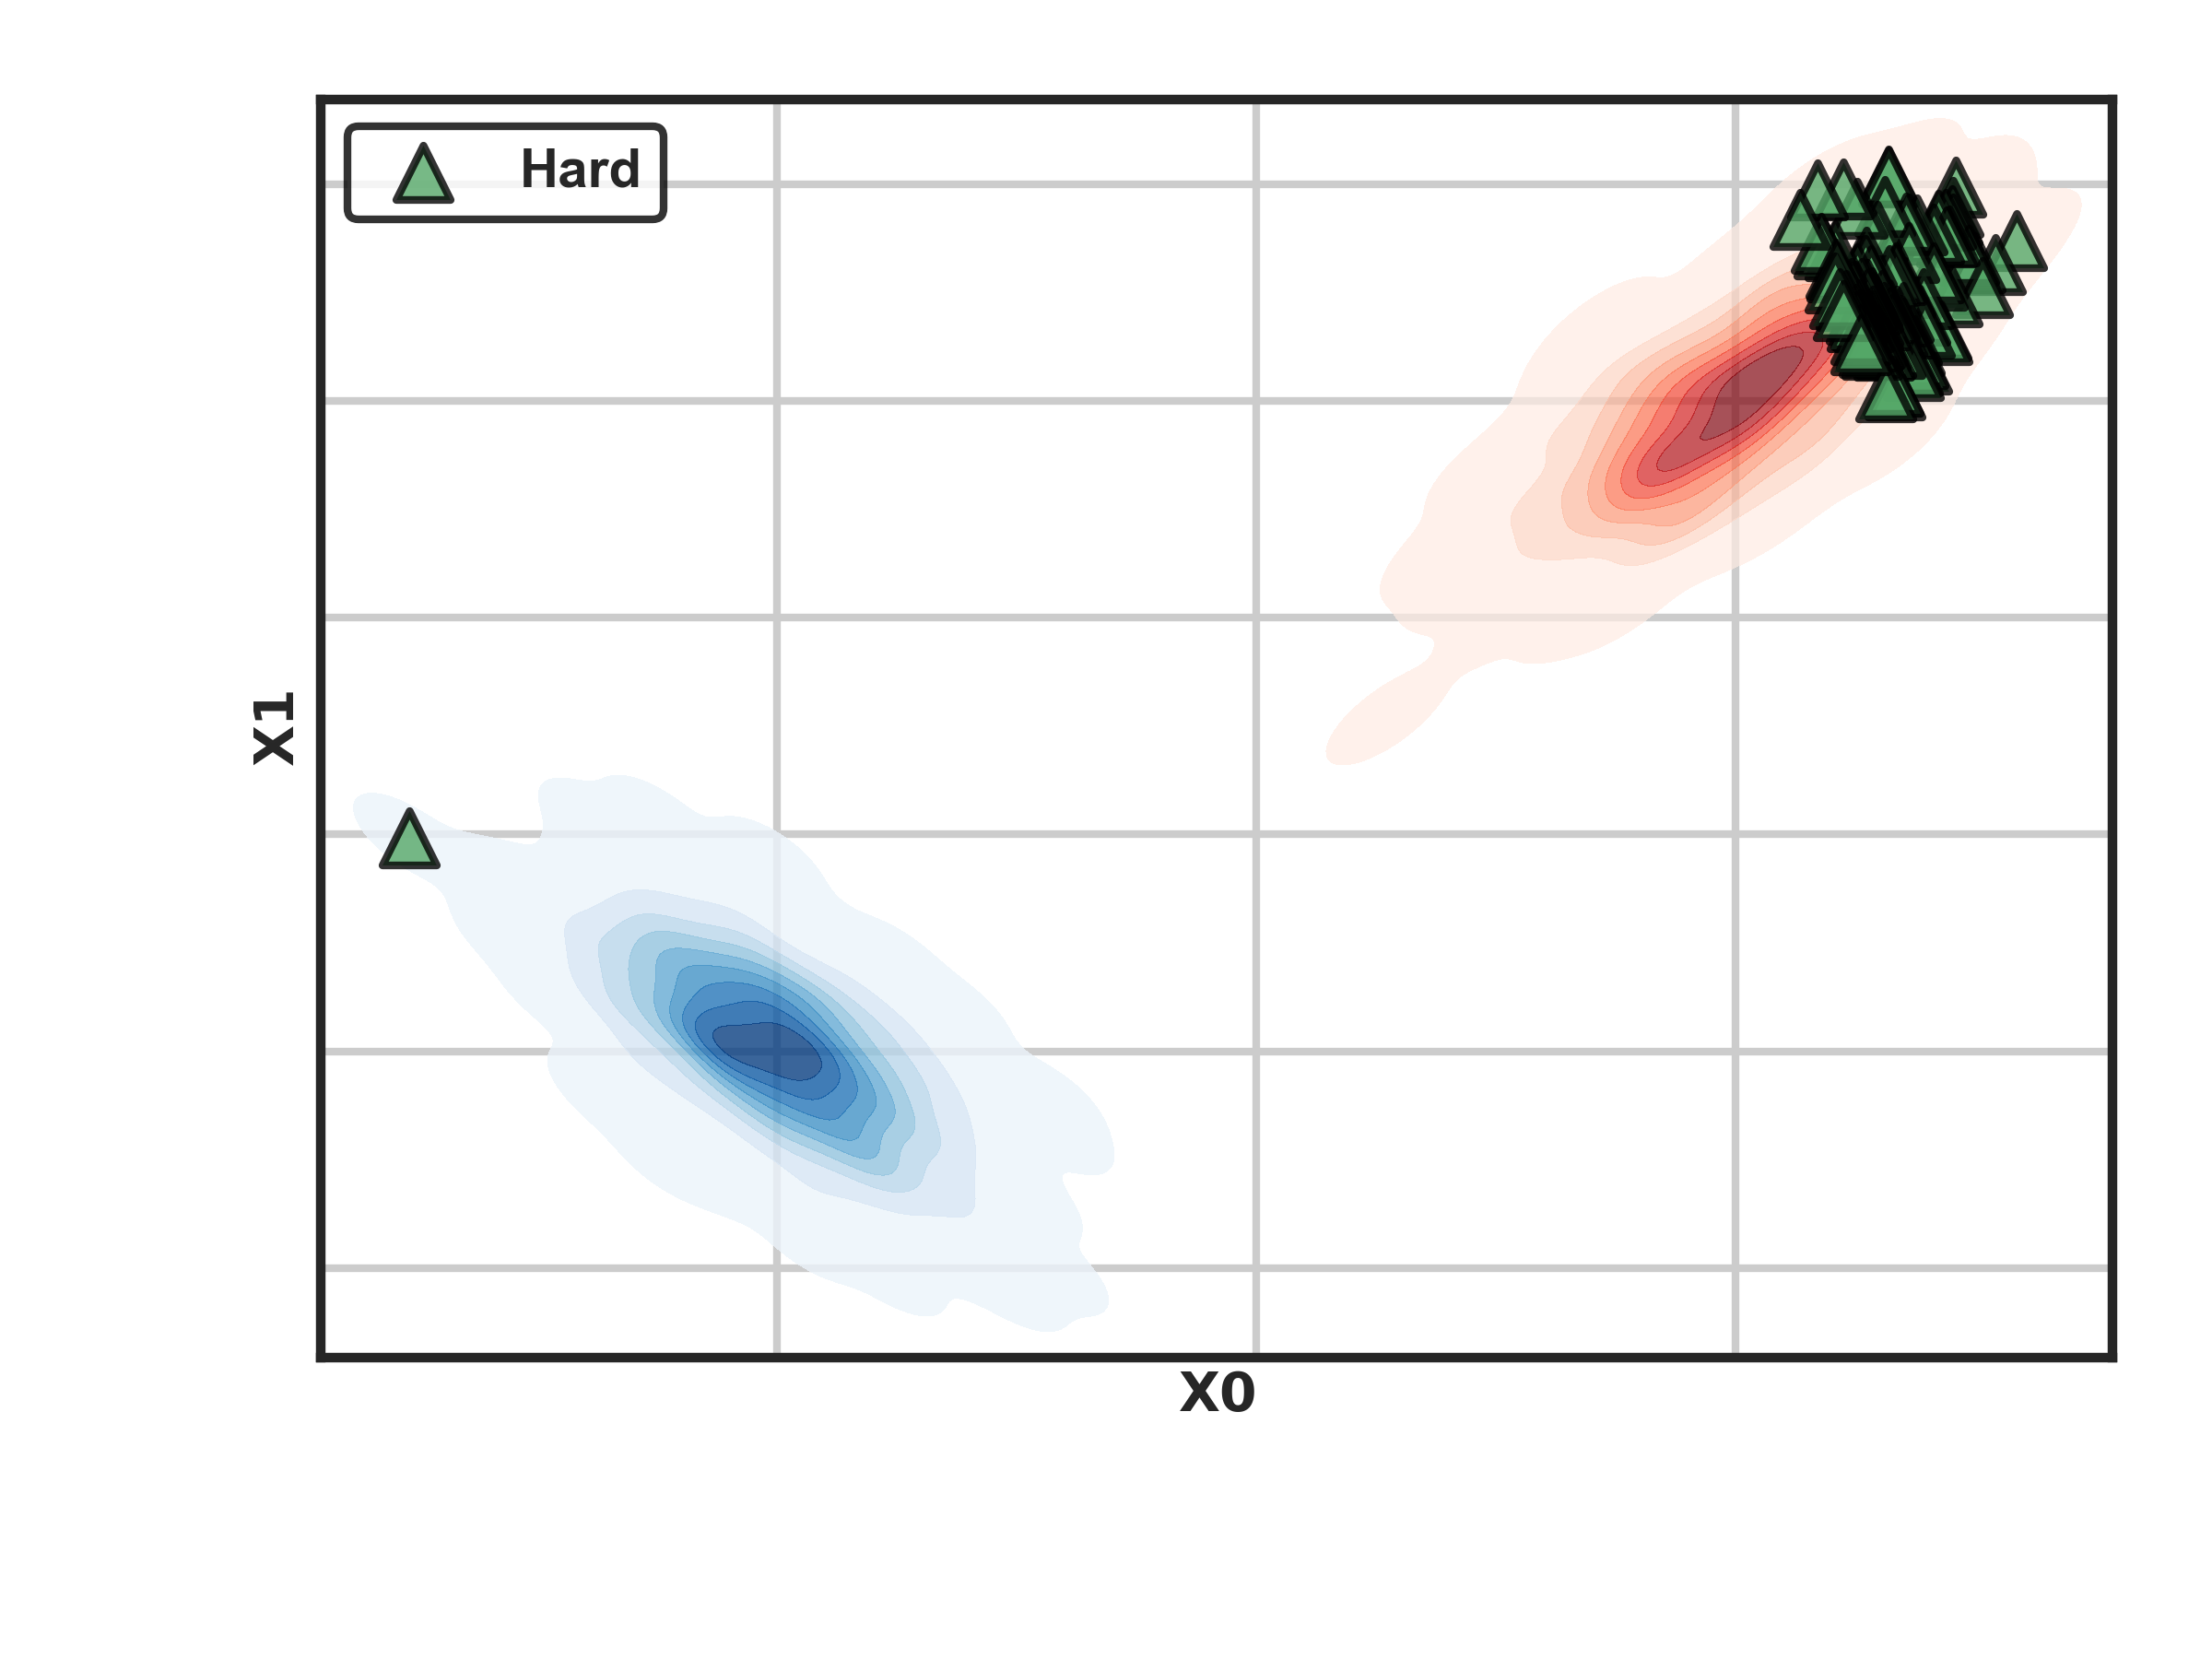}}
\\
\subfloat[\textsc{Moderate}]
{\includegraphics[width=0.32\textwidth]{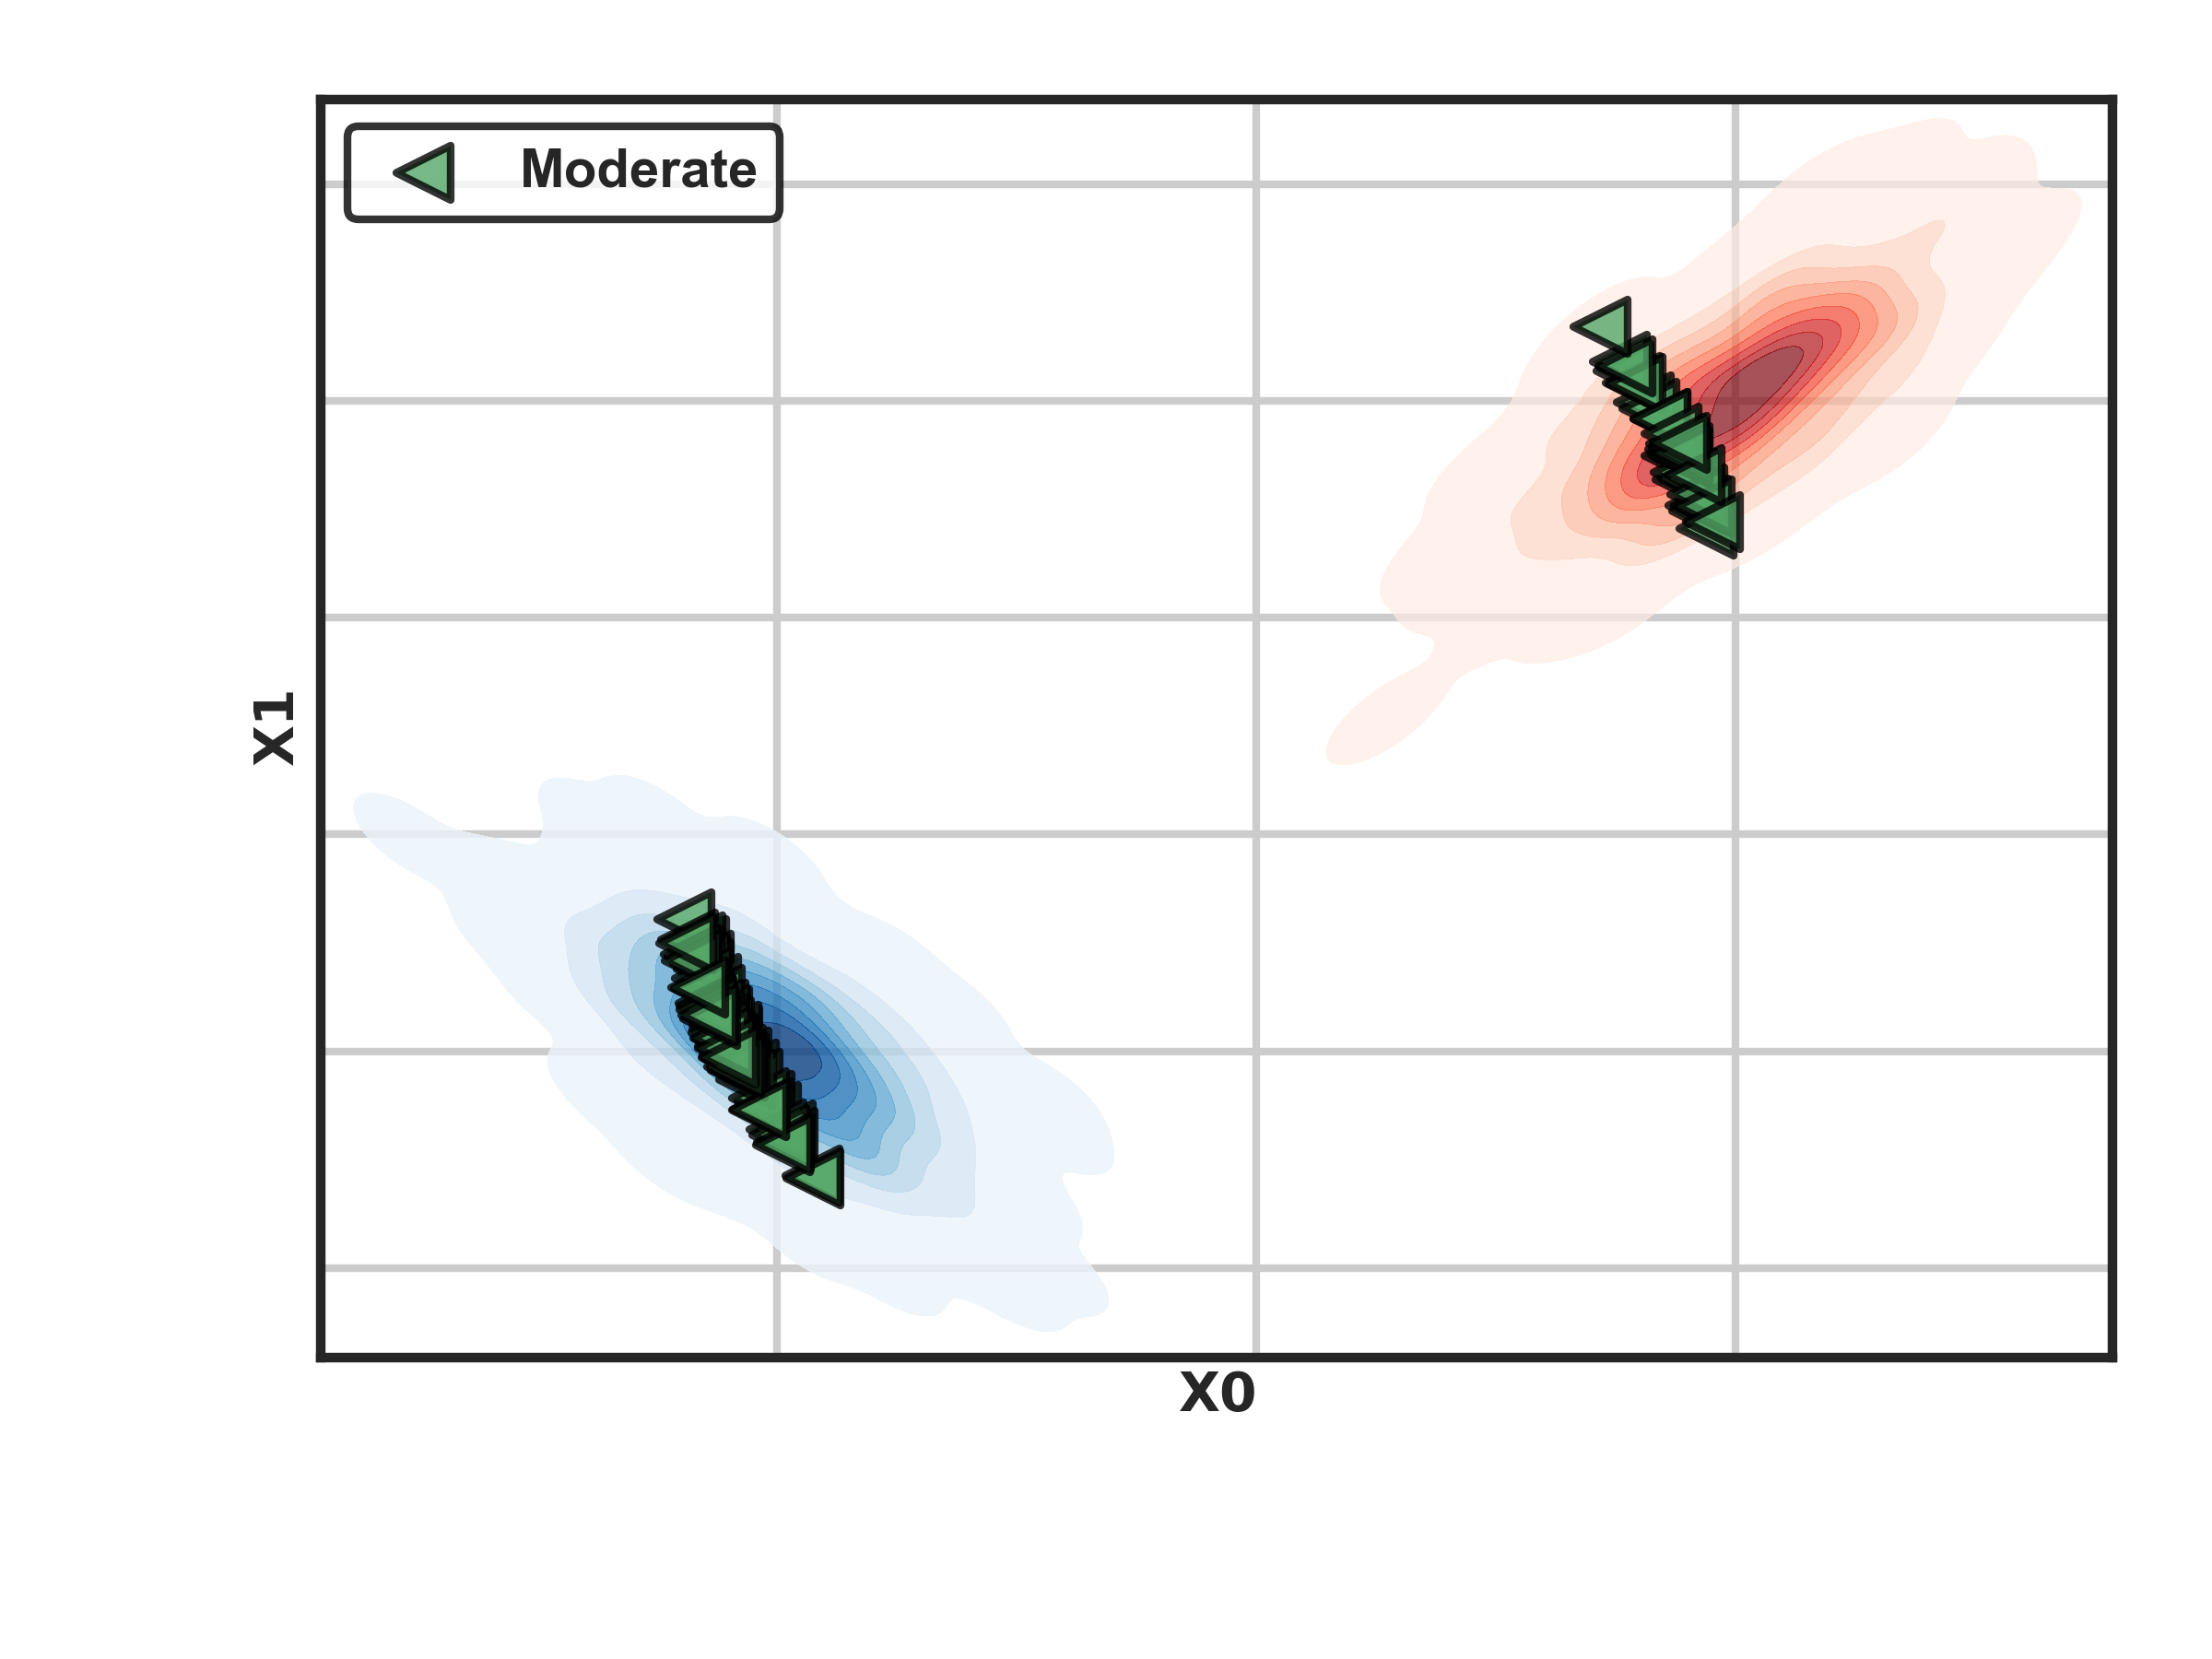}}
\subfloat[\textsc{Herding}]
{\includegraphics[width=0.32\textwidth]{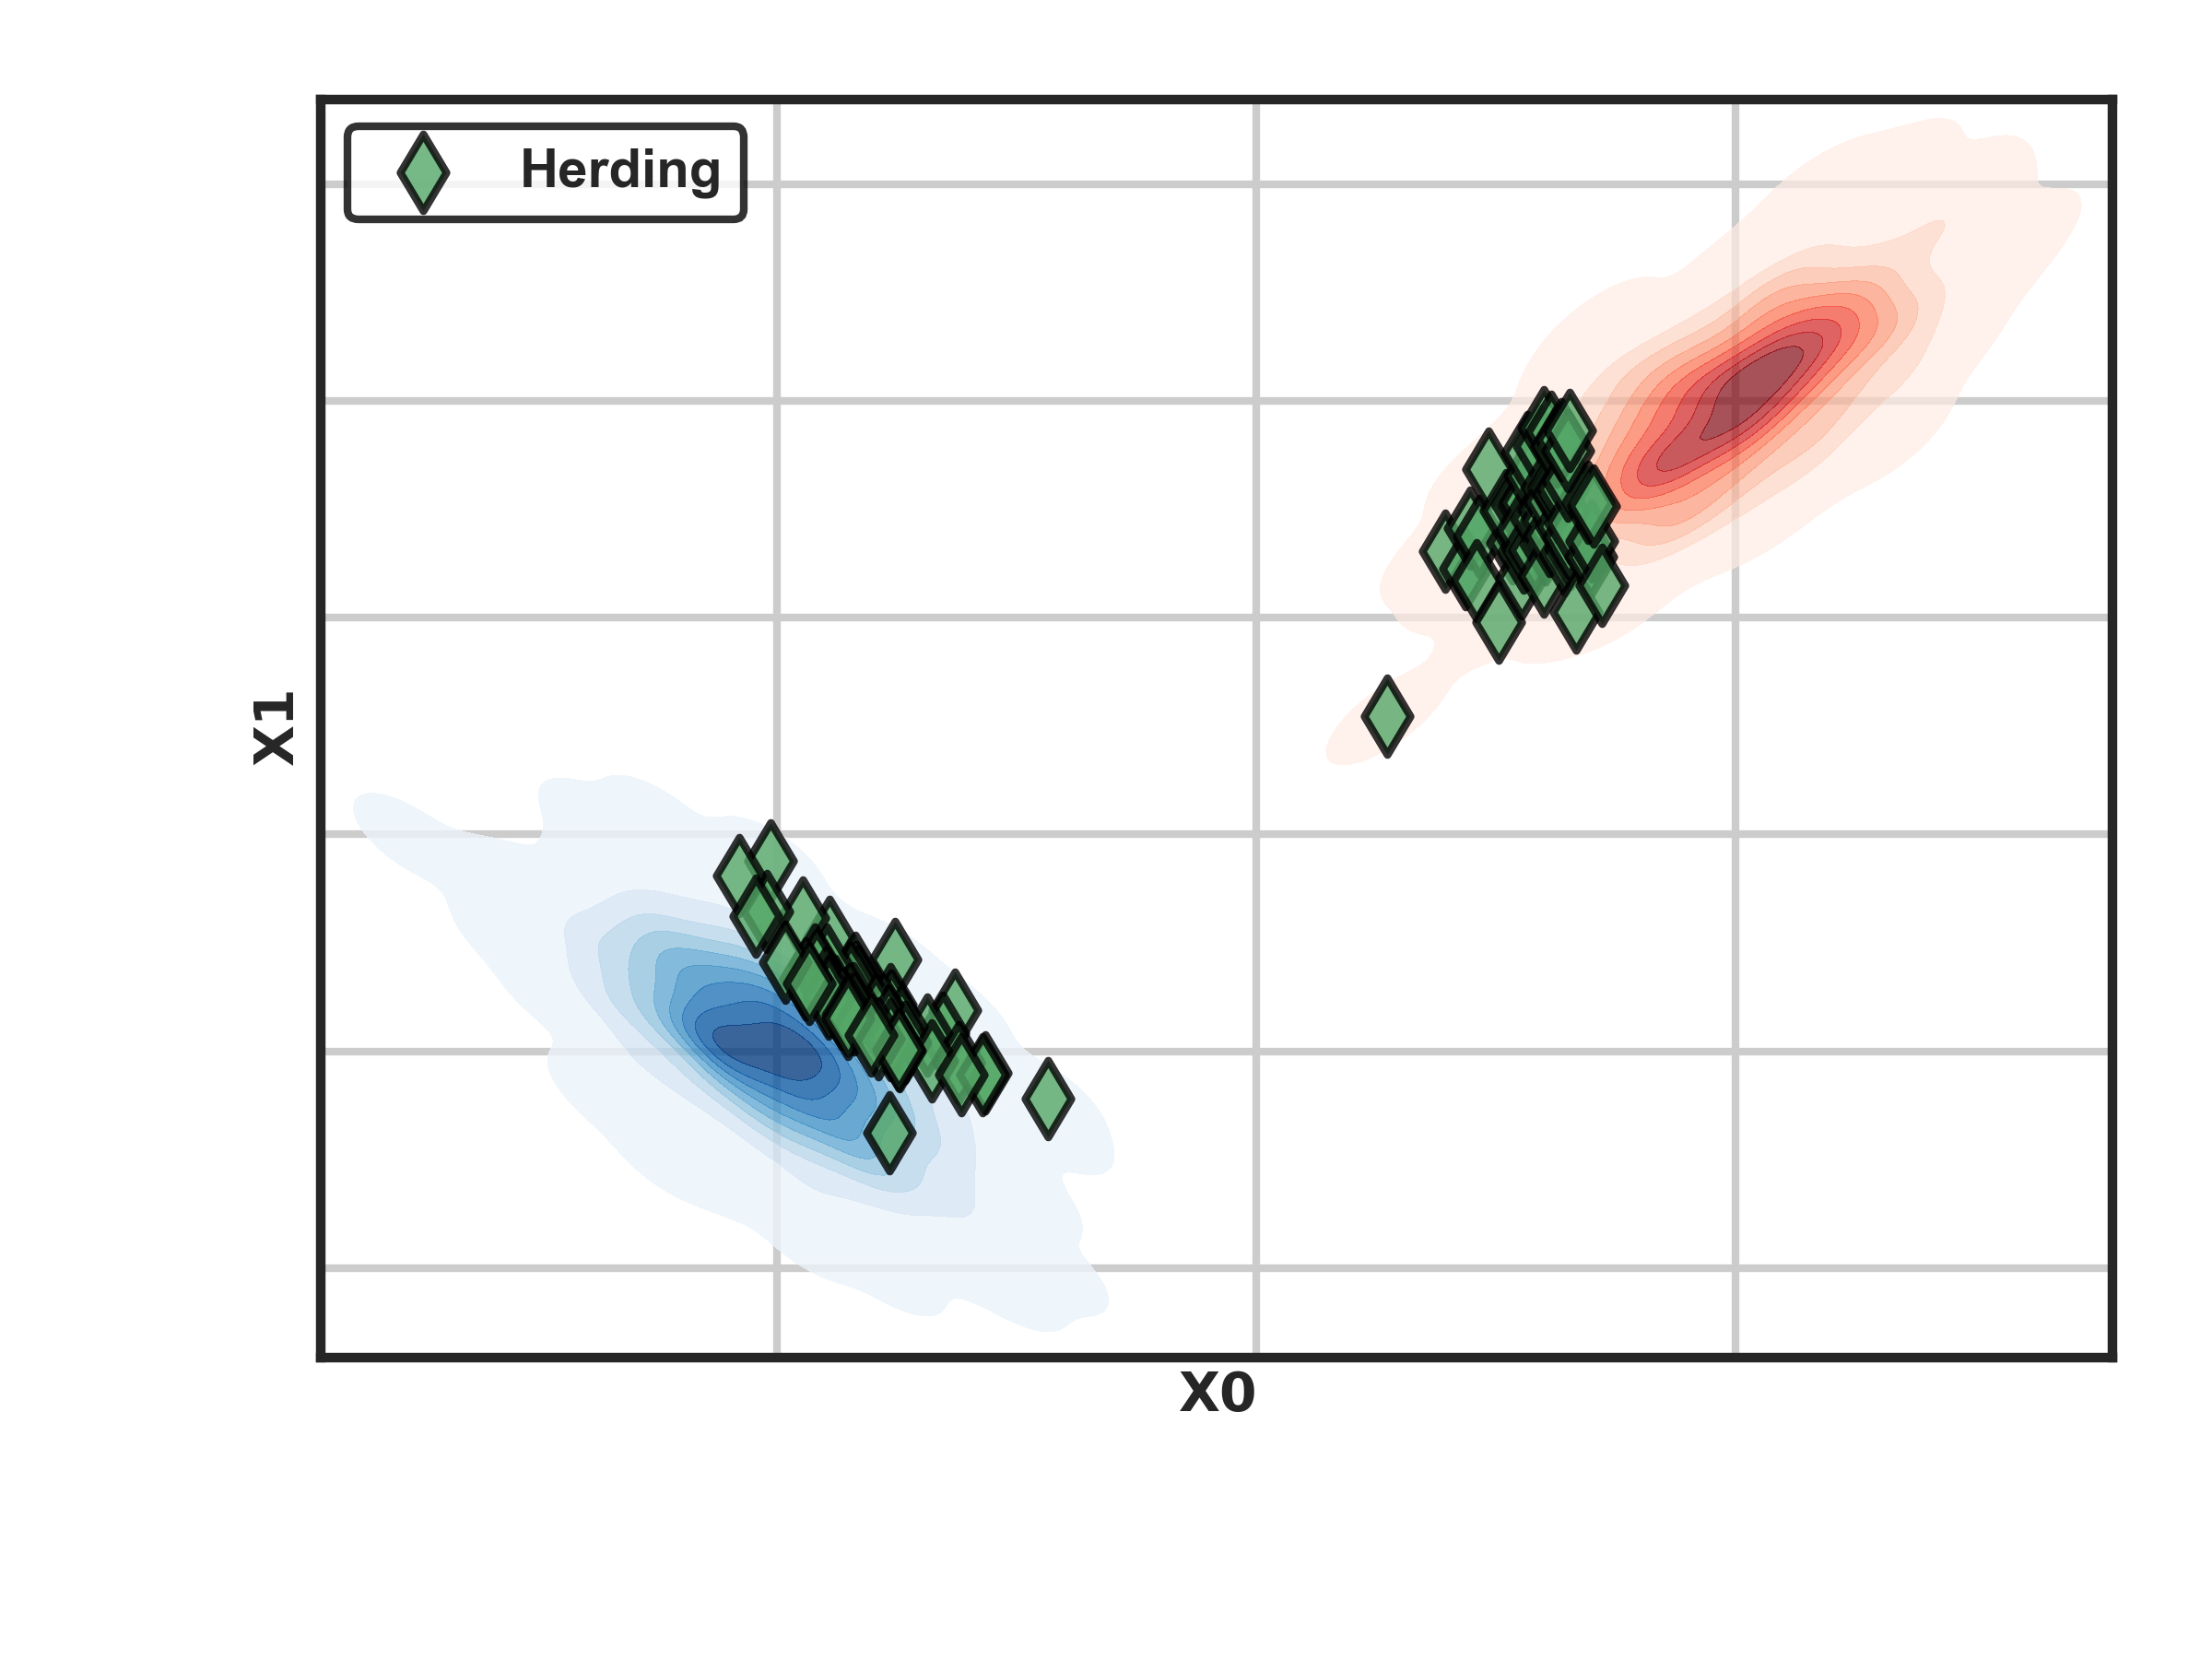}}
\subfloat[$\gm$ \textsc{Matching}]
{\includegraphics[width=0.32\textwidth]{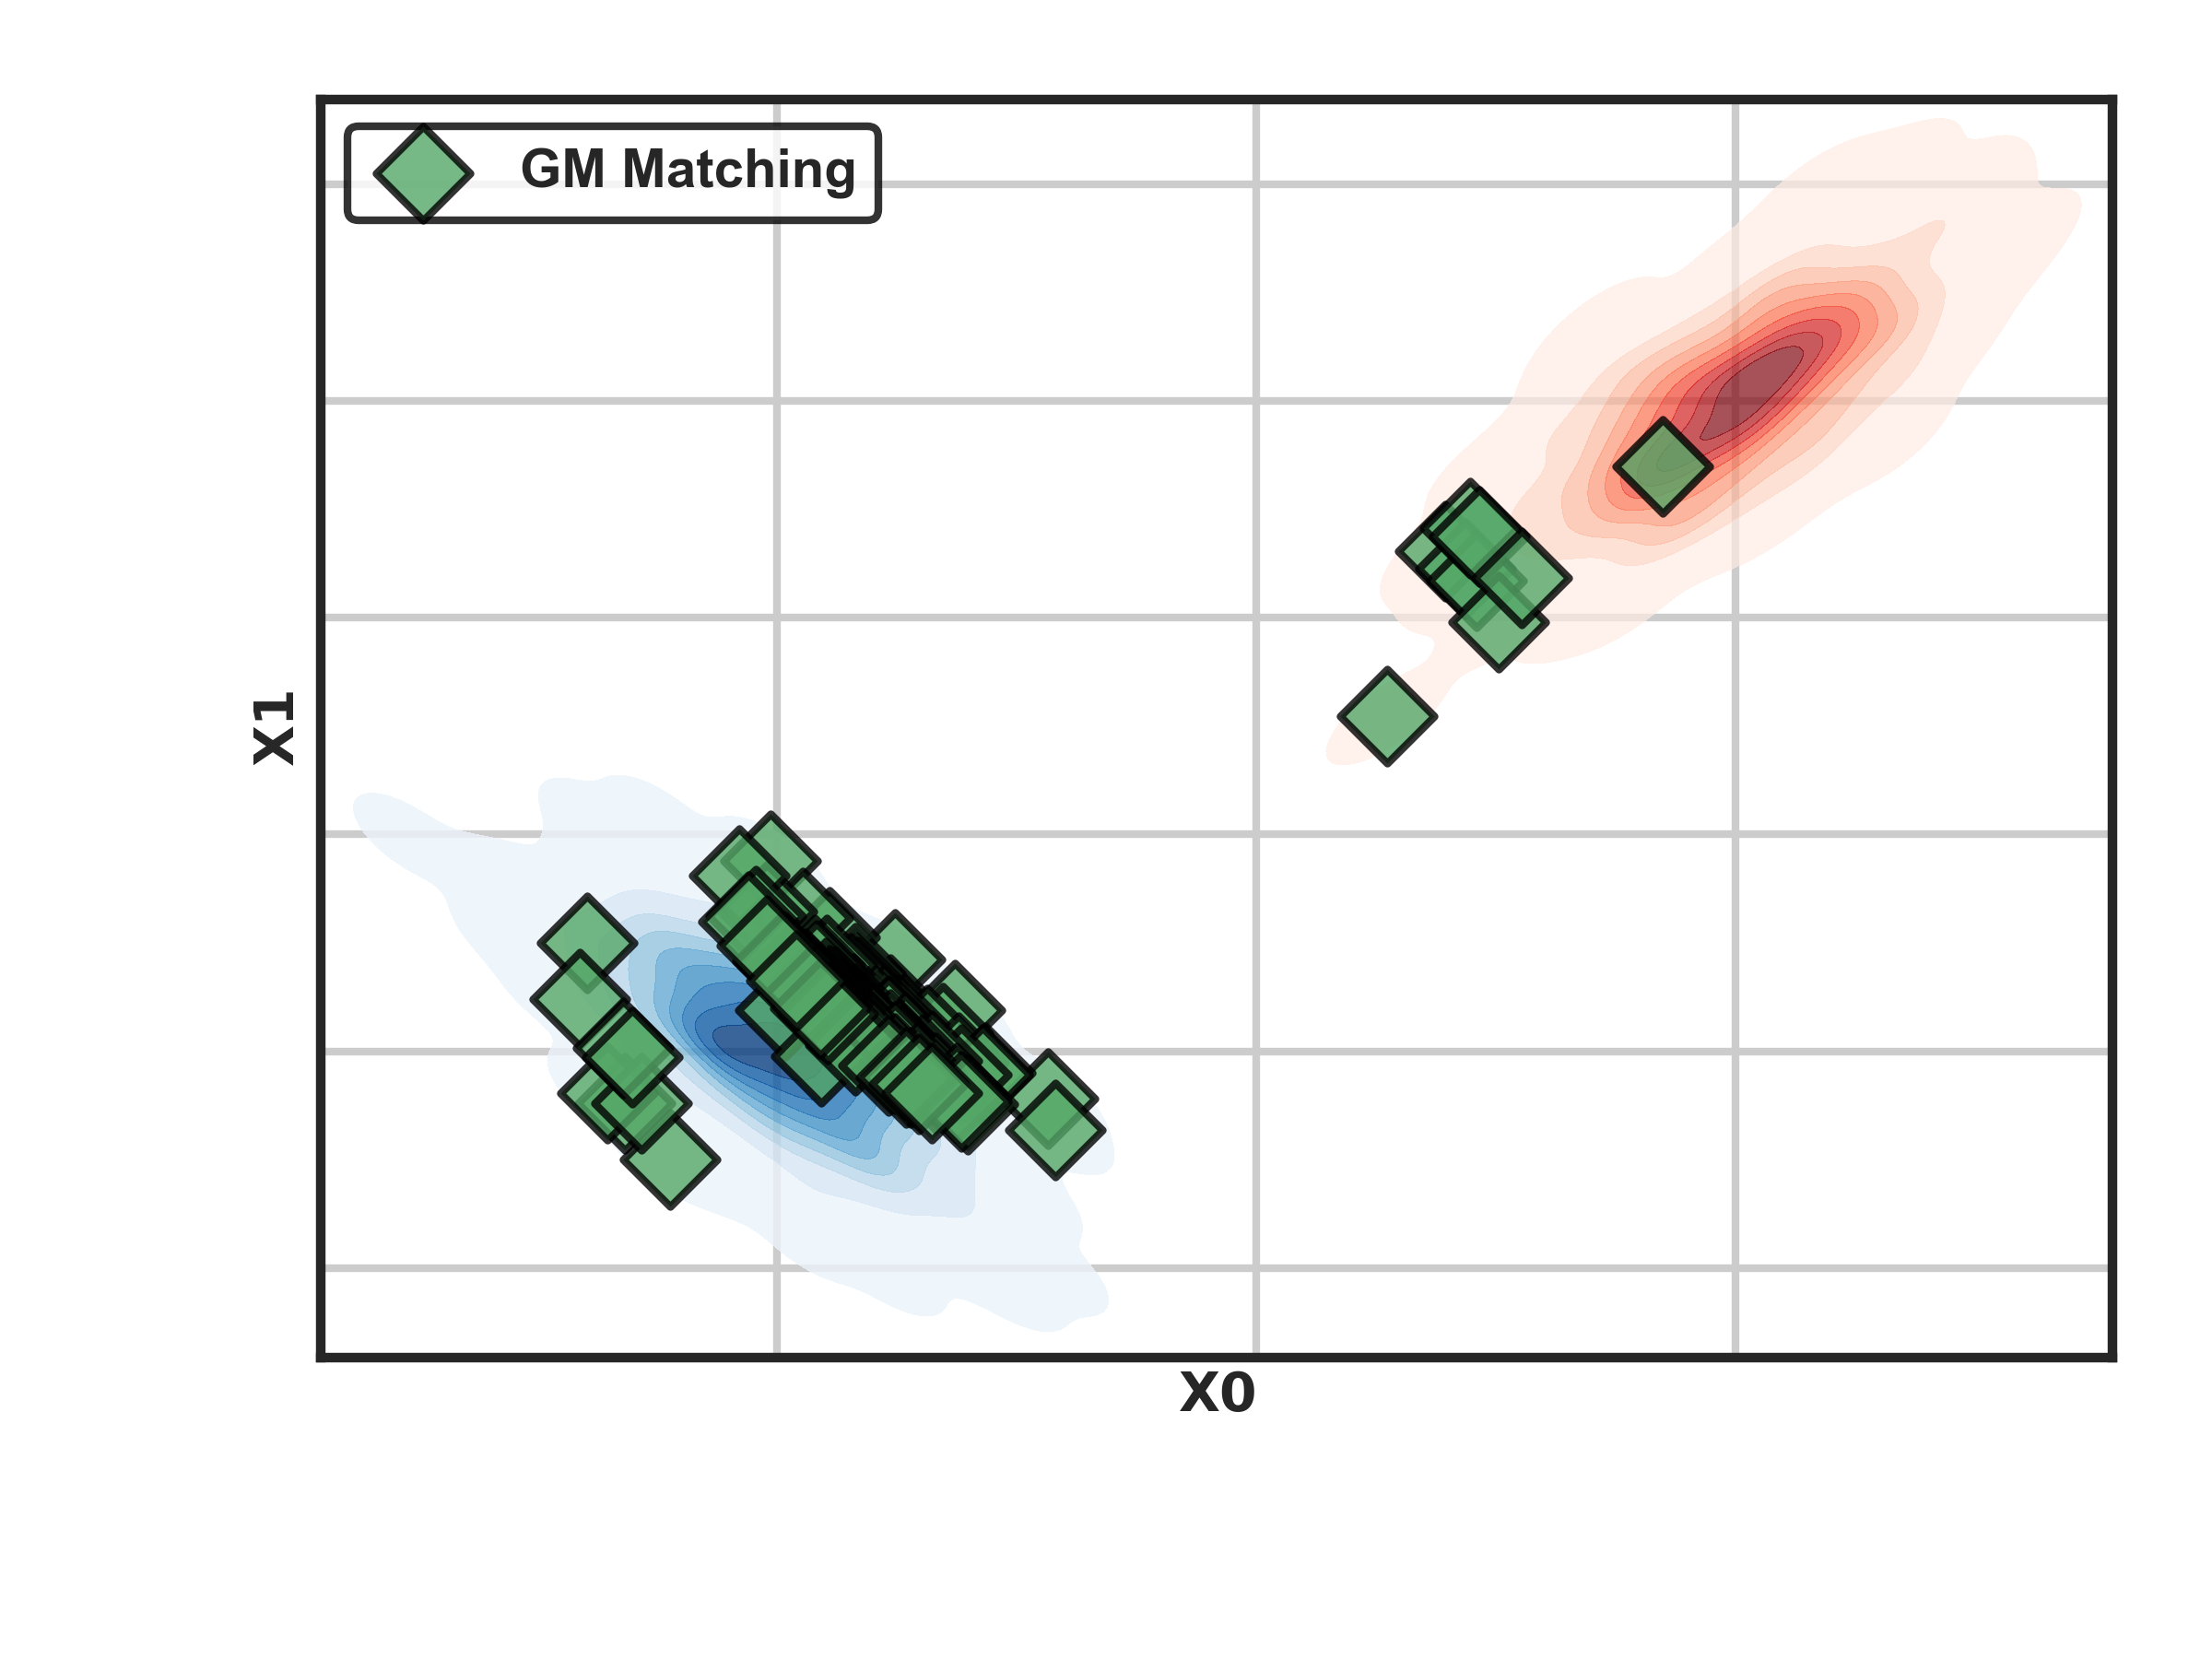}}
\caption{\footnotesize {\bf Toy Example:} {\bf 45\% of the samples are corrupted} i.e. drawn from an adversary chosen distribution (red). We compare several baselines for choosing 10\% samples: (\textsc{Uniform}) random sampling, (\textsc{Easy}) selects of samples closest to the centroid. (\textsc{Hard}) Selection of samples farthest from the centroid. (\textsc{Moderate}) selects samples closest to the median distance from the centroid. (\textsc{Herding}) moment matching, (\textsc{GM Matching}) robust moment (GM) matching~\eqref{eq:gm_matching}. Clearly $\gm$ Matching is significantly more robust and diverse than the other approaches even at such high corruption rates.}

\label{fig:toy-corr=45}
\end{figure*}

\clearpage
\subsection{Additional Benchmark Experiments}
We share additional results on benchmark datasets that was omitted from the main paper due to space constraint.~\cref{tab:cifarC}-\ref{tab:VGG-Shuffle}.

\input{NeuRips-2024/tables/tab-cifarC}
\input{NeuRips-2024/tables/tab-tinyC}

\input{NeuRips-2024/tables/tab-noisy}
\begin{table*}
    \footnotesize
    \centering
    \begin{tabular}{lccccc}
        \toprule
        
        & \multicolumn{2}{c}{\bf CIFAR-100 (Label noise)} 
        & \multicolumn{2}{c}{\bf Tiny ImageNet (Label noise)} 
        & \\
        \cmidrule(r){2-3} 
        \cmidrule(r){4-5} 
        {\bf Method / Ratio } 
        & 20\% 
        & 30\% 
        & 20\% 
        & 30\% 
        & {\bf Mean $\uparrow$} 
        \\
        \midrule
        Random 
        & 24.51$\pm$1.34 
        & 32.26$\pm$0.81 
        & 14.64$\pm$0.29 
        & 19.41$\pm$0.45 
        &
        \\
        Herding 
        & 29.42$\pm$1.54 
        & 37.50$\pm$2.12 
        & 15.14$\pm$0.45 
        & 20.19$\pm$0.45 
        & 
        \\
        Forgetting 
        & 29.48$\pm$1.98 
        & 38.01$\pm$2.21 
        & 11.25$\pm$0.90 
        & 17.07$\pm$0.66 
        & 
        \\
        GraNd-score 
        & 23.03$\pm$1.05 
        & 34.83$\pm$2.01 
        & 13.68$\pm$0.46 
        & 19.51$\pm$0.45 
        & 
        \\
        EL2N-score 
        & 21.95$\pm$1.08 
        & 31.63$\pm$2.84 
        & 10.11$\pm$0.25 
        & 13.69$\pm$0.32 
        & 
        \\
        Optimization-based 
        & 26.77$\pm$0.15 
        & 35.63$\pm$0.92 
        & 12.37$\pm$0.68 
        & 18.52$\pm$0.90 
        & 
        \\
        Self-sup.-selection 
        & 23.12$\pm$1.47 
        & 34.85$\pm$0.68 
        & 11.23$\pm$0.32 
        & 17.76$\pm$0.69 
        &
        \\
        Moderate-DS 
        & 28.45$\pm$0.53 
        & 36.55$\pm$1.26 
        & 15.27$\pm$0.31 
        & 20.33$\pm$0.28 
        & 
        \\
        {\bf $\gm$ Matching}
        & {\bf 43.33$\pm$ 1.02}
        & {\bf 58.41$\pm$ 0.68}
        & {\bf 23.14$\pm$ 0.92} 
        & {\bf 27.76$\pm$ 0.40}
        & 
        \\
        \bottomrule
    \end{tabular}
    \caption{35\% Label Noise}
    \label{tab:label-noise-0.35}
\end{table*}

\input{NeuRips-2024/tables/tab-noisy-tiny}

\input{NeuRips-2024/tables/tab-attacks}

\input{NeuRips-2024/tables/tab-vgg-shuffle}

\clearpage
\subsection{Additional Details on Baselines}

Here, we detail the technical aspects of the baselines used in our experiments:
\begin{itemize}
    \item \textbf{Random}: This approach involves randomly selecting a subset of the full dataset.
    \item \textbf{Herding} \cite{welling2009herding}: This method selects data points that are closest to the class centers.
    \item \textbf{Forgetting} \cite{toneva2018empirical}: Data points that are easily forgotten during optimization are chosen.
    \item \textbf{GraNd-score} \cite{paul2021deep}: Data points with larger loss gradient norms are included.
    \item \textbf{EL2N-score} \cite{paul2021deep}: This focuses on data points with larger norms of the error vector, which is the difference between the predicted class probabilities and the one-hot label encoding.
    \item \textbf{Optimization-based} \cite{yang2022dataset}: This method uses the influence function \cite{koh2017understanding} to select data points that minimize the generalization gap under strict constraints.
    \item \textbf{Self-sup.-selection} \cite{sorscher2022beyond}: After self-supervised pre-training and clustering, data points are selected based on their distance to the nearest cluster centroid, with the number of clusters set to the number of classes to avoid tuning. Points with larger distances are chosen.
\end{itemize}

% \clearpage
% \subsection{Numerical Implementation of $\gm$}

% \begin{lstlisting}[language=Python]
% """
% Robust Estimation of Location Parameters
% """
% import numpy as np
% from scipy.spatial.distance import cdist, euclidean

% def robust_mean_estimate(
% 		data: np.ndarray,
% 		estimator: str = 'geo_med',
% 		eps: float = 1e-10,
% 		max_iter: int = 1000) -> np.ndarray:
% 	"""
%     Implements: "On the point for which the sum of the distances to 
%     n given points is minimum (1927)". E Weiszfeld, F Plastria; 
%     Annals of Operations Research.
    
%     Robust Estimation of Location Parameters
%     :param data: np.ndarray of shape (n_samples, n_features)
%     :param estimator: str, 'geo_med' for geometric median
%     :param eps: float, stopping criteria
%     :param max_iter: int, maximum number of iterations
	
%     returns np.ndarray of shape (n_features, 1)
%             robust estimate of location parameter (mean)
% 	"""
% 	if estimator == 'geo_med':
%     	# initial Guess : centroid / empirical mean
%     	mu = np.mean(a=data, axis=0)
%     	num_iter = 0
%     	while num_iter < max_iter:
%     		# noinspection PyTypeChecker
%     		distances = cdist(data, [mu]).astype(mu.dtype)
%     		distances = np.where(distances == 0, 1, distances)
%     		mu1 = (data / distances).sum(axis=0) / (1. / distances).sum(axis=0)
%     		guess_movement = np.sqrt(((mu - mu1) ** 2).sum())
%     		mu = mu1
%     		if guess_movement <= eps:
%     			return mu
%     		num_iter += 1
%     	print('Ran out of Max iter for GM - returning sub optimal')
%     	return mu
  
% 	else:
% 		raise NotImplementedError
% \end{lstlisting}
