# Supplementary material for: Geometric Median (GM) Matching for Robust Data Pruning
Source: arXiv:2406.17188 source file (2025-01-17)
Supplement: Supplementary file 2 [file notations.tex]

\subsection{Notations and Abbreviations}
\bgroup

\begin{tabular}{p{1in}p{3.25in}}
$\displaystyle a$ & A scalar (integer or real)\\
$\displaystyle \va$ & A vector\\
$\displaystyle \mA$ & A matrix\\
$\displaystyle \ra$ & A scalar random variable\\
$\displaystyle \rva$ & A vector-valued random variable\\
$\displaystyle \sA, \gA$ & A set\\
$\displaystyle [a, b]$ & The real interval including $a$ and $b$\\
$\displaystyle \sA \backslash \sB$ & Set subtraction, i.e., the set containing the elements of $\sA$ that are not in $\sB$\\
$\displaystyle \erva_i$ & Element $i$ of the random vector $\rva$ \\
$\displaystyle P(\ra)$ & A probability distribution over a discrete variable\\
$\displaystyle p(\ra)$ & A probability distribution over a continuous variable, or over
a variable whose type has not been specified\\
$\displaystyle f: \sA \rightarrow \sB$ & The function $f$ with domain $\sA$ and range $\sB$\\
$\displaystyle f \circ g $ & Composition of the functions $f$ and $g$ \\
  $\displaystyle f(\vx ; \vtheta) $ & A function of $\vx$ parametrized by $\vtheta$.
  (Sometimes we write $f(\vx)$ and omit the argument $\vtheta$ to lighten notation) \\
$\displaystyle || \vx ||_p $ & $\normlp$ norm of $\vx$ \\
$\displaystyle \1(condition)$ & is 1 if the condition is true, 0 otherwise\\
$\gmm$ & Geometric Median Matching 
\end{tabular}
\egroup
