# Supplementary material for: Geometric Median (GM) Matching for Robust Data Pruning
Source: arXiv:2406.17188 source file (2025-01-17)
Supplement: Supplementary file 4 [file appendix.tex]

\subsection{Notations and Abbreviations}
\bgroup

\begin{tabular}{p{1in}p{3.25in}}
$\displaystyle a$ & A scalar (integer or real)\\
$\displaystyle \va$ & A vector\\
$\displaystyle \mA$ & A matrix\\
$\displaystyle \ra$ & A scalar random variable\\
$\displaystyle \rva$ & A vector-valued random variable\\
$\displaystyle \sA, \gA$ & A set\\
$\displaystyle [a, b]$ & The real interval including $a$ and $b$\\
$\displaystyle \sA \backslash \sB$ & Set subtraction, i.e., the set containing the elements of $\sA$ that are not in $\sB$\\
$\displaystyle \erva_i$ & Element $i$ of the random vector $\rva$ \\
$\displaystyle P(\ra)$ & A probability distribution over a discrete variable\\
$\displaystyle p(\ra)$ & A probability distribution over a continuous variable, or over
a variable whose type has not been specified\\
$\displaystyle f: \sA \rightarrow \sB$ & The function $f$ with domain $\sA$ and range $\sB$\\
$\displaystyle f \circ g $ & Composition of the functions $f$ and $g$ \\
  $\displaystyle f(\vx ; \vtheta) $ & A function of $\vx$ parametrized by $\vtheta$.
  (Sometimes we write $f(\vx)$ and omit the argument $\vtheta$ to lighten notation) \\
$\displaystyle || \vx ||_p $ & $\normlp$ norm of $\vx$ \\
$\displaystyle \1(condition)$ & is 1 if the condition is true, 0 otherwise\\
$\gmm$ & Geometric Median Matching 
\end{tabular}
\egroup

% \clearpage
% \subsection{Additional Implementation Details}
% \label{sec:app-gm}
% Recall from~\cref{def:geo_med}, $\gm$ refers to the point that minimizes the 

% \begin{lstlisting}[language=Python]
% """
% Robust Estimation of Location Parameters
% """
% import numpy as np
% from scipy.spatial.distance import cdist, euclidean

% def robust_mean_estimate(
% 		data: np.ndarray,
% 		estimator: str = 'geo_med',
% 		eps: float = 1e-10,
% 		max_iter: int = 1000) -> np.ndarray:
% 	"""
%     Implements: "On the point for which the sum of the distances to 
%     n given points is minimum (1927)". E Weiszfeld, F Plastria; 
%     Annals of Operations Research.
    
%     Robust Estimation of Location Parameters
%     :param data: np.ndarray of shape (n_samples, n_features)
%     :param estimator: str, 'geo_med' for geometric median
%     :param eps: float, stopping criteria
%     :param max_iter: int, maximum number of iterations
	
%     returns np.ndarray of shape (n_features, 1)
%             robust estimate of location parameter (mean)
% 	"""
% 	if estimator == 'geo_med':
%     	# initial Guess : centroid / empirical mean
%     	mu = np.mean(a=data, axis=0)
%     	num_iter = 0
%     	while num_iter < max_iter:
%     		# noinspection PyTypeChecker
%     		distances = cdist(data, [mu]).astype(mu.dtype)
%     		distances = np.where(distances == 0, 1, distances)
%     		mu1 = (data / distances).sum(axis=0) / (1. / distances).sum(axis=0)
%     		guess_movement = np.sqrt(((mu - mu1) ** 2).sum())
%     		mu = mu1
%     		if guess_movement <= eps:
%     			return mu
%     		num_iter += 1
%     	print('Ran out of Max iter for GM - returning sub optimal')
%     	return mu
  
% 	else:
% 		raise NotImplementedError
% \end{lstlisting}

% \clearpage
% \subsection{Toy Experiments}
% \label{sec:app-toy}
% \input{plots/toy/fig.toy-corr=0}
% \input{plots/toy/fig.toy-corr=20}
% \input{plots/toy/fig.toy-corr=40}
% % \input{plots/toy/fig.toy-corr=45}

\clearpage
% \subsection{Complete Proofs}
% \label{sec:app-proofs}
% In this section we will describe the proof techniques involved in establishing the theoretical claims in the paper. 
\subsection{Proof of~\cref{lemma:score_dist_dev}}
\begin{proof}
    The original importance score without the corrupted sample is: 
    \begin{flalign}
        d(\vx_i, y_i) = \|\vx_i - \mu_y^\gG\|^2_2
    \end{flalign}
    
    The importance score with the corrupted sample affecting the centroid is:
    \begin{flalign}
        d'(\vx_i, y_i) = \| \vx_i - \mu_y^\gB\|^2_2
    \end{flalign}
    We can calculate the deviation as:
    \begin{flalign*}
        \Delta d(\vx_i, y_i) 
        &= d(\vx_i,y_i) - d'(\vx_i, y_i) \\
        &= \bigg(\vx_i - \mu_y^\gB \bigg)^T\bigg(\vx_i -\mu_y^\gB\bigg) - \bigg(\vx_i - \mu_y^\gG \bigg)^T\bigg(\vx_i -\mu_y^\gG\bigg)
    \end{flalign*}
    The result follows by expanding and defining $\Delta \mu_y = \mu_y^\gB - \mu_y^\gG$
\end{proof}

% \begin{theorem*}
%     Suppose that, we are given, a set of $\alpha$-corrupted samples $\gD$ (\cref{def:corruption_model}), pretrained proxy model $\phi_\mB$, and an $\epsilon$ approx. $\gm(\cdot)$ oracle~\eqref{eq:gm}, assume that $\phi_\mB(\vx) \leq R \; \forall \vx \in D$. Then, $\gm$ Matching guarantees that the mean of the selected $k$-subset converges to the neighborhood of $\bm{\mu}^\gG = \E_{\vx \in \sD_\sG}(\phi_\mB(\vx))$ at the rate $\gO(\frac{1}{k})$ as:   
%     \begin{equation}
%         \E\bigg\|\frac{1}{k} \sum_{\vx_i \in \gD_\gS}\vx_i - \bm{\mu}^\gG\bigg \|^2\leq 
%         \frac{8|\gD_\gG|}{(|\gD_\gG|-|\gD_\gB|)^2}\sum_{\vx \in \gD_\gG}\E\bigg\|\phi_\mB(\vx) -\bm{\mu}^\gG \bigg\|^2 +\frac{2\epsilon^2}{(|\gD_\gG|-|\gD_\gB|)^2}.
%      \end{equation}
% \end{theorem*}

\subsection{Intermediate Lemmas}
% We restate~\cref{lemma:gm_mean_bound}for convenience:

In order to prove~\cref{th:gm_match_cvg}, we will first establish the following result which follows from the definition of $\gm$; see also~\citep{lopuhaa1991breakdown,minsker2015geometric,cohen2016geometric,chen2017distributed,li2019rsa,wu2020federated, pmlr-v151-acharya22a} for similar adaptations.

\begin{lemma}
    Given a set of $\alpha$-corrupted samples $\gD = \gD_\gG \cup \gD_\gB$ (~\cref{def:corruption_model}), and an $\epsilon$-approx. $\gm(\cdot)$ oracle~\eqref{eq:gm}, then we have: 
    \begin{equation}
        \E\bigg\| \bm{\mu}^\gm - \bm{\mu}^\gG\bigg \|^2\leq 
        \frac{8|\gD_\gG|}{(|\gD_\gG|-|\gD_\gB|)^2}\sum_{\vx \in \gD_\gG}\E\bigg\|\vx -\bm{\mu}^\gG \bigg\|^2 +\frac{2\epsilon^2}{(|\gD_\gG|-|\gD_\gB|)^2}
        \label{eq:gm_mean_bound}
     \end{equation}
     where, $\bm{\mu}^\gm = \gm(\{\vx_i \in \gD\})$ is the $\epsilon$-approximate $\gm$ over the entire ($\alpha$-corrupted) dataset; and $\bm{\mu}^\gG = \frac{1}{|\gD_\gG|}\sum_{\vx_i \in \gD_\gG}\vx_i$ denotes the mean of the (underlying) uncorrupted set. 
\label{lemma:gm_mean_bound}
\end{lemma} 

\begin{proof}
Note that, by using triangle inequality, we can write:
\begin{flalign}
    \sum_{\vx_i \in \gD} \bigg\|\bm{\mu}^\gm - \vx_i\bigg\| 
    \nonumber
    & \geq \sum_{\vx_i \in \gD_\gB} \bigg( \bigg\|\vx_i\bigg\| - \bigg\|\bm{\mu}^\gm\bigg\|\bigg) +
    \sum_{\vx_i \in \gD_\gG} \bigg( \bigg\|\bm{\mu}^\gm\bigg\| - \bigg\|\vx_i\bigg\|\bigg)\\
    \nonumber
    & = \bigg( \sum_{\vx_i \in \gD_\gG} - \sum_{\vx_i \in \gD_\gB} \bigg) \bigg\|\bm{\mu}^\gm\bigg\| +
    \sum_{\vx_i \in \gD_\gB} \bigg\|\vx_i\bigg\| - \sum_{\vx_i \in \gD_\gG} \bigg\|\vx_i\bigg\|\\
    & = \bigg( |\gD_\gG| - |\gD_\gB|\bigg) \bigg\|\bm{\mu}^\gm\bigg\| +
    \sum_{\vx_i \in \gD} \bigg\|\vx_i\bigg\| - 2\sum_{\vx_i \in \gD_\gG} \bigg\|\vx_i\bigg\|.
\end{flalign}
    
Now, by definition~\eqref{eq:gm_epsilon}; we have that:
\begin{equation}
    \sum_{\vx_i \in \gD} \bigg\|\bm{\mu}^\gm - \vx_i\bigg\| 
    \leq \inf_{\vz \in \gH} \sum_{\vx_i \in \gD} \bigg\| \vz - \vx_i\bigg\| + \epsilon
    \leq \sum_{\vx_i \in \gD} \bigg\|\vx_i\bigg\| + \epsilon
\end{equation}

Combining these two inequalities, we get:
\begin{flalign}
    \bigg( |\gD_\gG| - |\gD_\gB|\bigg) \bigg\|\bm{\mu}^\gm\bigg\|
    \leq \sum_{\vx_i \in \gD} \bigg\|\vx_i\bigg\| - \sum_{\vx_i \in \gD} \bigg\|\vx_i\bigg\| + 2 \sum_{\vx_i \in \gD_\gG} \bigg\|\vx_i\bigg\| + \epsilon
\end{flalign}
This implies: 
\begin{flalign}
    \bigg\|\bm{\mu}^\gm\bigg\| \leq \frac{2 }{\bigg(|\gD_\gG| - |\gD_\gB|\bigg)}\sum_{\vx_i \in \gD_\gG} \bigg\|\vx_i\bigg\| + \frac{\epsilon}{\bigg( |\gD_\gG| - |\gD_\gB|\bigg)}
\end{flalign}
Squaring both sides, 
\begin{flalign}
    \bigg\|\bm{\mu}^\gm\bigg\|^2 
    &\leq \Bigg[\frac{2}{\bigg(|\gD_\gG| - |\gD_\gB|\bigg)}\sum_{\vx_i \in \gD_\gG} \bigg\|\vx_i\bigg\| + \frac{\epsilon}{\bigg( |\gD_\gG| - |\gD_\gB|\bigg)}\Bigg]^2\\
    &\leq 2\Bigg[\frac{2}{\bigg(|\gD_\gG| - |\gD_\gB|\bigg)}\sum_{\vx_i \in \gD_\gG} \bigg\|\vx_i\bigg\|\Bigg]^2 + 2 \Bigg[ \frac{\epsilon}{\bigg( |\gD_\gG| - |\gD_\gB|\bigg)}\Bigg]^2
\end{flalign}
Where, the last step is a well-known consequence of triangle inequality and AM-GM inequality. 
Taking expectation on  both sides, we have:
\begin{flalign}
    \E\bigg\|\bm{\mu}^\gm\bigg\|^2 
    &\leq \frac{8}{\bigg(|\gD_\gG| - |\gD_\gB|\bigg)^2}\sum_{\vx_i \in \gD_\gG} \E\bigg\|\vx_i\bigg\|^2 + \frac{2\epsilon^2}{\bigg( |\gD_\gG| - |\gD_\gB|\bigg)^2}
\end{flalign}
Since, $\gm$ is {\bf translation equivariant}, we can write:
\begin{flalign}
    \E\bigg[\gm\bigg(\bigg\{\vx_i - \bm{\mu}^\gG | \vx_i \in \gD\bigg\}\bigg)\bigg]
    = \E\bigg[\gm\bigg(\bigg\{\vx_i | \vx_i \in \gD \bigg\}\bigg) - \bm{\mu}^\gG \bigg]
\end{flalign}
Consequently we have that :
\begin{flalign}
    \nonumber
    \E\bigg\|\bm{\mu}^\gm - \bm{\mu}^\gG \bigg\|^2
    &\leq \frac{8}{\bigg(|\gD_\gG| - |\gD_\gB|\bigg)^2}\sum_{\vx_i \in \gD_\gG} \E\bigg\|\vx_i - \bm{\mu}^\gG \bigg\|^2 + \frac{2\epsilon^2}{\bigg( |\gD_\gG| - |\gD_\gB|\bigg)^2}
\end{flalign}
This concludes the proof.
\end{proof}

\subsection{Proof of Theorem~\ref{th:gm_match_cvg}}
We restate the theorem for convenience:

{\bf Theorem}~\ref{th:gm_match_cvg} 
Suppose that, we are given, a set of $\alpha$-corrupted samples $\gD$ (\cref{def:corruption_model}), and an $\epsilon$ approx. $\gm(\cdot)$ oracle~\eqref{eq:gm}. Then, $\gmm$ guarantees that the mean of the selected $k$-subset $\bm{\mu}^\gS = \frac{1}{k} \sum_{\vx_i \in \gD_\gS}\vx_i$ converges to the neighborhood of $\bm{\mu}^\gG = \E_{\vx \in \gD_\gG}(\vx)$ at the rate $\gO(\frac{1}{k})$ such that:   
\begin{equation}
    \E\bigg\|\bm{\mu}^\gS - \bm{\mu}^\gG\bigg \|^2\leq 
    \frac{8|\gD_\gG|}{(|\gD_\gG|-|\gD_\gB|)^2}\sum_{\vx \in \gD_\gG}\E\bigg\|\vx -\Mu^\gG \bigg\|^2 +\frac{2\epsilon^2}{(|\gD_\gG|-|\gD_\gB|)^2}
\end{equation}
        
\begin{proof}    

To prove this result, we first show that $\gmm$ converges to $\Mu_\epsilon^\gm$ at $\gO(\frac{1}{k})$. It suffices to show that the error $\delta = \bigg\| \Mu^\gm_\epsilon - \frac{1}{k} \sum_{\vx_i \in \gS}\vx_i\bigg\| \rightarrow 0$ asymptotically. We will follow the proof technique in~\citep{chen2010super} mutatis mutandis to prove this result. 
We also assume that $\gD$ contains the support of the resulting noisy distribution.

We start by defining a $\gm$-centered marginal polytope as the convex hull -- 
\begin{flalign}
    \gM_\epsilon := \text{conv}\bigg\{\vx -\Mu^\gm_\epsilon \;| \vx \in \gD\bigg\}
\end{flalign}

% and thus by invoking the {\bf translation equivariance} property of $\gm$ we get that it also resides in the relative interior of $\gM_\epsilon$.
Then, we can rewrite the update equation~\eqref{eq:theta_update} as: 
\begin{flalign}
    \vtheta_{t+1} 
    &= \vtheta_t + \Mu_\epsilon^\gm - \vx_{t+1}\\
    &= \vtheta_t - (\vx_{t+1} - \Mu_\epsilon^\gm)\\
    &= \vtheta_t - \bigg(\argmax_{\vx \in \gD} \langle \vtheta_t, \vx \rangle - \Mu_\epsilon^\gm\bigg)\\
    &= \vtheta_t - \argmax_{\vm \in \gM_\epsilon} \langle \vtheta_t, \vm \rangle\\
    &= \vtheta_t - \vm_t
\end{flalign}

Now, squaring both sides we get :

\begin{flalign}
    \|\vtheta_{t+1}\|^2 = \|\theta_t\|^2 + \|\vm_t\|^2 - 2 \langle \vtheta_t, \vm_t \rangle
\end{flalign}

rearranging the terms we get:
\begin{flalign}
    \|\vtheta_{t+1}\|^2 - \|\theta_t\|^2 
    &= \|\vm_t\|^2 - 2 \langle \vtheta_t, \vm_t \rangle \\
    &= \|\vm_t\|^2 - 2 \|\vm_t\|\|\vtheta_t\|\langle \frac{\vtheta_t}{\|\vtheta_t\|}, \frac{\vm_t}{\|\vm_t\|} \rangle\\
    &= 2\|\vm_t\|\bigg( \frac{1}{2}\|\vm_t\| - \|\vtheta_t\|\langle \frac{\vtheta_t}{\|\vtheta_t\|}, \frac{\vm_t}{\|\vm_t\|} \rangle \bigg)
\end{flalign}

Assume that $\|\vx_i\| \leq r \;  \forall \vx_i \in \gD$. , Then we note that, 
\begin{flalign*}
    \|\vx_i - \Mu_\epsilon^\gm\| 
    &\leq \|\vx_i\| + \|\Mu_\epsilon^\gm\| \leq 2r
\end{flalign*}
Plugging this in, we get:
\begin{flalign}
    \|\vtheta_{t+1}\|^2 - \|\theta_t\|^2 
    &\leq 2\|\vm_t\| \bigg( r - \|\vtheta_t\|\langle \frac{\vtheta_t}{\|\vtheta_t\|}, \frac{\vm_t}{\|\vm_t\|} \rangle \bigg)
\end{flalign}

Recall that, $\Mu_\epsilon^\gm$ is guaranteed to be in the relative interior of 
$\text{conv}\{\vx \;| \vx \in \gD\}$~\citep{lopuhaa1991breakdown, minsker2015geometric}. Consequently, $\exists \kappa$-ball around $\Mu_\epsilon^\gm$ contained inside $\gM$ and we have $\forall t > 0$
\begin{flalign}
    \langle \frac{\vtheta_t}{\|\vtheta_t\|}, \frac{\vm_t}{\|\vm_t\|} \rangle 
    &\geq \kappa > 0
\end{flalign}
This implies, $\forall t > 0$
\begin{flalign}
    \|\vtheta_t\| \leq \frac{r}{\kappa}
\end{flalign}

Expanding the value of $\vtheta_t$ we have:
\begin{flalign}
    \bigg\|\vtheta_k\bigg\| = \bigg\|\vtheta_0  + k \Mu^\gm_\epsilon - \sum_{i=1}^k \vx_k \bigg\| \leq \frac{r}{\kappa}
\end{flalign}
Apply Cauchy Schwartz inequality:
\begin{flalign}
    \bigg\|k \Mu^\gm_\epsilon - \sum_{i=1}^k \vx_k \bigg\|
    &\leq \bigg\|\vtheta_0\bigg\| + \frac{r}{\kappa} 
\end{flalign}
normalizing both sides by number of iterations $k$
\begin{flalign}
    \bigg\|\Mu^\gm_\epsilon - \frac{1}{k}\sum_{i=1}^k \vx_k \bigg\|
    &\leq \frac{1}{k}\bigg(\bigg\|\vtheta_0\bigg\| + \frac{r}{\kappa}\bigg) 
\end{flalign}
Thus, we have that $\gmm$ converges to $\Mu^\gm_\epsilon$ at the rate $\gO(\frac{1}{k})$. 

Combining this with~\cref{lemma:gm_mean_bound}, completes the proof. 
\end{proof}
